# Supplementary material for: MeGAS: Thermomechanical Dynamic Gaussian Splatting for Thermophysical Scene Editing
Source: arXiv:2606.23455 source file (2026-06-22)
Supplement: Supplementary file 1 [file X_supp.tex]

\clearpage
\setcounter{page}{1}

\title{%
    \makebox[\textwidth][c]{%
        \parbox{\dimexpr\textwidth+1.0em\relax}{\centering\sloppy
        % Supplementary Material for \\
        \method\hspace{-0.25em}\meltIcon[0.9em]:\ 
        Thermomechanical Dynamic Gaussian Splatting for Thermophysical Scene Editing
        \\ 
        - Supplementary Material -
        }
    }
    \vspace{-1.0 em}
}

\author{}
\institute{}

\titlerunning{MeGAS: Thermomechanical Dynamic Gaussian Splatting}
\authorrunning{Z. Yang et al.}

\maketitle

% \renewcommand{\thetable}{\thesection.\arabic{table}}
% \renewcommand{\thefigure}{\thesection.\arabic{figure}}

% This document provides (1) training details for the topology-adaptive GS, (2) full formulations and implementation details of the MPM–LBM simulator, (3) derivations and implementation of the implicit-surface-guided densification, (4) prompt and parameter settings for editing baselines, and (5) additional qualitative results.
This supplementary material provides detailed descriptions of the training procedure for topology-adaptive Gaussian Splatting (Sec. \ref{supp:train_3dgs}), the full formulations and implementation details of the MPM-LBM simulator (Sec. \ref{supp:mpm_lbm}), the derivation and implementation of the implicit-surface-guided densification module (Sec. \ref{supp:imls_densify}), the computational cost analysis of each stage (Sec.~\ref{supp:computation_cost}), the generalization behavior of topology-adaptive rendering (Sec. \ref{supp:general_topology_render}), the experimental setup for thermophysical scene editing including baseline prompts, parameter settings, and user-study details (Sec. \ref{supp:exp_edit}), and additional qualitative results on multi-material editing, multi-view consistency, and real-world scenes (Secs. \ref{supp:seg_material}-\ref{supp:more_real_data}).

\vspace{-0.5 em}
\section{Details for Training Topology-Adaptive GS}
\label{supp:train_3dgs}
\vspace{-0.25 em}
% 我们首先使用COLMAP对输入的图像序列以获取位姿和稀疏点云。除了得到逼真的渲染，我们还希望重建的3DGS模型能够有较好的几何，因此在原有3DGS的Pipeline基础上，我们加入了PGSR中的Plane约束，which包括约束|min(s1,s2,s3)|使gs接近于平面surfel，以及使用unbiased plane depth约束depth和normal的一致性。
% 在PGSR的基础上，我们使用了Sec.4.2.1 Internal-Free Uniform Gaussian Regularization来进一步抑制大形变时内部Floater的暴露和gs分布不均匀导致的needle-like floaters。We train 3DGS with the plane-aware regularization from PGSR以及我们的anisotropy loss for 30k iterations:
% L = L_rgb(I,I) + L_geo() + lambda_anisotropy * L_ani
% 我们在训练过程中每2500步开启一次Low-contribution Gaussian Pruning，the weight-pruning threshold tau_prune we used is 0.2，同时我们每1000步apply 一次scale clamping with tau_scale = 1/128. All experiments are conducted on a single NVIDIA RTX 4090 GPU.
% 我们在NeRF-Synthetic Dataset上测试了我们模块对PSNR的影响，在减少内部floater以及得到更均匀的GS分布同时，保持了一样的渲染质量。
We first run COLMAP~\cite{schonberger2016structure} with the input image sequence to estimate the camera poses and sparse point cloud for reconstruction. 
Building on the vanilla 3D Gaussian Splatting pipeline~\cite{kerbl3Dgaussians}, we incorporate the planar regularization from \cite{chen2024pgsr,huang20242d} to improve geometric fidelity.
Specifically, each Gaussian is encouraged to approximate a local plane by penalizing the smallest principal scale $||\min(s_1, s_2, s_3)||_{1}$, and we adopt the unbiased plane-depth regularization to enforce consistency between the rendered depth and the corresponding surface normals to further align with the underlying surface.
On top of the planar regularization, we apply our internal-free uniform Gaussian regularization, introduced in Sec.~\textcolor{red}{4.2.1} of the main paper, to enhance robustness under large deformations.
The topology-adaptive 3DGS is optimized for 30k iterations with a joint loss:
\begin{equation}
    \mathcal{L}
    = \mathcal{L}_{\mathrm{rgb}}
    + \mathcal{L}_{\mathrm{geo}}
    + \lambda_{\mathrm{aniso}} \mathcal{L}_{\mathrm{aniso}},
\end{equation}
where $\mathcal{L}_{\mathrm{rgb}}$ is the photometric loss from 3DGS~\cite{kerbl3Dgaussians}, $\mathcal{L}_{\mathrm{geo}}$ corresponds to the planar constraints from PGSR~\cite{chen2024pgsr}, and $\mathcal{L}_{\mathrm{aniso}}$ is our anisotropy loss.
The weight for anisotropy regularization $\lambda_{\mathrm{aniso}}$ is set to 0.1. 
During training, we perform low-contribution Gaussian pruning every 2{,}500 iterations with the pruning threshold of $\tau_{\text{prune}} $=$0.2$, and apply scale clamping every 1{,}000 iterations by truncating the principal scales with an upper bound $\tau_{\text{scale}}$=$1/128$.

Moreover, since we define each Gaussian normal as the direction of its shortest principal axis, the normal is ambiguous up to a sign in the absence of camera. To resolve this ambiguity, we introduce a learnable pseudo normal for each Gaussian and perform a short self-distillation stage after training. Each pseudo normal $\mathbf{n}'_i$ is randomly initialized and optimized using the rasterized Gaussian normal $\mathbf{n}_i$ as a pseudo label, with the loss:
\begin{equation}
\mathcal{L}_{\text{normal}} = \|\mathbf{N}' - 
\mathrm{stopgrad}(\mathbf{N})
\|_1,
\end{equation}
where $\mathbf{N}'$=$\sum_i T_i \alpha_i \mathbf{n}'_i$ and $\mathbf{N}$=$\sum_i T_i \alpha_i \mathbf{n}_i$. We finetune it for 500 iterations and 
% \clearpage\noindent
correct the orientation of Gaussian normals by enforcing alignment with the directions of the pseudo normals.

\begin{wraptable}{r}{0.475 \textwidth}
\vspace{-0.25 em}
\caption{
\textbf{Ablation of rendering quality.} 
We progressively add each module on top of the backbone. Our module substantially reduces internal floaters and yields a more uniform Gaussian distribution, while maintaining comparable PSNR.
Although the anisotropy regularization slightly degrades PSNR, the subsequent scale clamping recovers the rendering quality.
}
\vspace{1.0 em}
% \begin{table}[t]
\resizebox{\linewidth}{!}{
\begin{tabular}{lccc}
\specialrule{.1em}{.1em}{.1em}
Module (Progressively Add)    & PSNR$\uparrow$ & SSIM$\uparrow$ & LPIPS$\downarrow$ \\
\midrule
Backbone~\cite{chen2024pgsr}  & 37.33          & 0.9813          & 0.031             \\
\midrule
w/ Internal Pruning           & 36.76          & 0.9801          & 0.035             \\
w/ Anisotropy Reg.            & 35.81          & 0.9767          & 0.045             \\
w/ Scale Clamping             & 37.24          & 0.9805          & 0.031             \\
\specialrule{.1em}{.1em}{.1em}
\end{tabular}
}
\vspace{-2.0 em}

\label{supp:tab:psnr}
% \end{table}
\end{wraptable}

We additionally validate our internal-free uniform Gaussian regularization on the NeRF-Synthetic dataset~\cite{mildenhall2021nerf} in terms of rendering quality. 
As shown in Tab.~\ref{supp:tab:psnr}, the regularization substantially reduces internal floaters and yields a more uniform Gaussian distribution, while maintaining comparable PSNR to the vanilla PGSR~\cite{chen2024pgsr} baseline.

% 对于室外场景，我们会先使用PGSR对场景进行正常重建，然后分割出前景，Specifically，我们先使用GroundedSAM通过前景的prompt，i.e. "Truck","Lego Dozer"，获得多视图2D mask，然后使用对比学习实现前景的3D分割，之后对其使用internal-free uniform Gaussian regularization
For outdoor scenes, we first perform scene reconstruction with PGSR and then extract the foreground. Specifically, we employ GroundedSAM~\cite{ren2024grounded} with foreground prompts (e.g., “\textit{Truck}”, “\textit{Lego Dozer}”) to obtain multi-view 2D masks, and subsequently perform 3D foreground segmentation via contrastive learning~\cite{ying2024omniseg3d}. The resulting foreground Gaussians are then refined using our internal-free uniform Gaussian regularization.
All experiments are conducted on an NVIDIA RTX 4090 24GB GPU.

\begin{figure}[h] \centering
    \vspace{-2.0 em}
    \includegraphics[width=0.975 \textwidth]{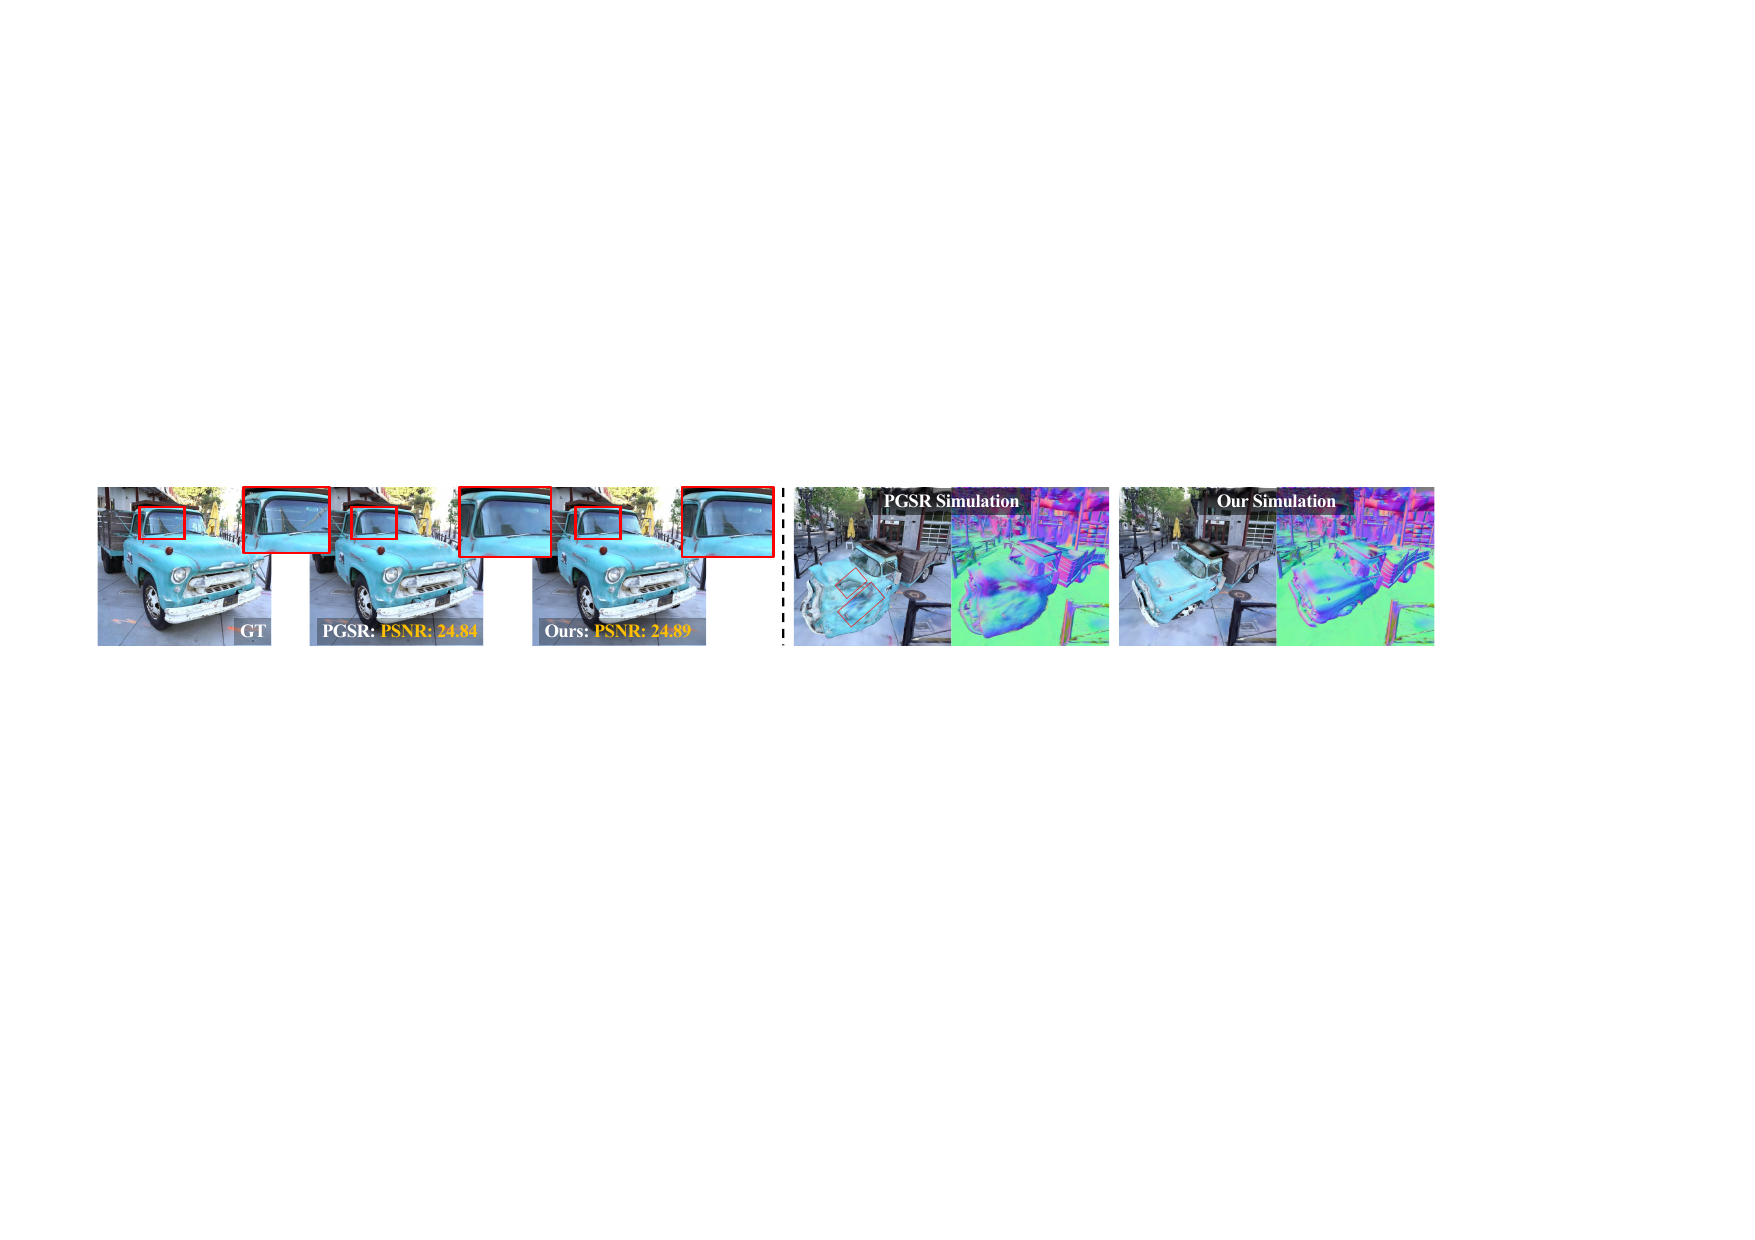}
    % \vspace{-3.5 em}
    \caption{
    We also add real-world finetuning comparisons, where our method adapts GS topology to melting-induced extreme deformations, while maintaining comparable rendering quality. 
    }
\end{figure}

\vspace{-0.5 em}
\section{Details for MPM-LBM Simulator}
\label{supp:mpm_lbm}
\vspace{-0.25 em}

% \begin{table}[h]
\begin{wraptable}{l}{0.55 \textwidth}
  \centering
  \vspace{-2.5 em}
  \caption{
  \textbf{Material and discretization parameters.}
  We use identical physical parameters across all experiments.
  }
  \vspace{1.0 em}
  \resizebox{\linewidth}{!}{
  \begin{tabular}{lcl}
    \hline
    Parameter & Value & Description \\
    \hline
    $E$ & $2.8\times10^{4}$ & Young's modulus \\
    $\nu$ & $0.4$ & Poisson's ratio \\
    $g$ & $1.0$ & Gravity acceleration \\
    $\rho$ & $100.0$ & Density of the solid \\
    $\eta$ & $100.0$ & Viscosity coefficient \\
    $h_{\text{shear}}$ & $1.0$ & Shear ratio for plastic flow \\
    $\sigma_{Y}$ & $1.0$ & Yield threshold \\
    $T_{\text{melt}}$ & $0.7$ & Thermal phase threshold \\
    \hline
    $\Delta t$ & $1.0\times 10^{-4}$ & Time step size \\
    $N_{\text{sub}}$ & $100$ & MPM sub-steps per frame \\
    $N_{\text{grid}}$ & $100^3$ & Grid resolution \\
    \hline
  \end{tabular}
  }
  
  \label{tab:mpm_params}
  \vspace{-2.0 em}
% \end{table}

\end{wraptable}

% 我们在此给出Thermal-Driven Material Point Method的完整过程，包括LBM的Heat advection-diffusion Update以及MPM的详细设置
We employ a hybrid particle-grid discretization for the MPM solver and the Lattice Boltzmann solver for the thermal advection-diffusion field. The MPM background grid and the LBM thermal lattice share the same Cartesian layout and spacing $\Delta$x, which allows all operations to be carried out on a common grid without any additional interpolation.

At the particle level (index $p$), we store the position $\mathbf{x}_p$, velocity $\mathbf{v}_p$, mass $m_p$, volume $V_p^0$, elastic deformation gradient $\mathbf{F}_p^{E}$, affine momentum matrix $\mathbf{C}_p$, temperature $T_p$ and its gradient $\nabla T_p$, and a phase flag indicating whether the material is solid or melted.
Grid / lattice nodes (index $i$) store  
mass $m_i$, velocity $\mathbf{v}_i$, and temperature $T_i$.  
For the LBM solver, each lattice node additionally stores the scalar distribution functions $g_{i,k}$ associated with discrete velocities $\mathbf{c}_k$ and weights $w_k$.
Cubic B-spline basis functions are used to define the particle-to-grid and grid-to-particle transfer weights $w_{ip}$ and their gradients $\nabla w_{ip}$.
A single time step from $t^n$ to $t^{n+1}=t^n+\Delta t$ consists of particle-to-grid transfer (P2G), grid update, and grid-to-particle transfer (G2P). The explicit algorithm is outlined as follows.

\noindent\textbf{Particle-to-Grid Transfer.}
We first reset all grid quantities to zero, then accumulate particle mass and momentum via APIC~\cite{jiang2015affine}:
\vspace{-0.5 em}
\begin{equation}
\vspace{-0.25 em}
\begin{aligned}
    m_i^{\,n} &= \sum_p w_{ip}^{\,n} m_p, \\
    \vspace{-1.0 em}
    m_i^{\,n} \mathbf{v}_i^{\,n}
    &= \sum_p w_{ip}^{\,n} m_p
    \left( \mathbf{v}_p^{\,n}
    + \mathbf{C}_p^{\,n} (\mathbf{x}_i - \mathbf{x}_p^{\,n}) \right).
\end{aligned}
\vspace{-0.25 em}
\end{equation}

\noindent For the thermal field we transfer a mass-weighted nodal temperature and its gradient:
\begin{equation}
    m_i^{\,n} T_i^{\,n}
    = \sum_p w_{ip}^{\,n} m_p \left( T_p^{\,n}
    + (\mathbf{x}_i - \mathbf{x}_p^{\,n})^\top \nabla T_p^{\,n} \right).
    \vspace{-0.5 em}
\end{equation}

After the accumulation, grid velocities and temperatures are normalised by mass for nodes with $m_i^{\,n} > 0$
\[
    T_i^{\,n} \leftarrow (m_i^{\,n} T_i^{\,n}) / m_i^{\,n},
    \;
    v_i^{\,n} \leftarrow (m_i^{\,n} v_i^{\,n}) / m_i^{\,n}.
\]

\noindent\textbf{Grid Update.}
Mechanical grid velocities are updated under internal and external forces:
\begin{equation}
    \mathbf{v}_i^{\,n+1}
    = \mathbf{v}_i^{\,n}
    - \frac{\Delta t}{m_i^{\,n}}
      \sum_p \boldsymbol{\tau}_p^{\,n} \nabla w_{ip}^{\,n} V_p^0
    + \Delta t\, \mathbf{g},
\end{equation}
where $\boldsymbol{\tau}_p^{\,n}$ is the Kirchhoff stress computed from the elastic deformation gradient
$\mathbf{F}_p^{E,n}$ and the current constitutive model (solid or melted), and $\mathbf{g}$ is the gravity ( or other external forces).

Thermal boundary conditions are applied to grid nodes associated with user-specified heat sources by constraining their temperatures to the prescribed source values, $T_i^{\,n} = T_{\text{source}}$.
In practice, $T_{\text{source}}$ is implemented as a Neumann-type heating condition, which incrementally increases the boundary temperature according to the imposed heat flux.

The grid temperatures at time $t^{n+1}$ are then updated by performing one step of the LBM solver, denoted by \texttt{LBM\_Update}.

\noindent\textbf{Thermal Advection-Diffusion Solver.}
The temperature field on the grid is advanced with a Lattice Boltzmann solver for the advection-diffusion equation (ADE):
\begin{equation}
\frac{\partial T}{\partial t}
+ \mathbf{u} \cdot \nabla T
= \alpha \nabla^2 T + S,
\end{equation}
where $\mathbf{u}$ is an advection velocity, $\alpha$ is the thermal diffusivity, and $S$ is a volumetric heat source.
In our pure diffusion experiments we simply set $\mathbf{u}=\mathbf{0}$, but the formulation also supports a fully
coupled Navier-Stokes LBM, in which case $\mathbf{u}$ is taken from the fluid velocity field described below.

We employ a standard single-relaxation-time (BGK) advection-diffusion LBM.
At each lattice node and direction $k$, the scalar populations $g_{i,k}$ evolve as:
\vspace{-0.75 em}
\begin{equation}
\label{eq:lbm_T_update}
% \begin{aligned}
g_{i,k}(\mathbf{x} + \mathbf{c}_k \Delta t,\; t + \Delta t)
= g_{i,k}(\mathbf{x}, t)
- \frac{\Delta t}{\tau_T} \left( g_{i,k} - g^{\text{eq}}_{i,k} \right) 
+ \Delta t\, Q_{i,k},
% \end{aligned}
\end{equation}
where $\tau_T$ is the thermal relaxation time.
The macroscopic temperature and discretized source term are recovered from the moments:
\begin{equation}
T_i = \sum_k g_{i,k}, 
\qquad
q_i = \sum_k Q_{i,k}.
\end{equation}

The equilibrium distribution is chosen analogously to the standard LB fluid equilibrium,
but with a single conserved scalar:
\begin{equation}
g^{\text{eq}}_{i,k} = w_k T_i 
\left[
1 
+ \frac{\mathbf{c}_k \cdot \mathbf{u}_i}{c_s^2}
+ \frac{(\mathbf{c}_k \cdot \mathbf{u}_i)^2}{2 c_s^4}
- \frac{\mathbf{u}_i \cdot \mathbf{u}_i}{2 c_s^2}
\right],
\end{equation}
where $c_s$ is the lattice sound speed and $\mathbf{u}_i$ is the prescribed advection velocity at node $i$
(for pure diffusion we set $\mathbf{u}_i = \mathbf{0}$).
The source term is discretized as:
\begin{equation}
Q_{i,k} = w_k\, q_i 
\left( 
1 - \frac{\Delta t}{2 \tau_T}
\right).
\end{equation}
A Chapman-Enskog expansion shows that this scheme recovers the ADE with thermal diffusivity:
\begin{equation}
\alpha = c_s^2 \left( \tau_T - \frac{\Delta t}{2} \right).
\end{equation}

If fluid motion is to be resolved, we augment the above temperature solver with an isothermal LBM for the (weakly compressible) Navier-Stokes equations:
\vspace{-1.0 em}
\begin{equation}
\partial_t (\rho \mathbf{u}) + \nabla \cdot (\rho \mathbf{u} \mathbf{u})
= -\nabla p + \nabla \cdot (2 \rho \nu \mathbf{D}) + \rho \mathbf{g} + \mathbf{F}_{\text{ext}},
\end{equation}
where $\rho$ is the density, $\nu$ is the kinematic viscosity, $\mathbf{D}$ is the rate-of-strain tensor, and $\mathbf{F}_{\text{ext}}$ collects body forces (e.g.\ buoyancy).

We introduce an additional set of distribution functions $f_{i,k}$ living on the same lattice with velocities $\mathbf{c}_k$ and weights $w_k$. Their evolution is given by:
\begin{equation}
\label{eq:lbm_f_update}
% \begin{aligned}
f_{i,k}(\mathbf{x} + \mathbf{c}_k \Delta t,\; t + \Delta t)=
f_{i,k}(\mathbf{x}, t)
- \frac{\Delta t}{\tau_f} \left( f_{i,k} - f^{\text{eq}}_{i,k} \right) 
+ \Delta t\, F_{i,k},
%\end{aligned}
\end{equation}
where $\tau_f$ is the fluid relaxation time and $F_{i,k}$ is a forcing term.
The macroscopic density and velocity are recovered as:
\begin{equation}
\rho_i = \sum_k f_{i,k}, 
\qquad
\rho_i \mathbf{u}_i = \sum_k \mathbf{c}_k f_{i,k}
+ \frac{\Delta t}{2}\, \mathbf{F}_i,
\end{equation}
with $\mathbf{F}_i$ the total body force at node $i$.
The equilibrium distribution is the standard second-order isothermal form:
\begin{equation}
f^{\text{eq}}_{i,k} = w_k \rho_i 
\left[
1 
+ \frac{\mathbf{c}_k \cdot \mathbf{u}_i}{c_s^2}
+ \frac{(\mathbf{c}_k \cdot \mathbf{u}_i)^2}{2 c_s^4}
- \frac{\mathbf{u}_i \cdot \mathbf{u}_i}{2 c_s^2}
\right].
\end{equation}
Under this choice, a Chapman-Enskog analysis shows that the LB scheme recovers the Navier-Stokes equations in the low-Mach-number limit, with kinematic viscosity:
\begin{equation}
\nu = c_s^2 \left( \tau_f - \frac{\Delta t}{2} \right).
\end{equation}

\noindent Body forces are incorporated via a standard Guo-type forcing term:
\begin{equation}
F_{i,k} = w_k
\left[
\frac{\mathbf{c}_k - \mathbf{u}_i}{c_s^2}
+ \frac{(\mathbf{c}_k \cdot \mathbf{u}_i)}{c_s^4}\,\mathbf{c}_k
\right]\!\cdot\! \mathbf{F}_i.
\end{equation}

For thermally driven flows, we use a Boussinesq approximation and define:
\begin{equation}
\mathbf{F}_i
= \rho_0 \beta \left( T_i - T_{\text{ref}} \right) \mathbf{g}
+ \mathbf{F}_{\text{other}},
\end{equation}
where $\rho_0$ is a reference density, $\beta$ is the thermal expansion coefficient, $T_{\text{ref}}$ is a reference temperature, and $\mathbf{F}_{\text{other}}$ collects any additional body forces.
The buoyancy term couples the temperature LBM and the Navier-Stokes LBM: the temperature field $T_i$ feeds into the body force $\mathbf{F}_i$, while the fluid velocity $\mathbf{u}_i$ is used as the advection velocity in the thermal equilibrium $g^{\text{eq}}_{i,k}$ in Eq.~\eqref{eq:lbm_T_update}.
In the special case where fluid motion is neglected, we simply disable the Navier-Stokes solver and set $\mathbf{u}_i=\mathbf{0}$ everywhere, resulting in a purely diffusive temperature evolution.

\noindent\textbf{Grid-to-Particle Transfer and Constitutive Update.}
After the grid velocities and temperatures have been advanced, we interpolate them back to particles:
\vspace{-0.25 em}
\begin{equation}
\mathbf{v}_p^{n+1} = \sum_i w_{ip}^n\, \mathbf{v}_i^{n+1},
\vspace{-0.25 em}
\end{equation}
\vspace{-0.25 em}
\begin{equation}
\nabla \mathbf{v}_p^{n+1} = \sum_i \mathbf{v}_i^{n+1} 
(\nabla w_{ip}^n)^{\!\top}
\vspace{-0.25 em}
\end{equation}

\vspace{-0.75 em}
\begin{equation}
\mathbf{x}_p^{n+1} = \mathbf{x}_p^{n} + \Delta t\, \mathbf{v}_p^{n+1},
\vspace{-0.5 em}
\end{equation}
\vspace{-0.25 em}
\begin{equation}
\mathbf{C}_p^{n+1} 
= \frac{4}{\Delta x^2} \sum_i w_{ip}^n\, \mathbf{v}_i^{n+1} 
(\mathbf{x}_i - \mathbf{x}_p^{n})^{\!\top},
\vspace{-0.25 em}
\end{equation}
\vspace{-0.25 em}
\begin{equation}
T_p^{n+1} = \sum_i w_{ip}^n\, T_i^{n+1},
\vspace{-0.25 em}
\end{equation}
\vspace{-0.25 em}
\begin{equation}
\nabla T_p^{n+1} = \sum_i T_i^{n+1} \left(\nabla w_{ip}^n\right)^{\!\top}.
\vspace{-0.25 em}
\end{equation}

\noindent The elastic deformation gradient is updated as:
\begin{equation}
\mathbf{F}_{p}^{E,n+1}
= \left(\mathbf{I} + \Delta t\, \nabla \mathbf{v}_p^{n+1}\right)
\mathbf{F}_p^{E,n}.
\end{equation}

Finally, we perform \textbf{temperature-driven phase switching}: 
if the particle temperature exceeds the melting threshold $\tau_{\text{melt}}$, we switch its constitutive model from solid to melted state, 
i.e.\ from StVK elasticity~\cite{klar2016drucker} to a Herschel-Bulkley viscoplastic model~\cite{yue2015continuum}; 
otherwise we keep the solid model:
\begin{equation}
(\tau_p^{n+1},\, \mathbf{F}_{p}^{E,n+1}) 
=
\begin{cases}
\text{solidModel}\!\left(\mathbf{F}_{p}^{E,n+1}\right),
\;\;\; T_p^{n+1} \le T_{\text{melt}}, \\[5pt]
\text{meltedModel}\!\left(\mathbf{F}_{p}^{E,n+1}\right),
T_p^{n+1} > T_{\text{melt}}.
\end{cases}
\end{equation}

For the StVK elasticity model, we define the Kirchhoff stress $\tau$ as:
\begin{equation}
\boldsymbol{\tau}
= \mathbf{U}\bigl( 2\mu\boldsymbol{\epsilon}
+ \lambda\mathrm{tr}(\boldsymbol{\epsilon})\mathbf{I} \bigr)\mathbf{V}^T ,
\end{equation}
where 
$\mathbf{F}^E = \mathbf{U}\, \boldsymbol{\Sigma}\, \mathbf{V}^{\!\top}$ is the SVD decomposition of $\mathbf{F}$ 
and 
$\boldsymbol{\epsilon} = \log(\boldsymbol{\Sigma})$ denotes the Hencky strain. Here $\mu$ and $\lambda$ are the Lamé parameters.

\iffalse
\begin{figure}[t] % 使用 !t 尝试强制图像置顶
    \centering
    \scriptsize
    \includegraphics[width=\linewidth]{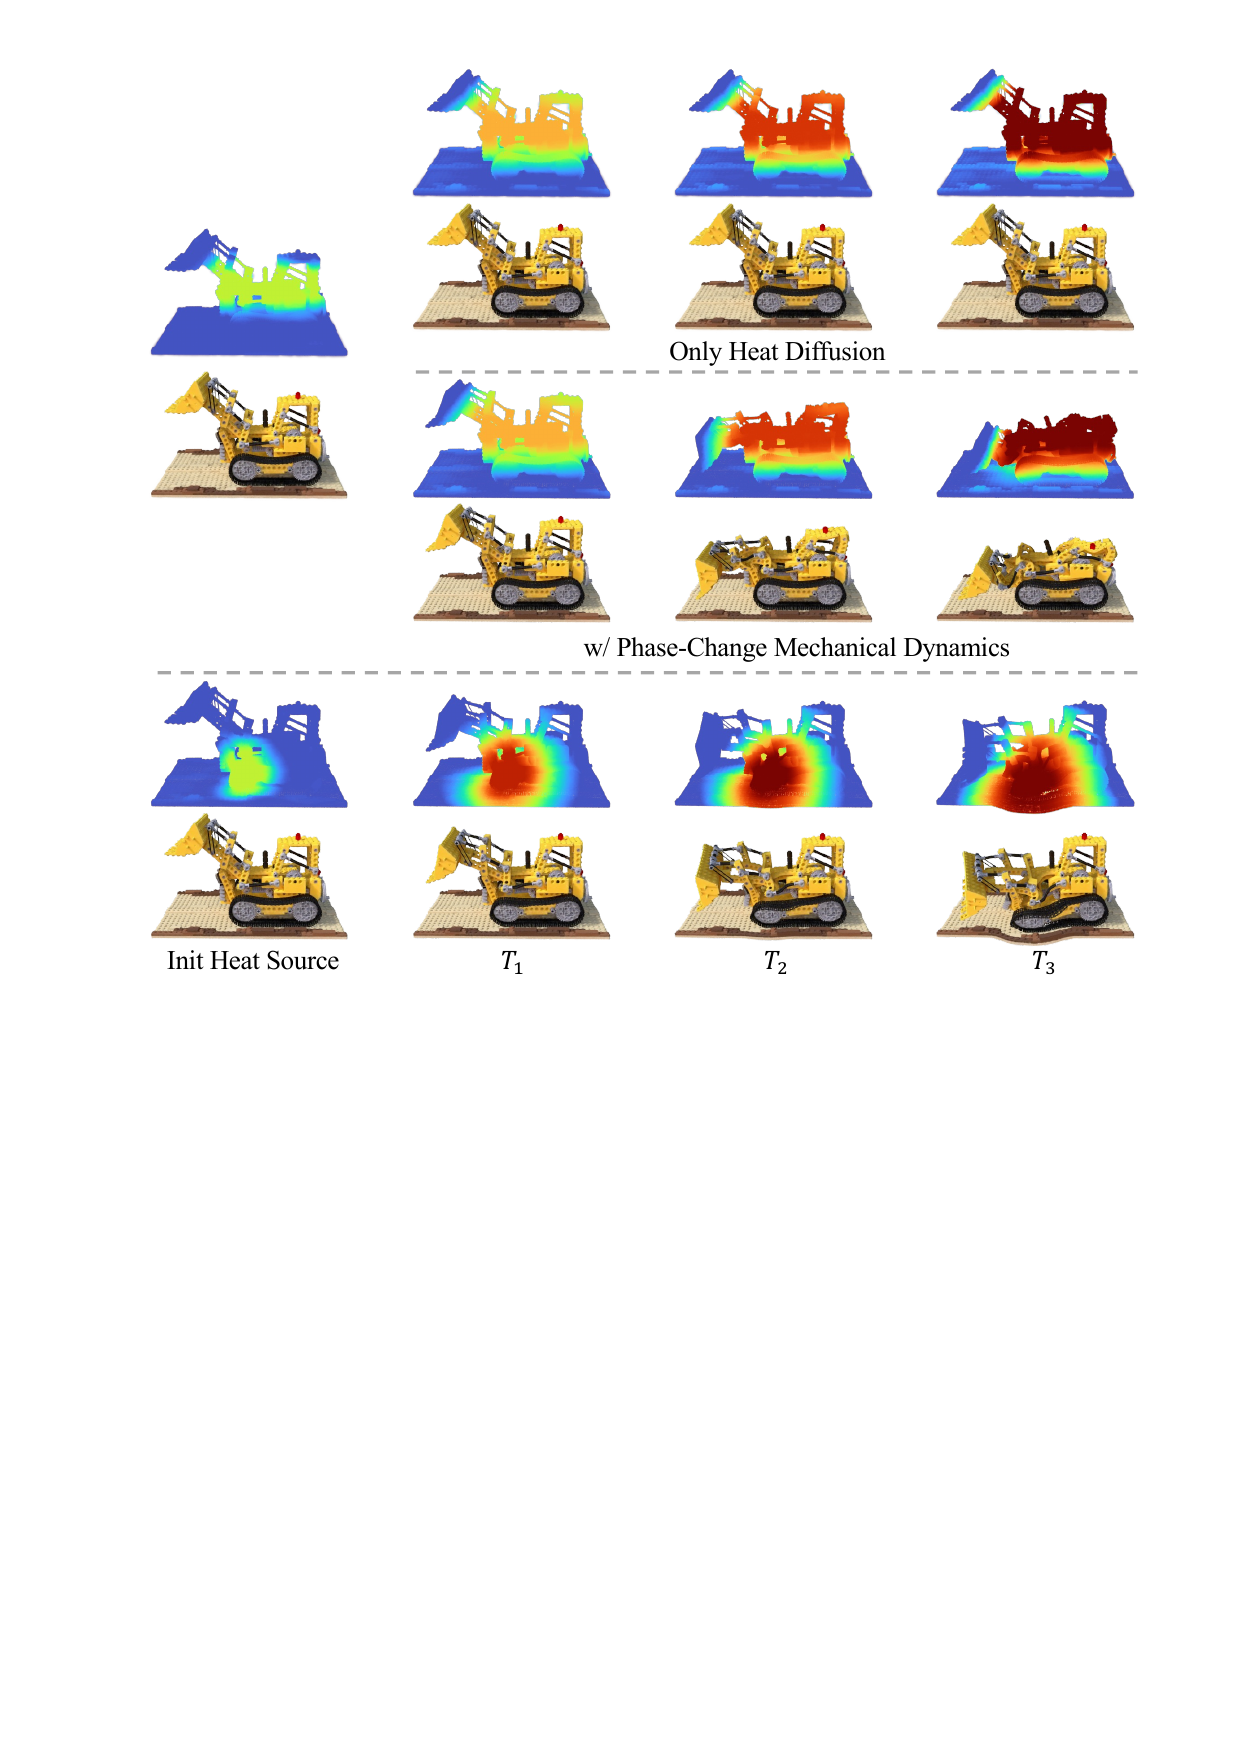}
    \vspace{-2.0 em}
    \caption{
    \textbf{Heat diffusion with constitutive modeling switching.}
    We first present visualizations of pure heat diffusion, where the temperature field gradually propagates from high to low values over time.
    By incorporating phase-change-controlled constitutive model switching, we present melting behavior that is explicitly driven by the evolving temperature field.
    Moreover, we show that different configurations of heat sources give rise to distinct melting patterns and effects.
    }
    \label{fig:supp:diffusion_process}
    \vspace{-2.0 em}
\end{figure}
\fi

For the Herschel-Bulkley viscoplastic model, we first compute the deviatoric part of the trial Kirchhoff stress:
\begin{equation}
\mathbf{s}_{n+1}^{\mathrm{pre}}
= \mu\, \mathrm{dev}\!\left[\tau_{n+1}\right],
\qquad
s_{n+1}^{\mathrm{pre}}
= \left\| \mathbf{s}_{n+1}^{\mathrm{pre}} \right\|_{F},
\end{equation}
where $\mathrm{dev}(\cdot)$ denotes the deviatoric part and 
$\|\cdot\|_{F}$ the Frobenius norm. 
If the von Mises equivalent stress satisfies:
\begin{equation}
s_{n+1}^{\mathrm{pre}}
- \sqrt{\frac{2}{3}}\, \sigma_Y \le 0,
% \vspace{-1.0 em}
\end{equation}
with $\sigma_Y$ the yield stress, the response remains elastic and the trial state is accepted.
Otherwise, plastic flow is activated and we perform a semi-implicit return-mapping step.
Define $\tilde{\mu}=\frac{\mu}{3}\;\mathrm{Tr}(\Sigma^2)$, we update the $s_{n+1}$ explicitly as:
\begin{equation}
\eta^{1/h}\left(s_{n+1} - s_{n+1}^{\mathrm{pre}}\right)
+ 2\tilde{\mu}\,\Delta t
\left(
s_{n+1} - \sqrt{\frac{2}{3}}\, \sigma_Y
\right)^{1/h}
= 0,
\end{equation}
where $\eta$ is the viscosity parameter and $h$ is the shear rate. We obtain $s_{n+1}$ via bisection.
The deviatoric stress is then projected back onto the yield surface as:
\begin{equation}
\hat{\mathbf{s}}_{n+1}
= 
\frac{s_{n+1}}{s_{n+1}^{\,\mathrm{pre}}}\,
\mathbf{s}_{n+1}^{\,\mathrm{pre}} ,
\end{equation}
and we update the Kirchhoff stress with $\hat{\mathbf{s}}_{n+1}$ as:
\begin{equation}
\boldsymbol{\tau} = \mathbf{U}\,
\exp\!\left(
\frac{\hat{s}}{2\mu}\, \mathrm{dev}\!\left[\boldsymbol{\epsilon}\right]
+ \frac{1}{3}\, \mathrm{Tr}(\boldsymbol{\epsilon})\, \mathbf{I}
\right)
\mathbf{V}^{T}.
\end{equation}

% As shown in Fig.~\ref{fig:supp:diffusion_process}, we illustrate the process of heat diffusion alone, as well as the constitutive model switching governed by phase-change control.
\input{sections/supp/2_raytracing}
\vspace{-1.0 em}
\section{Details for Densification with Implicit Surface Guidance}
\label{supp:imls_densify}
\vspace{-0.5 em}
We provide the full formulation and implementation details for the implicit-surface-guided adaptive densification (Sec.~\textcolor{red}{4.2.2}).

Define $\mathcal{G}_s = \left\{
G_i^{s} = 
\left( 
\mathbf{x}_i^{s},\,
\mathbf{R}_i^{s},\,
\mathbf{S}_i^{s},\,
\mathbf{o}_i^{s},\,
\mathbf{c}_i^{s}
\right)
\right\}
$ the Gaussians that lie on the reconstructed object surface in the rest state, and $\Phi_{t}(\cdot)$ is the deformation mapping at time step $t$ obtained from the MPM simulation.
After deformation, we obtain the deformed surface Gaussians:
\begin{equation}
\tilde{\mathcal{G}}_s^{\,t}
=
\Phi_{t}(\mathcal{G}_s)
=
\left\{
\tilde{G}_i^{s}
=
\left(
\tilde{\mathbf{x}}_i^{s},\,
\tilde{\mathbf{R}}_i^{s},\,
\tilde{\mathbf{S}}_i^{s},\,
\tilde{\mathbf{o}}_i^{s},\,
\tilde{\mathbf{c}}_i^{s}
\right)
\right\},
\end{equation}
and associate to each $\tilde{G}_i^{s}$ a surface normal $\tilde{\mathbf{n}}_i^{\,s}$
given by the shortest axis of $\tilde{\mathbf{S}}_i^{s}$.

% 此时我们有一组surfel-like的表面gaussian，以及内部填充的particle，我们希望用表面gaussian引导内部填充的particle去填补由于extreme deformation导致的表面开裂。我们希望填补的是原始表面gaussian存在空隙的区域，用于填补的对象是刚好填充这些空隙区域的internal particle，因此我们首要的第一步是通过surface detection来筛选出哪些internal particle可以被用来填充表面。我们在物体360度周围按照elevation 25度interval，azimuths 45度interval设置虚拟相机，并将internal particles初始化为isotropic Gaussian Splats with opacity=1。我们遍历virtual cameras，并记录光栅化过程中各个像素对应的gaussian splat with maximal alpha contribution along the ray, 从而筛选出用于填充表面的internal particles. 如图Fig.x所示，我们的方法在形变过程中有效的筛选出了正确的surface particles.

\begin{wrapfigure}[13]{r}{0.5\textwidth}
%\begin{figure}[t] % 使用 !t 尝试强制图像置顶
    \vspace{-1.75 em}
    \centering
    \scriptsize
    \includegraphics[width=\linewidth]{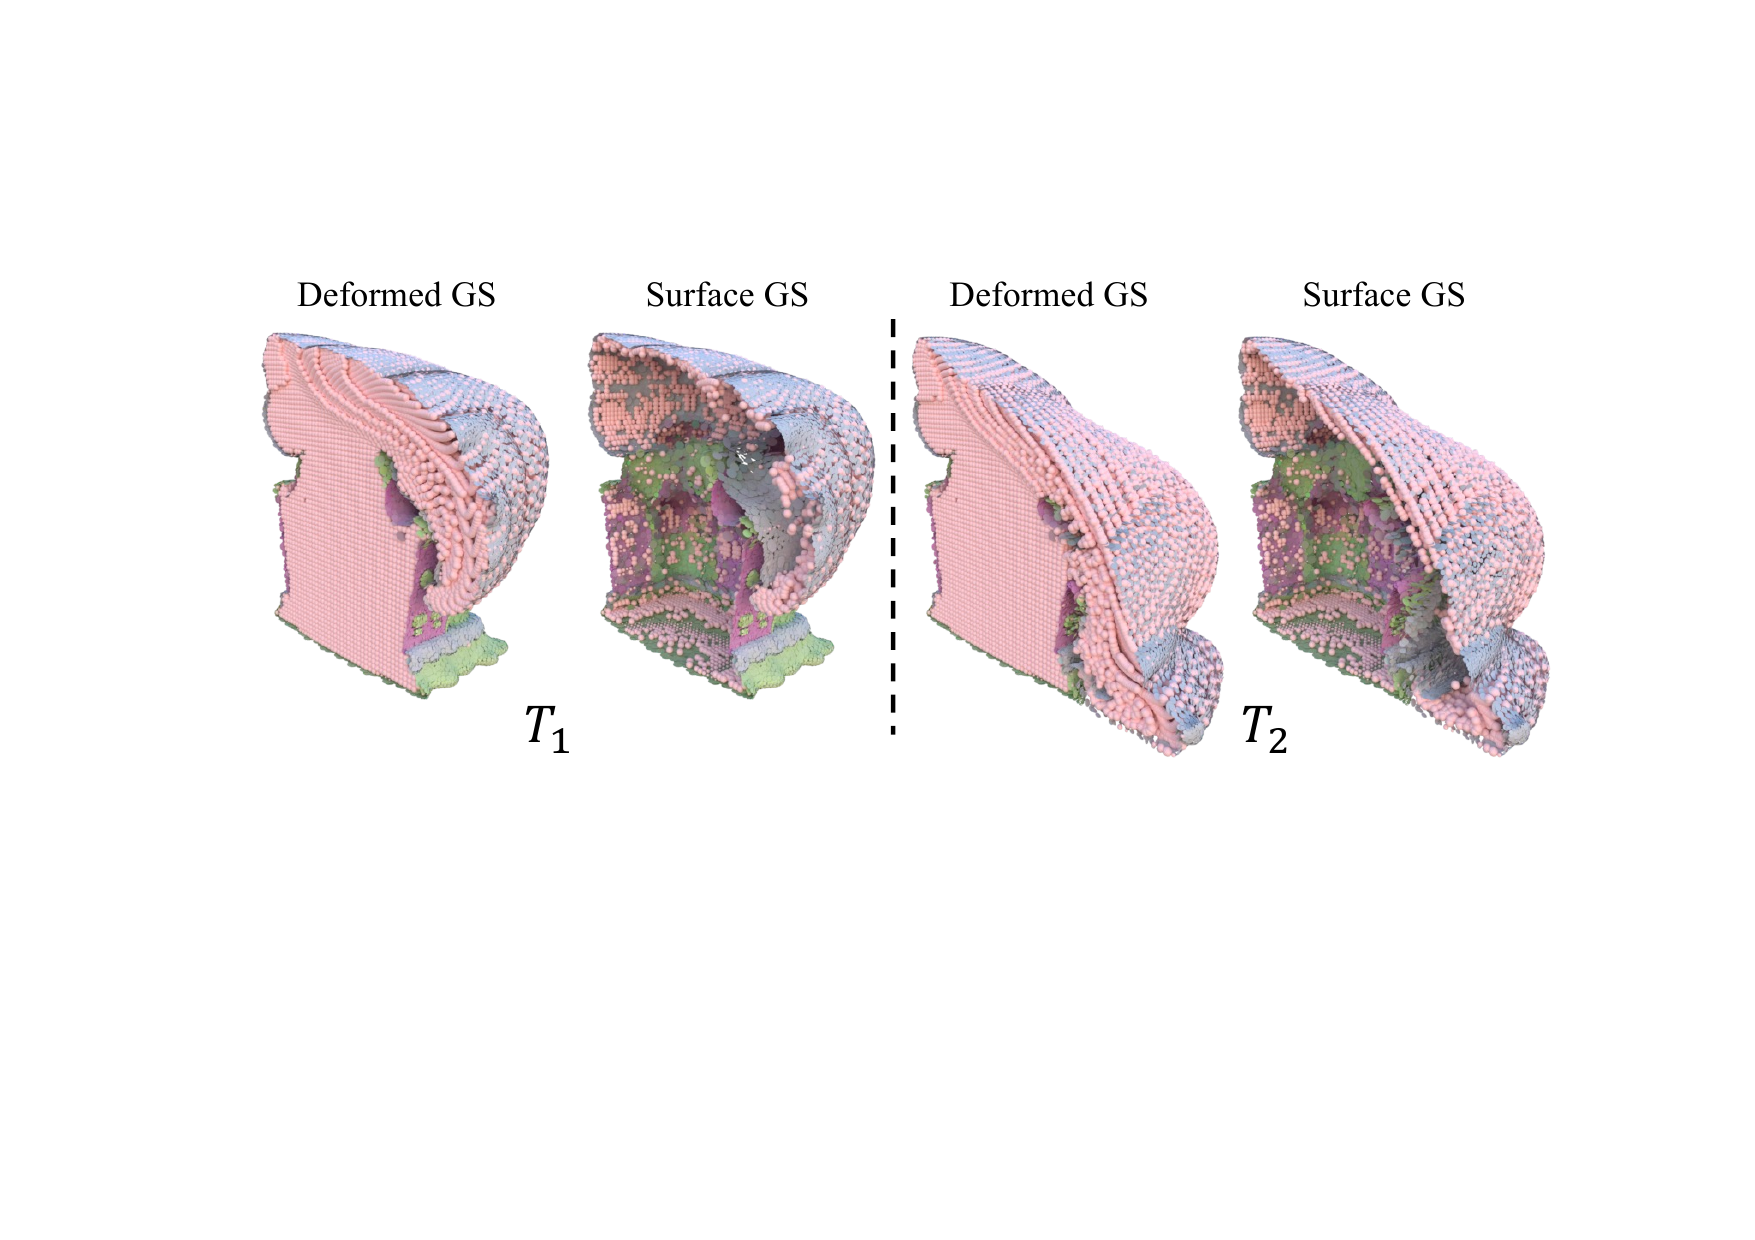}
    \vspace{-1.0 em}
    \caption{
    \textbf{Surface detection.}
    Our surface detection effectively filters the subset of internal particles, which are treated as candidates to be converted into new surface Gaussians for crack sealing.
    The internal particles are highlighted in pink for visualization. 
    }
    \label{fig:supp:surface_detection}
    \vspace{-2.0 em}
% \end{figure}
\end{wrapfigure}

\noindent\textbf{Surface Detection.}
At each rendering step, we maintain two sets of primitives: 
(i) a set of surfel-like surface Gaussians $\tilde{\mathcal{G}}_s^{\,t}$, and
(ii) a set of volumetric internal particles produced by the ray-tracing-based filling scheme.
Under extreme deformations, the surface Gaussians separate and expose cracks in the reconstructed surface, thus our goal is to reuse internal particles that lie close to the visible boundary to fill these newly exposed gaps.
% fill exactly these gaps. 
To this end, we first perform a surface detection that identifies which internal particles can be regarded as surface samples and are thus eligible for subsequent densification.

We distribute a set of virtual cameras on an object-centric viewing sphere to estimate visibility under deformation.
We sample camera azimuths every $45^{\circ}$ and elevations every $25^{\circ}$, covering the full $360^{\circ}$ around the object.
Internal particles $\mathbf{p}_j^t$ are initialized as isotropic Gaussian splats $G_j^p$ with opacity $\mathbf{o}_j=1$ and radius $r_j$:
\begin{equation}
r_j=\kappa\,\min\!\left\{\,\min_i\|\mathbf{p}_j^t-\mathbf{x}_i^s\|,\;\min_{k\neq j}\|\mathbf{p}_j^t-\mathbf{p}_k^t\|\,\right\},
\end{equation}
where $\kappa\in(0,1)$ is a shrinkage ratio, we set $\kappa=0.5$. 

We traverse the virtual cameras, rasterize the Gaussian splats $\{G_p,\; G_s\}$, and record the splat $G_i$ with maximal alpha contribution along the ray for each pixel.
The union of these front-most splats over all views yields the set of visible internal particles, which we treat as candidates to be converted into new surface Gaussians for crack sealing.
As shown in Fig.~\ref{fig:supp:surface_detection}, our surface detection strategy reliably tracks the evolving surface throughout large deformations.

\noindent\textbf{Implicit Surface from Deformed Gaussians.}
Given the deformed surface Gaussians $\tilde{\mathcal{G}}_s^{\,t}$, we follow the implicit moving least squares (IMLS) formulation for point set surfaces~\cite{alexa2001point,kolluri2008provably,oztireli2009feature} and define an implicit function:
\begin{equation}
f(\mathbf{x})
=
\frac{
\sum_i G_i^s (\mathbf{x})\,
(\tilde{\mathbf{n}}_{i}^{s})^{\!\top}
(\mathbf{x}-\tilde{\mathbf{x}}_{i}^{s})
}{
\sum_i G_i^s (\mathbf{x})
}.
\end{equation}
The zero level set $\mathcal{S}_{\text{IMLS}}=\{\mathbf{x} \mid f(\mathbf{x}) = 0\}$ 
defines an approximation of the deformed surface.
For the spatial weighting kernel, we directly reuse the Gaussian kernel associated with each splat $G_i^s$:
\begin{equation}
G_i^s(\mathbf{x})
=
\begin{cases}
\displaystyle
e^{\!-\frac{1}{2}(\mathbf{x}-\mathbf{x}_i^s)^{\top}\boldsymbol{\Sigma}^{-1}(\mathbf{x}-\mathbf{x}_i^s)}, & \|\mathbf{x}-\mathbf{x}_i^s\|_2 < h, \\[6pt]
0, & \|\mathbf{x}-\mathbf{x}_i^s\|_2 \ge h,
\end{cases}
\end{equation}
where $\boldsymbol{\Sigma}$ denotes the covariance of the Gaussian and $h$ is an adaptive influence radius.
For a query point $\mathbf{x}$, we estimate $h$ from the local density of Gaussians as
$h(\mathbf{x}) = \eta\, \bar{d}(\mathbf{x})$, 
where $\bar{d}(\mathbf{x})$ is the average distance to the $k$ nearest surface
Gaussians in $\tilde{\mathcal{G}}_{s}^{\,t}$ (we use $k=32$) and 
$\eta$ is a constant scaling factor (we use $\eta=1.5$).

We then project each candidate internal particle $\mathbf{p}_j^{\,t}$, detected by the surface selection stage described above, onto the implicit surface $\mathcal{S}_{\text{IMLS}}$.
Let $\mathbf{x}_j^{(0)} = \mathbf{p}_j^{\,t}$ be the initialization.
We perform a small, fixed number $L$ of Newton-style iterations:

\begin{enumerate}
\vspace{-1.0 em}
\item Evaluate $f(\mathbf{x}_j^{(\ell)})$.

\item Approximate the gradient of $f$ at $\mathbf{x}_j^{(\ell)}$ by a locally weighted average of normals:
\begin{equation}
\nabla f(\mathbf{x}_j^{(\ell)})
    \approx
    \frac{
        \sum_{i} G_i^s(\mathbf{x}_j^{(\ell)})\, \tilde{\mathbf{n}}_i^{\,s}
    }{
        \sum_{i} G_i^s(\mathbf{x}_j^{(\ell)})
    }.
\end{equation}

\item Normalize the gradient to obtain the local surface normal:
\begin{equation}
\mathbf{n}_j^{(\ell)}
=
\frac{
    \nabla f(\mathbf{x}_j^{(\ell)})
}{
    \bigl\lVert \nabla f(\mathbf{x}_j^{(\ell)}) \bigr\rVert
}.
\end{equation}

\item Update the position along the normal direction:
\begin{equation}
\mathbf{x}_j^{(\ell+1)}
=
\mathbf{x}_j^{(\ell)}
-
\, f(\mathbf{x}_j^{(\ell)})\, \mathbf{n}_j^{(\ell)}.
\end{equation}
\end{enumerate}

We terminate the iterations if $\lvert f(\mathbf{x}_j^{(\ell)}) \rvert < \varepsilon$
(we use $\varepsilon = 10^{-5}$)
or when $\ell$ reaches $L_{\max}$ (we use $L_{\max} = 5$).
The final projected position and normal are denoted by $\mathbf{x}_j^{\star}$ and $\mathbf{n}_j$, respectively.

\noindent\textbf{Gaussian Kernel Refitting.}
Given $(\mathbf{x}_j^{\star}, \mathbf{n}_j, r_j)$, we assign a new Gaussian kernel
$G_j^{p}$ to the crack-filling particle:
\begin{itemize}
  % \vspace{-2.0 em}
  \item \textbf{Position.}
  The Gaussian center is set to the projected position,
  $\boldsymbol{\mu}_j = \mathbf{x}_j^{\star}$.

  \item \textbf{Orientation.}
  We construct a rotation matrix $\mathbf{R}_j$ whose normal axis is aligned with the surface normal $\mathbf{n}_j$.
  
  \item \textbf{Scale.}
  We construct the scale matrix to represent an isotropic disk in the tangent plane, i.e.,
  $\mathbf{S}_j = \mathrm{diag}(r_j,\,r_j,\,0)$.

  \item \textbf{Appearance.}
  The appearance parameter $\mathbf{c}_j$ is computed as the average of
  the $K$ nearest surface Gaussians in $\tilde{\mathcal{G}}_{s}^{\,t}$:
  \begin{equation}
  \vspace{-0.5 em}
  \mathbf{c}_j
  = \frac{1}{K}
    \sum_{i \in \mathcal{N}_K(\mathbf{x}_j^{\star})}
    \tilde{\mathbf{c}}_i^{\,s},
  \end{equation}
  where $\mathcal{N}_K(\mathbf{x}_j^{\star})$ denotes the indices of the $K$
  nearest neighbors in position space.

  \item \textbf{Opacity.}
  We initialize the opacity $o_j = 1$.
  % \vspace{-1.0 em}
\end{itemize}

\begin{wrapfigure}[18]{r}{0.5 \textwidth}
% \begin{figure}[!t] % 使用 !t 尝试强制图像置顶
    \vspace{-3.0 em}
    \centering
    \scriptsize
    \includegraphics[width=0.9\linewidth]{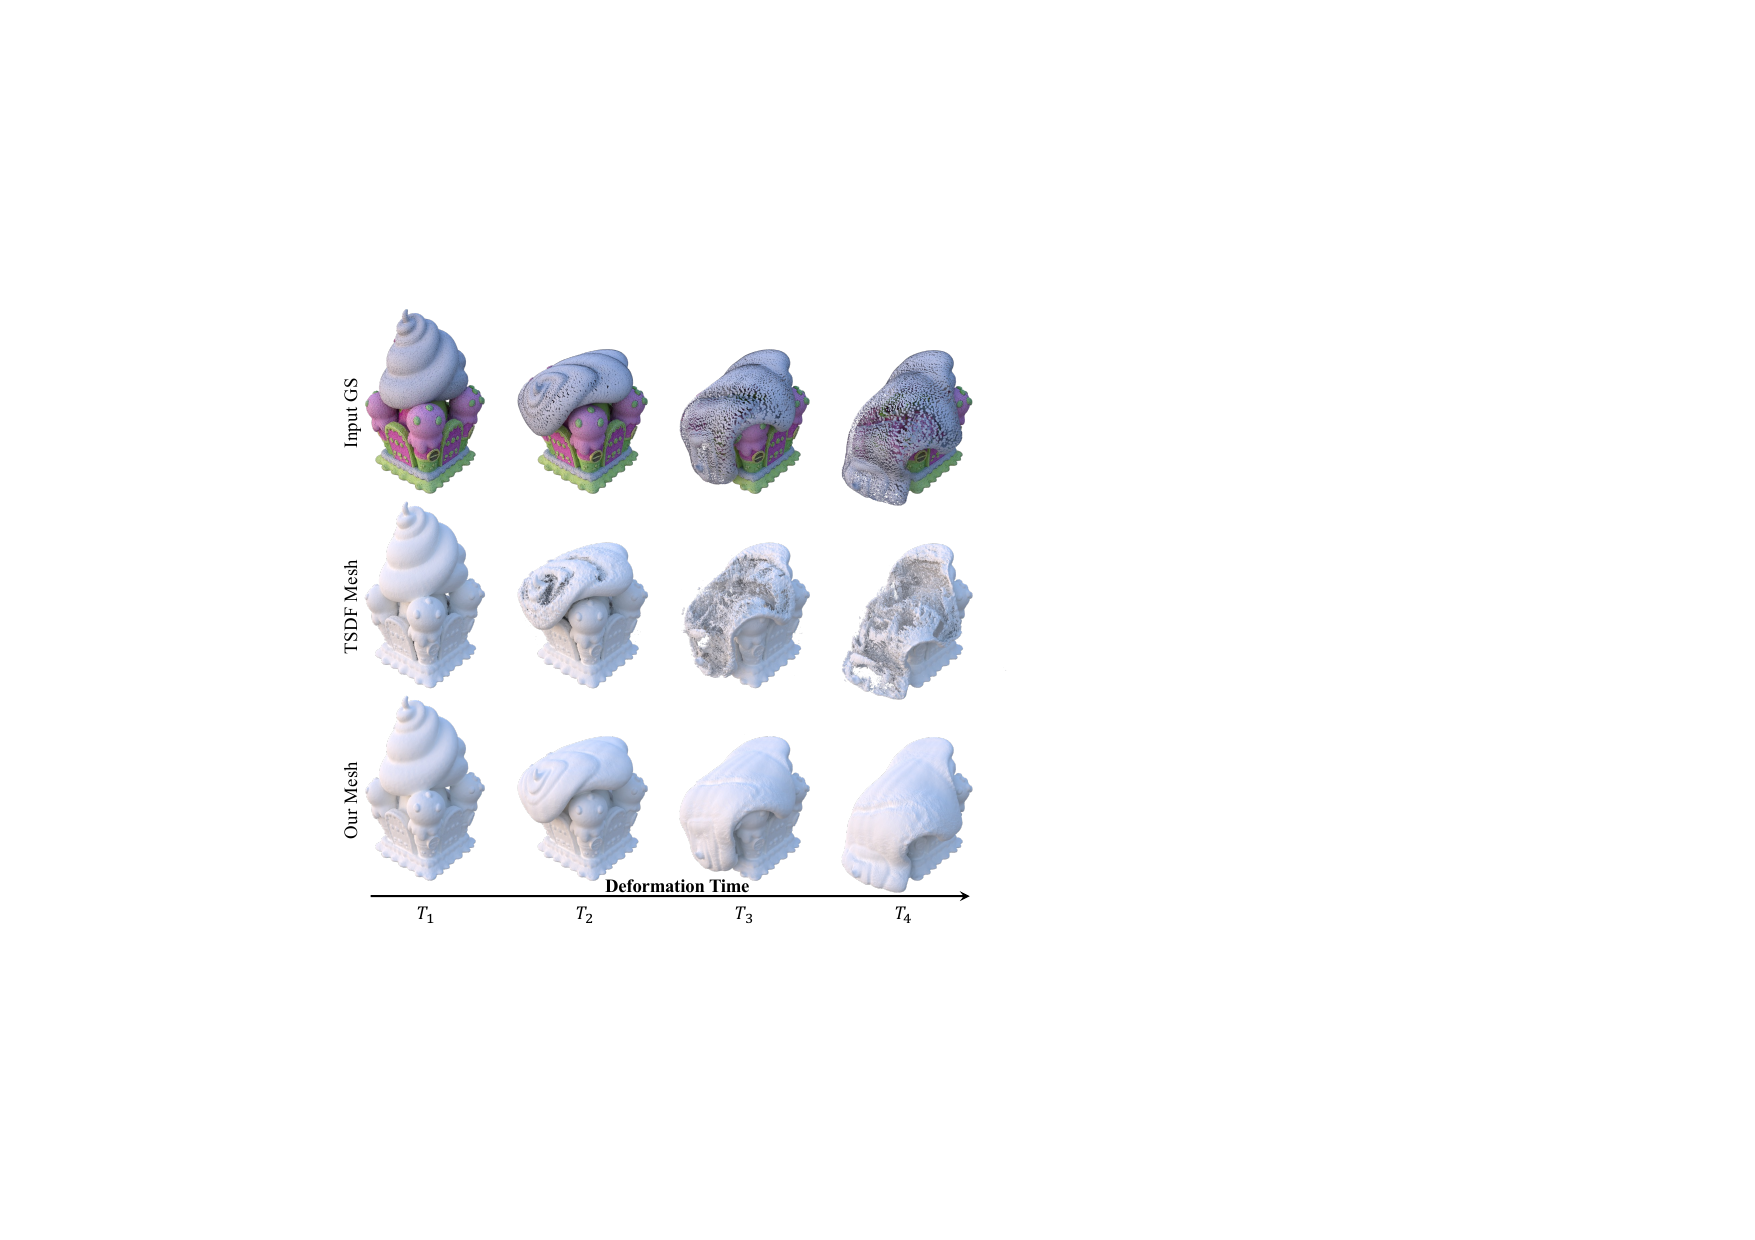}
    % \vspace{-1.0 em}
    \captionsetup{font=footnotesize}
    \caption{
    \textbf{Comparison of our IMLS GS-to-Mesh with TSDF-based baseline.}
    Compared with meshes obtained via TSDFusion, our approach, which combines Gaussian Splatting with IMLS, produces temporally more continuous and smoother surfaces while simultaneously preserving fine geometric details.
    }
    \label{fig:supp:mls_surface}
    % \vspace{-1.0 em}
% \end{figure}
\end{wrapfigure}

The resulting Gaussians $\{G_j^{p}\}$ are finally merged with the existing deformed surface Gaussians to produce the densified representation used for rendering.

We implement the above operation in CUDA, making its computational overhead negligible in practice.
Leveraging the IMLS formulation, we further reinterpret the Gaussian Splatting as a signed distance field and apply the Marching Cubes~\cite{lorensen1998marching} to extract high-quality meshes.
As illustrated in Fig.~\ref{fig:supp:mls_surface}, we compare our IMLS-based GS-to-mesh pipeline with a TSDF-fusion-based~\cite{newcombe2011kinectfusion} GS-to-mesh baseline, and our method consistently preserves finer geometric details.

% \clearpage
% \vspace{1.0 em}
\section{Computational Cost of Each Stage}
\label{supp:computation_cost}
% \vspace{-2.5 em}

\begin{table}[h]
\centering
\setlength{\tabcolsep}{2pt}

\resizebox{\linewidth}{!}{
    \Large
    % \fontsize{13pt}{14pt}\selectfont
    \begin{tabular}{lccccc}
        \toprule
        \textbf{Scene\textbackslash{}Module} 
        & \textbf{\#Splats (+ \#Filling)} 
        & \textbf{Internal Filling }
        & \textbf{MPM + LBM (substep) }
        & \textbf{IMLS Update }
        & \textbf{GS Rendering} \\
        \midrule
        % \multicolumn{6}{l}{\textbf{Synthetic scenes}} \\
        Candy house (\textit{Synthetic})
        & 154k (+103k) & 475 ms / 0.4 GB & 6 ms / 0.6 GB  & 375 ms / 0.9 GB   & 3 ms / 0.9 GB \\
        Lego (\textit{Synthetic})
        & 213k (+13k)  & 231 ms / 0.5 GB & 9 ms / 0.5 GB  & 419 ms / 0.8 GB   & 4 ms / 0.8 GB \\
        Toy bulldozer (\textit{Synthetic})
        & 52k (+47k)   & 206 ms / 0.3 GB & 8 ms / 0.4 GB  & 175 ms / 0.5 GB   & 2.0 ms / 0.5 GB \\
        
        \midrule
        
        % \multicolumn{6}{l}{\textbf{Real scenes}} \\
        Toy Sculpture (\textit{Real})
        & 683k (+70k)  & 662 ms / 1.3 GB & 13 ms / 1.2 GB & 1084 ms / 2.0 GB  & 7 ms / 1.9 GB \\
        Kitchen bulldozer (\textit{Real})
        & 175k (+25k)  & 288 ms / 0.4 GB & 9 ms / 0.5 GB  & 358 ms / 0.7 GB   & 3 ms / 0.8 GB \\
        Truck (\textit{Real})
        & 551k (+21k)  & 441 ms / 1.1 GB & 11 ms / 1.0 GB & 851 ms / 1.6 GB   & 9 ms / 1.5 GB \\
        \bottomrule
    % \vspace{-4.2 em}
    \end{tabular}
}

% \clearpage
\vspace{0.25 em}
\caption{Computational costs.}
% \vspace{-2.5 em}
\end{table}

Under the parameter settings in supp.Tab.~\ref{tab:mpm_params}, we show the
detailed per-scene costs with
runtime and peak GPU memory of each stage on an RTX 4070 
% \clearpage
12GB GPU.
In particular, the \textit{MPM+LBM} and \textit{IMLS update} stages are implemented using our custom Warp~\cite{macklin2022warp} CUDA kernels. The reported costs are measured per invocation of each stage. Note for real-world scenes, we only consider the segmented foreground object as mentioned in section.~\ref{supp:train_3dgs}.

% \begin{table}[h]
% \vspace{-2.0 em}
% \centering
% \large
% \caption{Computational costs.}
% \vspace{-1.0 em}
% \setlength{\tabcolsep}{4pt}
% \renewcommand{\arraystretch}{1.15}
% \resizebox{\linewidth}{!}{
% \begin{tabular}{l c c c c c}
% \specialrule{.1em}{.1em}{.1em}
% \textbf{Module} & \textbf{Internal Filling} & \textbf{MPM+LBM (substep)} & \textbf{IMLS Update} & \textbf{GS Rendering} & \textbf{GS Training} \\
% \textbf{Cost (Time/GPU)} & 200\,ms / 0.25\,GB & 10\,ms / 0.3\,GB & 150\,ms / 0.4\,GB & 2\,ms / 0.5\,GB & 5\,min / 2\,GB (30k steps) \\
% % \hline
% \specialrule{.1em}{.1em}{.1em}
% % \vspace{-4.5 em}
% \end{tabular}
% }
% \vspace{-2.0 em}
    
% \end{table}

\vspace{-1.0 em}
\section{Generalization of Topology-Adaptive Rendering}
\label{supp:general_topology_render}
\vspace{-0.25 em}
% 我们提出的Topology-Adaptive Gaussian Rendering make gaussian splats robuts and yield smoother geometry, 并且可以自然的泛化到其他MPM-driven deformations such as elastoplasticity. As shown in Fig.XX, 在一些特别极端的物理参数下，Naive 3DGS在MPM driven下出现了失败，物体断裂并且出现了极其明显的针状伪影，而我们的方法保持了合理的物理运动。

\begin{wrapfigure}{r}{0.4\linewidth}
% \hspace{-2.0 em}
% \vspace{-2.5 em} % 需要时微调
\centering
\animategraphics[autoplay,loop,width=\linewidth]{12}{figures/supp/elastic_large_deform/}{000000}{000023}
% \vspace{-2.25 em}
\caption{
Generalization to Other MPM-Driven Deformations and Improved Robustness
}

% \vspace{-2.875 em}

\label{fig:supp:elastic_large_deform}
\end{wrapfigure}

Our proposed Topology-Adaptive Gaussian Rendering enhances the robustness of Gaussian splats
% , produces smoother geometry, and naturally generalizes to other MPM-driven deformations, such as elastoplasticity.
by stabilizing splat geometry under extreme deformation, producing smoother surfaces, and naturally generalizing to other MPM-driven deformations such as elastoplasticity.
As shown in Fig.~\ref{fig:supp:elastic_large_deform}, under extreme physical parameter settings, naïve 3DGS breaks down with object fracture and severe needle-like artifacts. In contrast, our method maintains physically plausible motion throughout the deformation process.
\textbf{Please view the dynamic video in Fig.~\ref{fig:supp:elastic_large_deform} in \textcolor{red}{Adobe Acrobat Reader}.}
% \pagebreak[0]
\vspace{-0.75 em}
\section{Details for Thermophysical Scene Editing}
\label{supp:exp_edit}
\vspace{-0.25 em}
We compare \method with three representative editing pipelines: DGE~\cite{chen2024dge}, a text-driven diffusion-based editing method for 3DGS; 
AutoVFX~\cite{hsu2025autovfx}, which leverages an LLM model~\cite{achiam2023gpt} to generate scripts for external physics engines to perform mesh-based melting and composite the results back into the scene;
Runway Gen-4.5~\cite{runway_gen4}, a leading commercial image-to-video generation model that augments a single input image with text-guided dynamic effects. 

\iffalse
For DGE, we use the prompt "Turn the (Truck/Sculpture/Lego Dozer) into a melted like" with guidance scale=15 and optimize the GS model with 15k iterations, DGE只能实现静态场景的风格编辑，无法实现动态效果，同时对于融化这种物理驱动的现象拟合效果有限;
For AutoVFX, we use the prompt "Melt the (Truck/Sculpture/Lego Dozer)", AutoVFX对场景使用Bakedsdf重建出Mesh，通过GPT自动分割前景并调取Blender的FLIP仿真算法实现融化效果，时间成本较大，且没有考虑融化效果与原始场景appearance上的一致性；
For Runway Gen-4, we输入各个视角的静态渲染图像作为image condition并use the prompt "The camera keep state, over time the (Truck/Sculpture/Lego Dozer) begins to melt", Runway Gen-4在视觉上实现了vivid dynamic effects, 但是结果并不满足物理合理性，且没有考虑物体自身的材质appearance，同时各个视角的编辑效果独立，无法保证时序上的多视角一致性。
\fi

\textbf{For DGE}, we use the prompt  
\emph{``Make the (Truck / Sculpture / Lego Dozer) look melted''}  
with a guidance scale of $15$, and optimize the 3DGS model for $15$k iterations. 
Since DGE utilizes an image-level diffusion as prior, it can only perform style editing of static scenes and does not produce explicit dynamic motion. 
Moreover, its ability to faithfully capture melting, which is inherently a physics-driven phenomenon, is limited and often results in only superficial, texture-level changes.
\textbf{For AutoVFX}, we use the prompt  
\emph{``Melt the (Truck / Sculpture / Lego Dozer)''}.  
AutoVFX first reconstructs a mesh representation of the scene, then uses GPT-based scripting to automatically segment the foreground object and invoke Blender’s FLIP fluid simulation to realize a melting effect. 
While this pipeline can generate physically plausible deformations on the mesh, it incurs substantial computational overhead and does not explicitly enforce appearance consistency between the simulated melting result and the original scene, leading to noticeable appearance discrepancies in the final composites.
\textbf{For Runway Gen-4.5}, we input per-view static renderings of the reconstructed scene as image conditions and use the prompt  
\emph{``The camera keeps still, and over time the (Truck / Sculpture / Lego Dozer) begins to melt''}.  
Runway Gen-4.5 produces visually vivid dynamic effects, however, the generated motion is not constrained by physical laws and often violates basic physical plausibility. 
In addition, the model does not preserve the original material appearance of the object consistently, and each viewpoint is edited independently, which leads to temporal and multi-view inconsistencies across the different camera trajectories.

\noindent\textbf{User Study.}
We recruited 27 participants, and each participant was asked to evaluate 24 videos generated by different methods and from different viewpoints, and to rank the results according to their personal preference.
We present the user evaluation interface with one representative example as shown in Fig.~\ref{fig:supp:user_study}.

% 额外的视频生成模型对比
\begin{figure}[t] \centering
    % \vspace{-1.375 em}
    \includegraphics[width=0.95\linewidth]{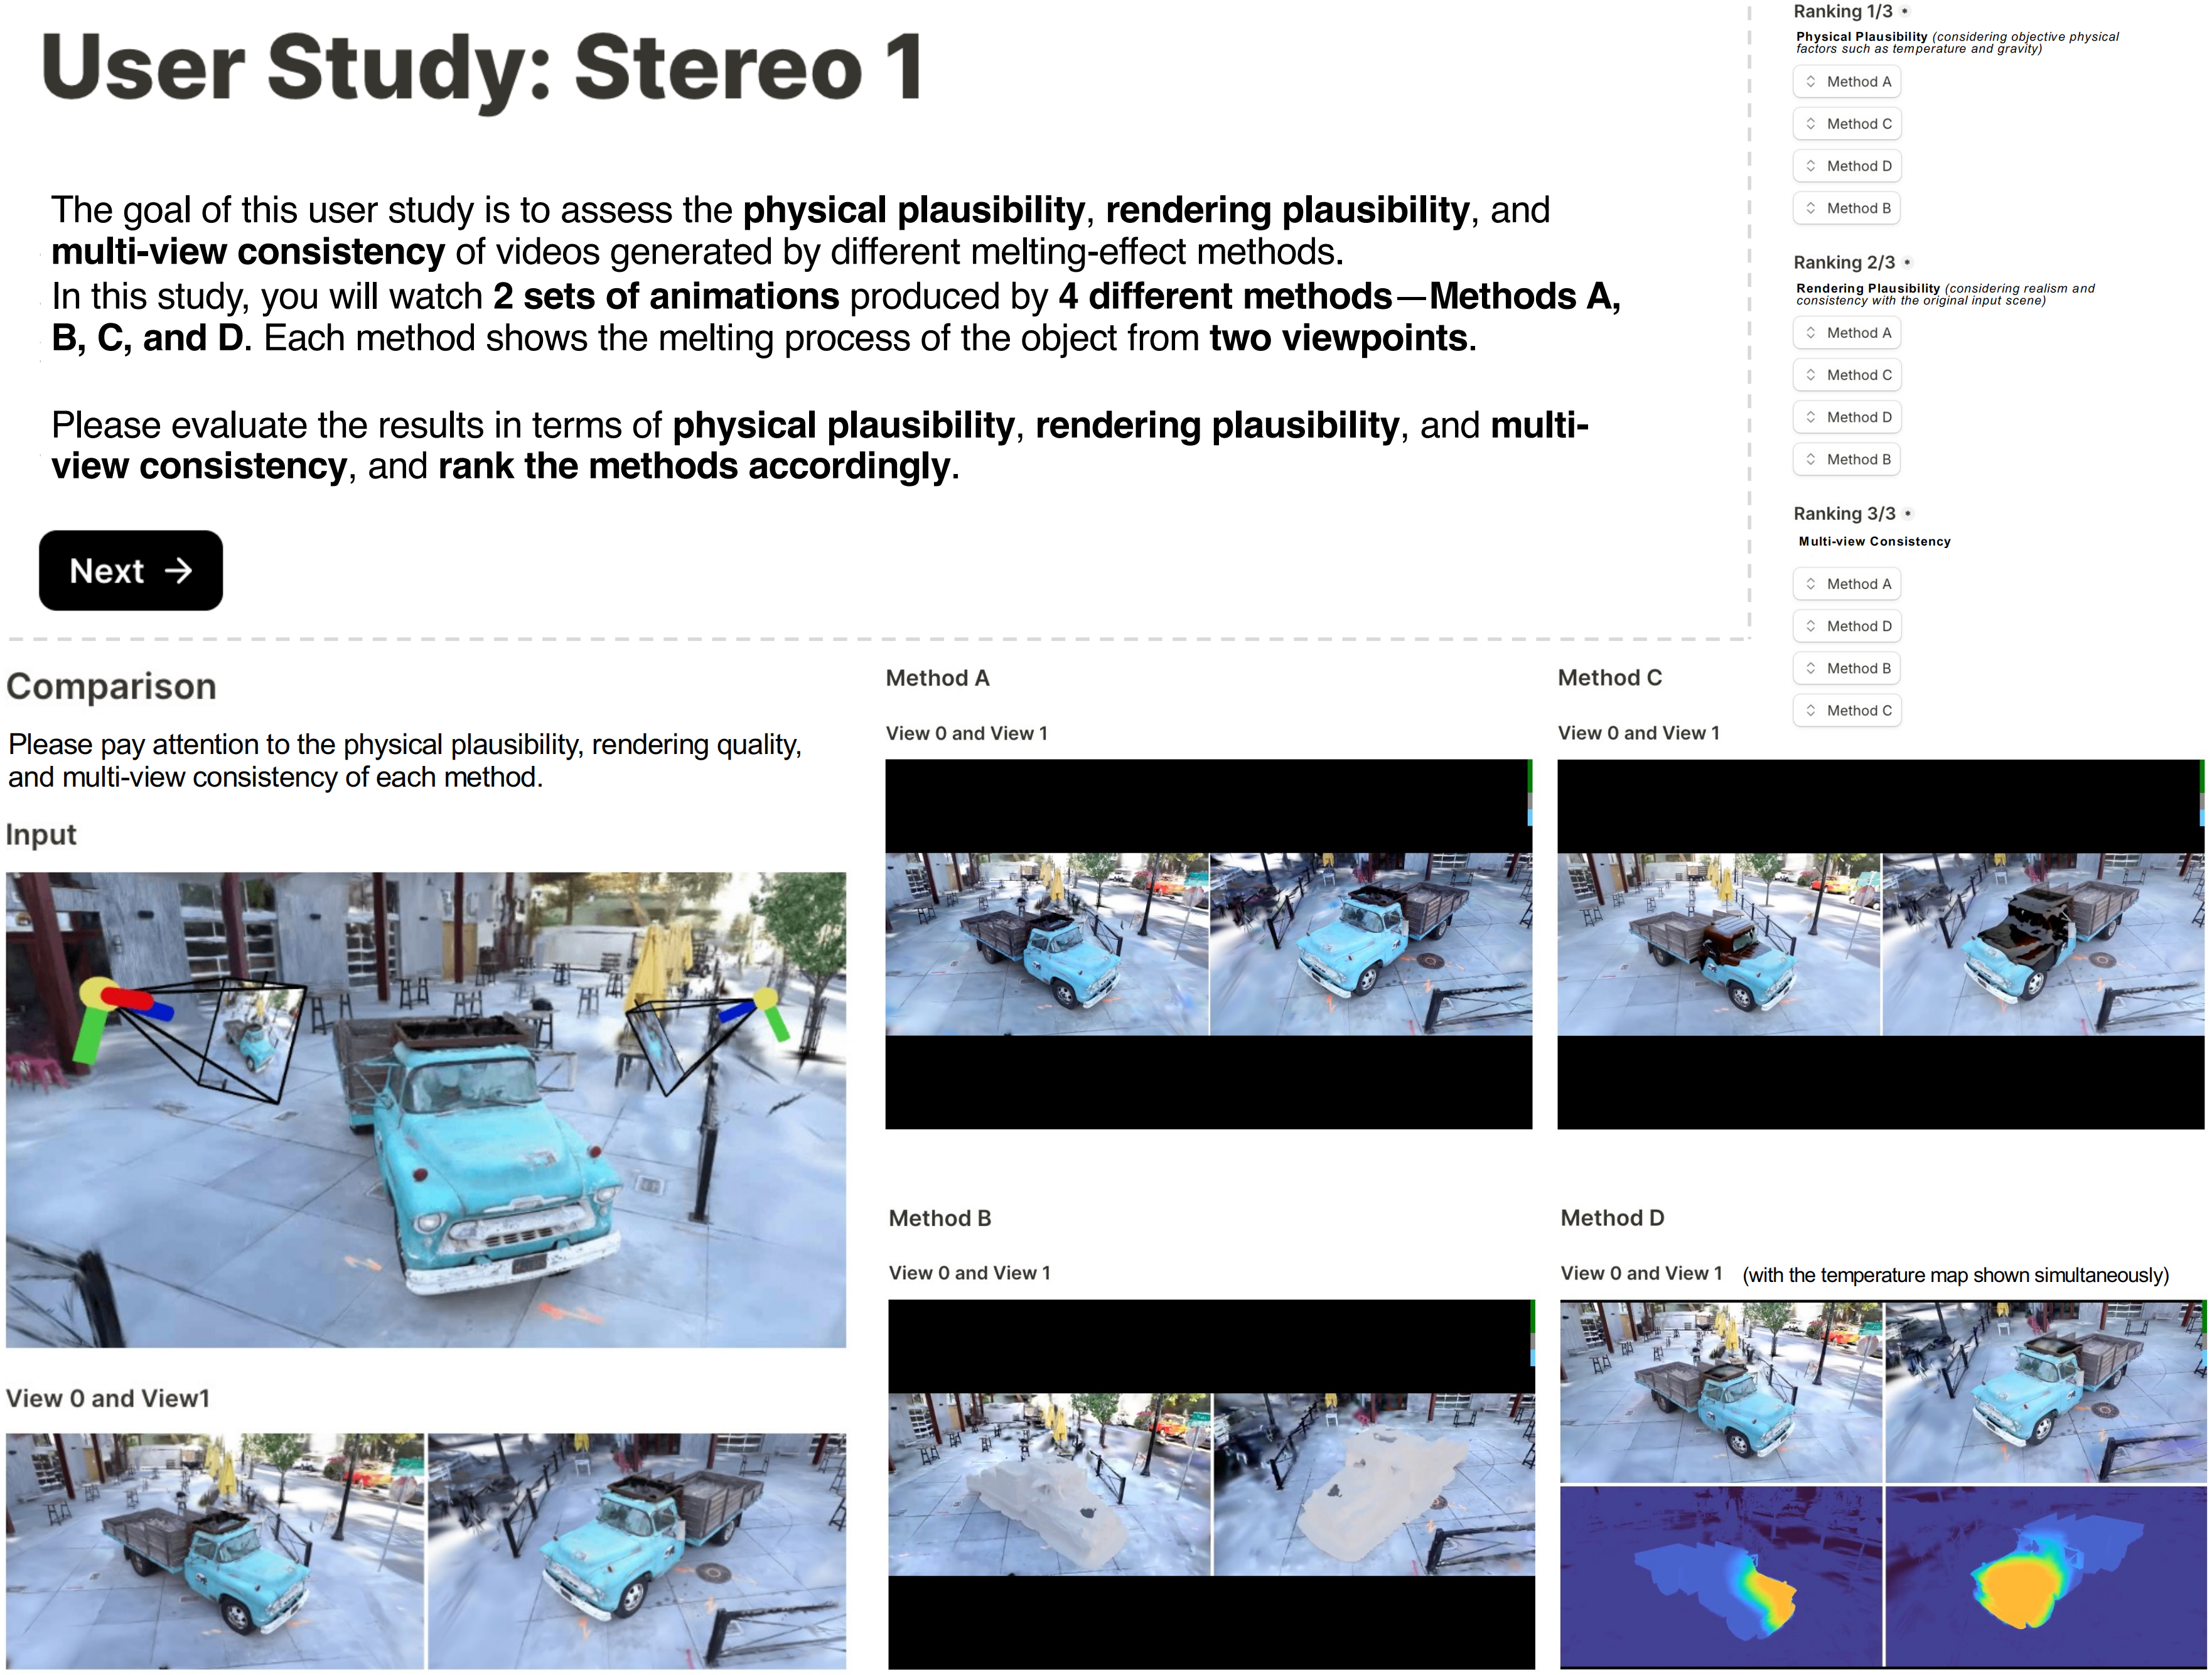}
    % \animategraphics[autoplay,loop,width=\linewidth]{15}{figures/supp/extra_video_gen/}{000000}{000023}
    % \vspace{-0.625 em}
    \caption{
    \textbf{The user evaluation interface.}
    We rearranged the layout of the interface to present it more clearly in the paper.
    }
    \label{fig:supp:user_study}
    \vspace{0.5 em}
\end{figure}

\begin{figure}[t] \centering
    % \vspace{-1.25 em}
    % \includegraphics[width=0.475 \textwidth]{figure/rebuttal/2_complex_scene.pdf}
    \animategraphics[autoplay,loop,width=\linewidth]{15}{figures/supp/extra_video_gen/}{000000}{000023}
    % \vspace{-2.0 em}
    \caption{
    \textbf{Comparison with extra video generation models.} Please view the dynamic videos in \textcolor{red}{Adobe Acrobat Reader}.
    }
    \label{fig:supp:extra_video_gen}
    % \vspace{-1.5 em}
\end{figure}

\noindent\textbf{Additional SOTA Video Generation Comparisons.}
We further compare our method against additional state-of-the-art video generation models, including Veo 3~\cite{veo3_google2025}, Wan 2.6~\cite{wan26_wan2026} and Kling 2.6~\cite{kling26_kuaishou2025}, to show that, for highly physics-grounded animations, although all of them produce vivid visual effects, even recent state-of-the-art video generation models still struggle with controllability, physical plausibility, and multi-view consistency (\textbf{please view the dynamic videos in Fig.~\ref{fig:supp:extra_video_gen} in \textcolor{red}{Adobe Acrobat Reader}}). 
For specific physical phenomena such as melting, coupling with explicit physics simulators remains essential.
This is also supported by prior works, where explicit simulation has been widely adopted as an effective paradigm for modeling specialized physical phenomena, such as in RainyGS~\cite{dai2025rainygs}, FieryGS~\cite{shen2026fierygs}, GaussianSplashing~\cite{feng2025gaussian}, and EnliveningGS~\cite{shen2025enliveninggs}, enabling data-free, controllable, and physically plausible animations.
% 我们比较了更多sota的video generation模型 Veo3/Wan2.6/Kling2.6 来说明for highly physical-grounded animations, 尽管all produce vivid effects but even SOTA models still struggle with controllability, physical plausibility and multi-view consistency. For specific physical phenomena like melting, coupling explicit physics simulators remains necessary.

\vspace{-0.5 em}
\section{Quantitative Evaluation against Simulation Platform}
\vspace{-0.25 em}
\label{supp:houdini_simulation}
We add a quantitative evaluation against independent mesh-based thermomechanical simulation references generated by Houdini~\cite{houdini}, a professional physical simulation platform, 
under the same heat-source and thermal-boundary setup as our method, these simulations provide an independent physics-based reference.
The temporally averaged surface accuracy shows \method aligns well with the reference while preserving photorealism. 

\begin{figure}[h] \centering
    \vspace{-2.0 em}
    \includegraphics[width=0.975 \textwidth]{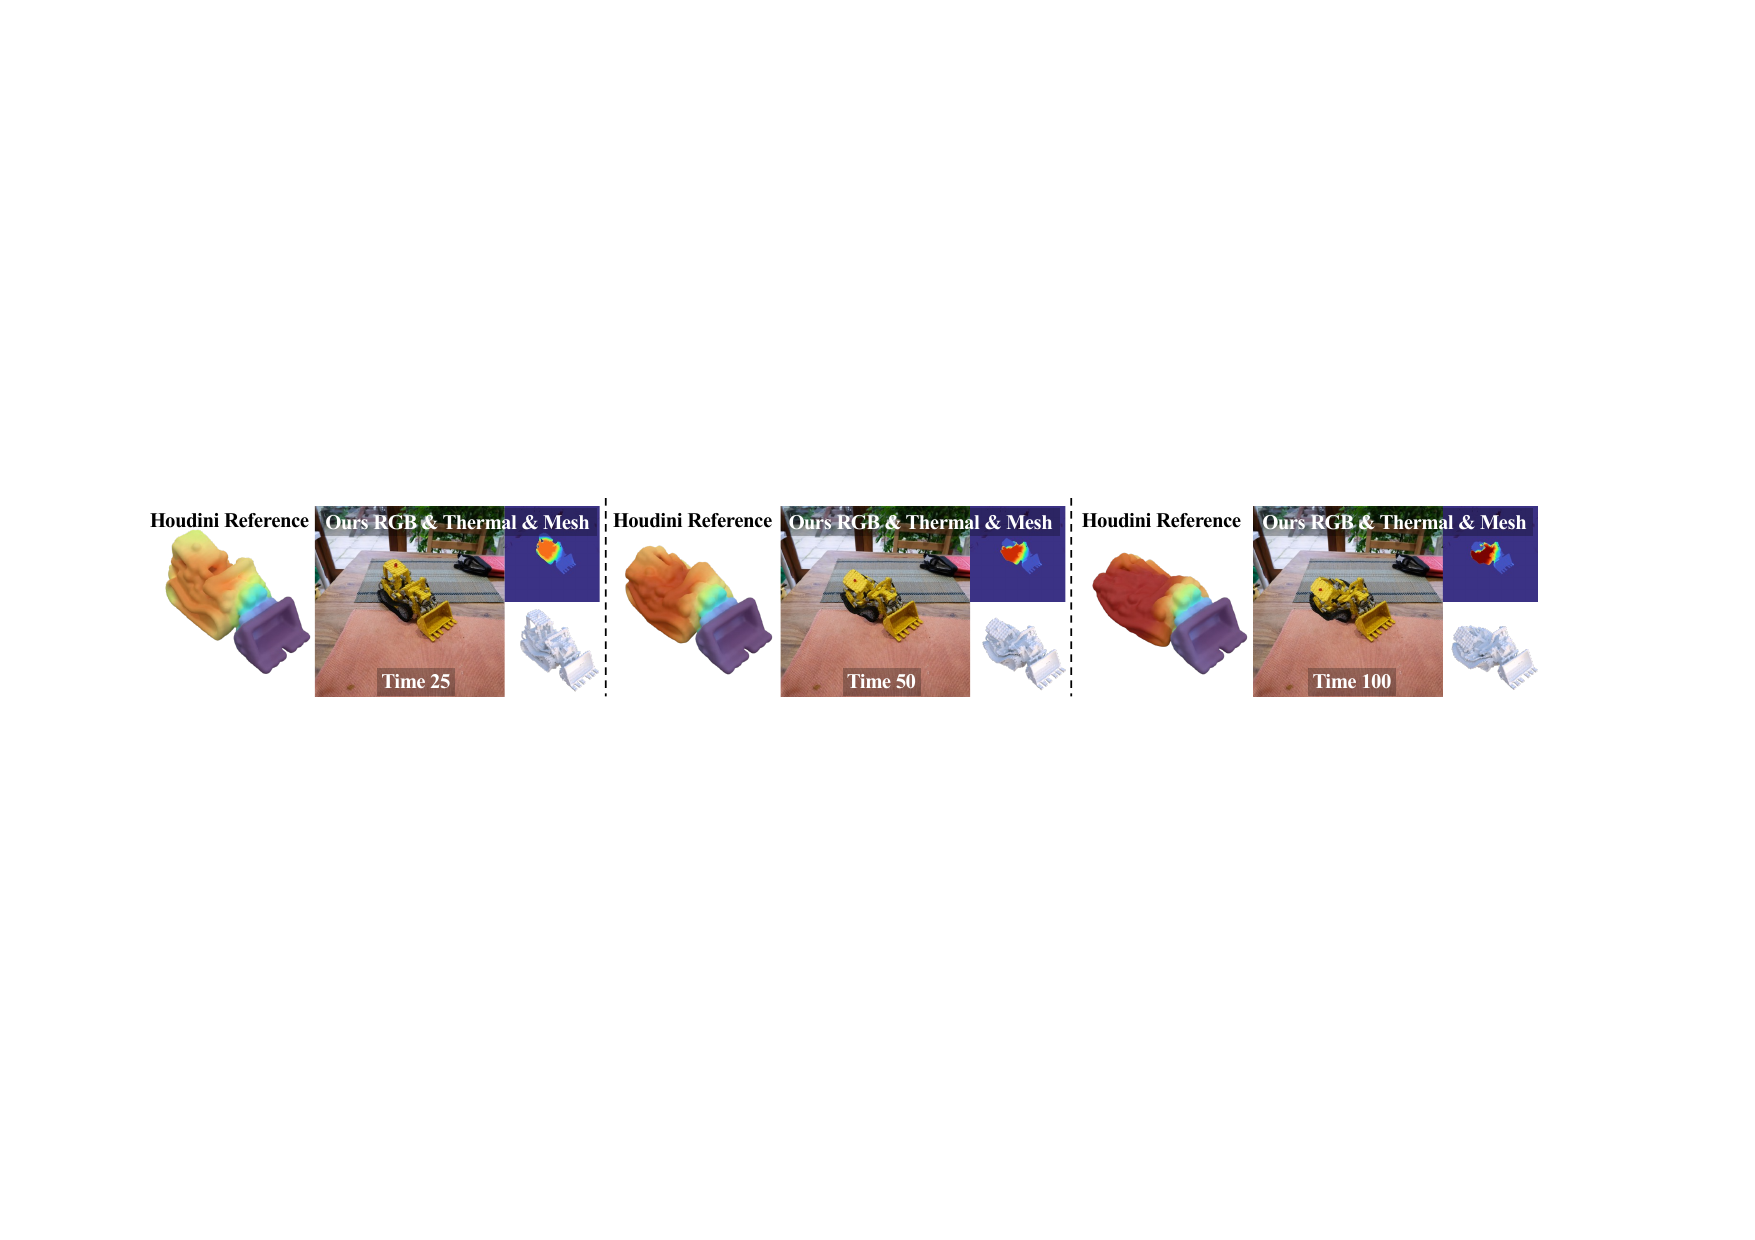}
    \vspace{-4.0 em}
\end{figure}

\begin{table}[h]
\centering
\large
\setlength{\tabcolsep}{4pt}

% \vspace{-1.0 em}
\resizebox{0.9\textwidth}{!}{
    \begin{tabular}{lcccc}
    \specialrule{.1em}{.1em}{.1em}
    Method       
    & Chamfer Distance $\downarrow $
    & F-score $\uparrow $
    & $\mathrm{Depth}_{\mathrm{RMSE}}$ $\downarrow$ 
    & Silhouette IoU $\uparrow$ \\
    \midrule
    PhysGaussian & 0.089 & 0.08 & 0.130 & 0.435 \\
    Ours         & \textbf{0.037} & \textbf{0.23} & \textbf{0.065} & \textbf{0.789} \\
    \specialrule{.1em}{.1em}{.1em}
    % \vspace{-3.375 em}
    \end{tabular}
}
\end{table}

\vspace{-2.5 em}
\section{Handling Different Materials}
\vspace{-0.25 em}
\label{supp:seg_material}
% \begin{figure}[t] \centering
\begin{wrapfigure}[6]{r}{0.7\linewidth}
    \vspace{-2.0 em}
    \includegraphics[width=\linewidth]{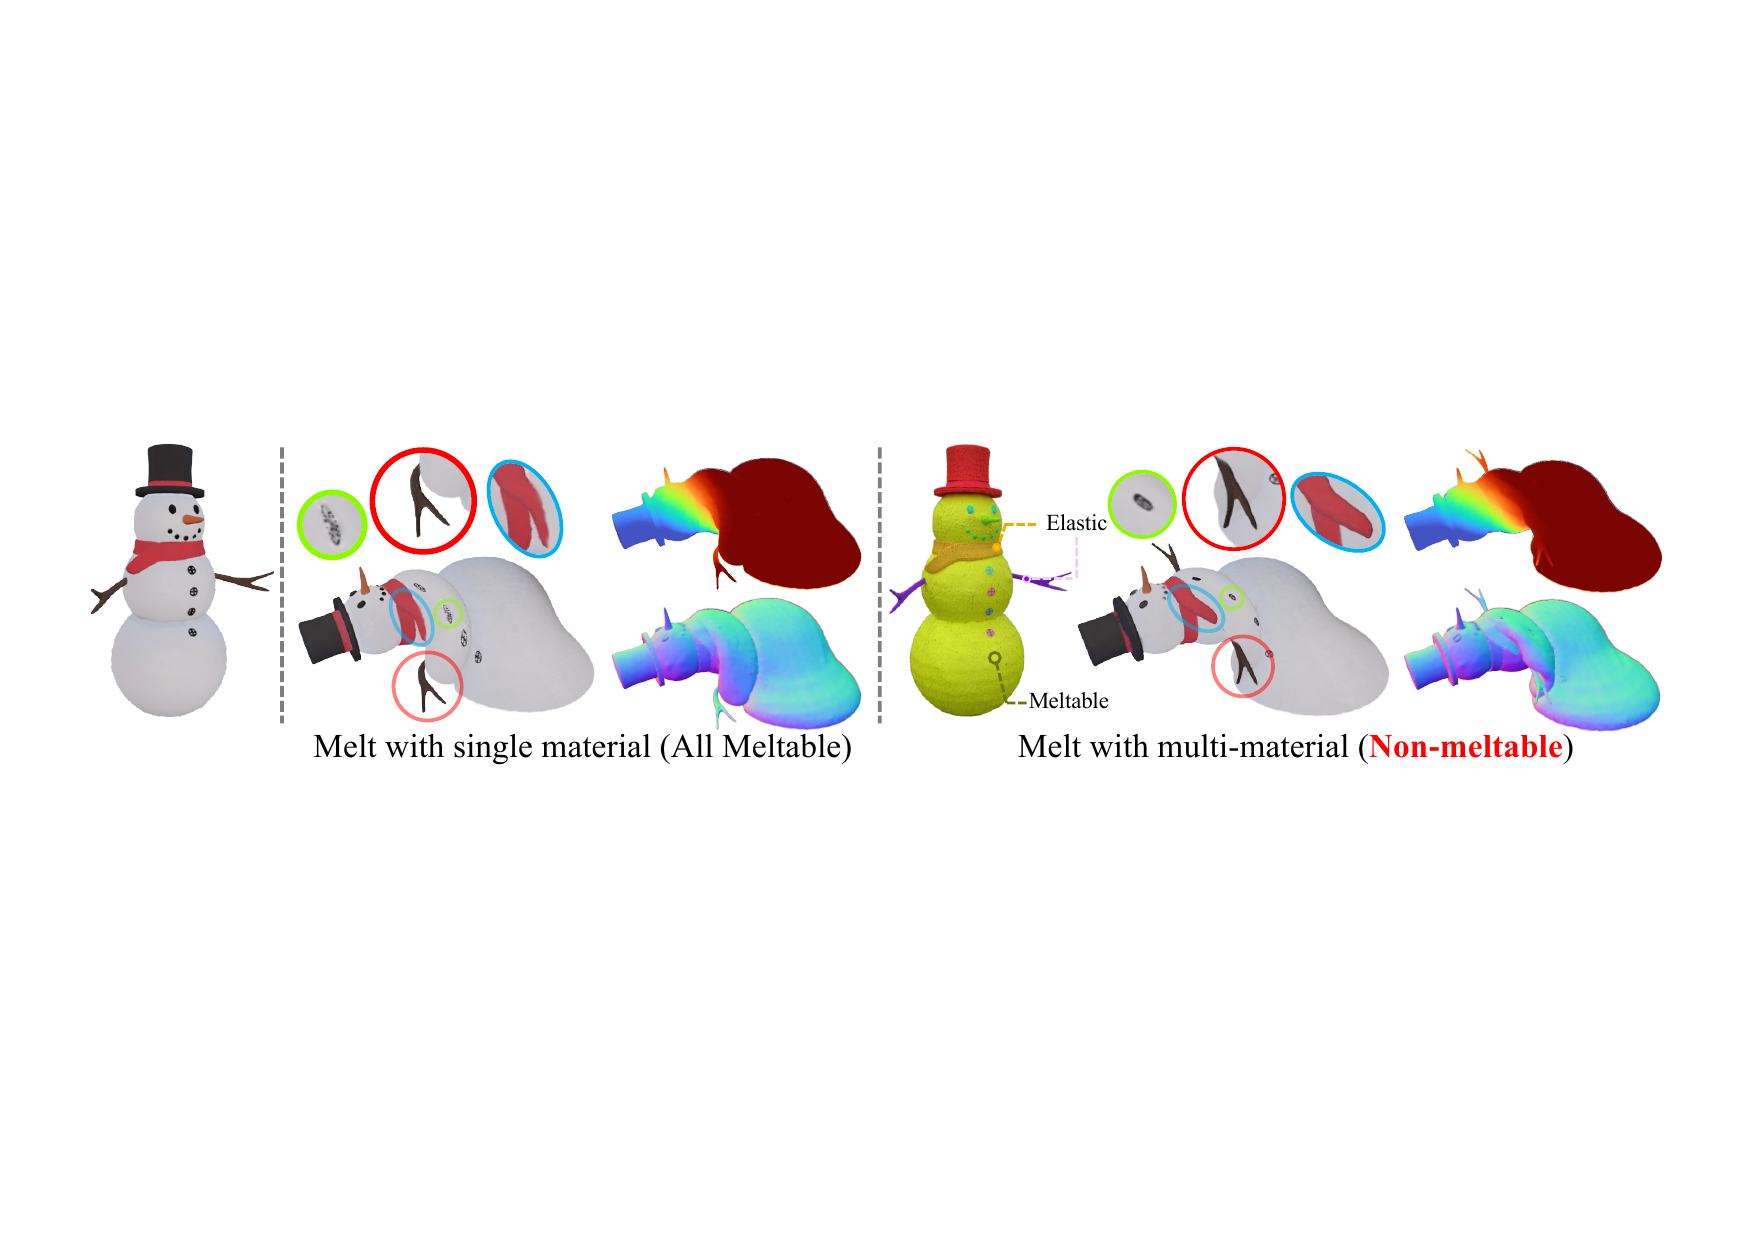}
    % \vspace{-2.0 em}
    \caption{
    Multi-material melting.
    }
    \label{fig:supp:multi_material_melt}
    \vspace{-1.5 em}
\end{wrapfigure}

We further consider multi-material thermophysical editing by performing part-level segmentation and assigning material-specific constitutive models to different object parts.
As shown in Fig.~\ref{fig:supp:multi_material_melt}, object components such as buttons and branches are specified as non-meltable materials (e.g., elastic),
while the snow regions remain thermally deformable, producing distinct deformation behaviors across materials and demonstrating that MeGAS can be naturally extended to handle heterogeneous material compositions.
% We further consider multi-material melting by performing part-level segmentation and assigning material-specific constitutive models to different object parts. This enables distinct deformation behaviors across materials and demonstrates that MeGAS can be naturally extended to handle heterogeneous material compositions.

\section{Additional Multi-view Results}
\vspace{-0.25 em}
\label{supp:multiview_render}
We provide additional multi-view rendering results for Section~\textcolor{red}{5.2} to further demonstrate cross-view consistency under large deformations as shown in Fig.~\ref{fig:supp:mv_render}. 
\textbf{Please view the dynamic videos in \textcolor{red}{Adobe Acrobat Reader}.}

\begin{figure}[h] \centering
    \vspace{-1.5 em}
    \animategraphics[autoplay,loop,width=\linewidth]{15}{figures/supp/mv_render/}{000000}{000029}
    \vspace{-1.5 em}
    \caption{
    Additional multi-view rendering results.
    }
    \label{fig:supp:mv_render}
    % \vspace{-2.5 em}
\end{figure}

\section{Additional Results on Real-World Scenes}
\label{supp:more_real_data}
As shown in Fig.~\ref{fig:supp:more_results}, we visualize the thermomechanical dynamics of our method under heat-diffusion control. As the temperature field propagates through the object, phase-change-aware control triggers constitutive model switching, yielding realistic melting-style scene editing. 
We illustrate the deformation process on real-world scenes, with rendered RGB images, rendered temperature field, and deformation geometries (rendered normals and meshes) at different viewpoints and time steps. 
% Our method achieves high physical plausibility as well as strong temporal and multi-view consistency.
Our method produces physically plausible thermomechanical dynamics while maintaining strong temporal and multi-view consistency.

\begin{figure*}[t] % 使用 !t 尝试强制图像置顶
    \centering
    \scriptsize
    \vspace{-3.0 em}
    \includegraphics[width=\textwidth]{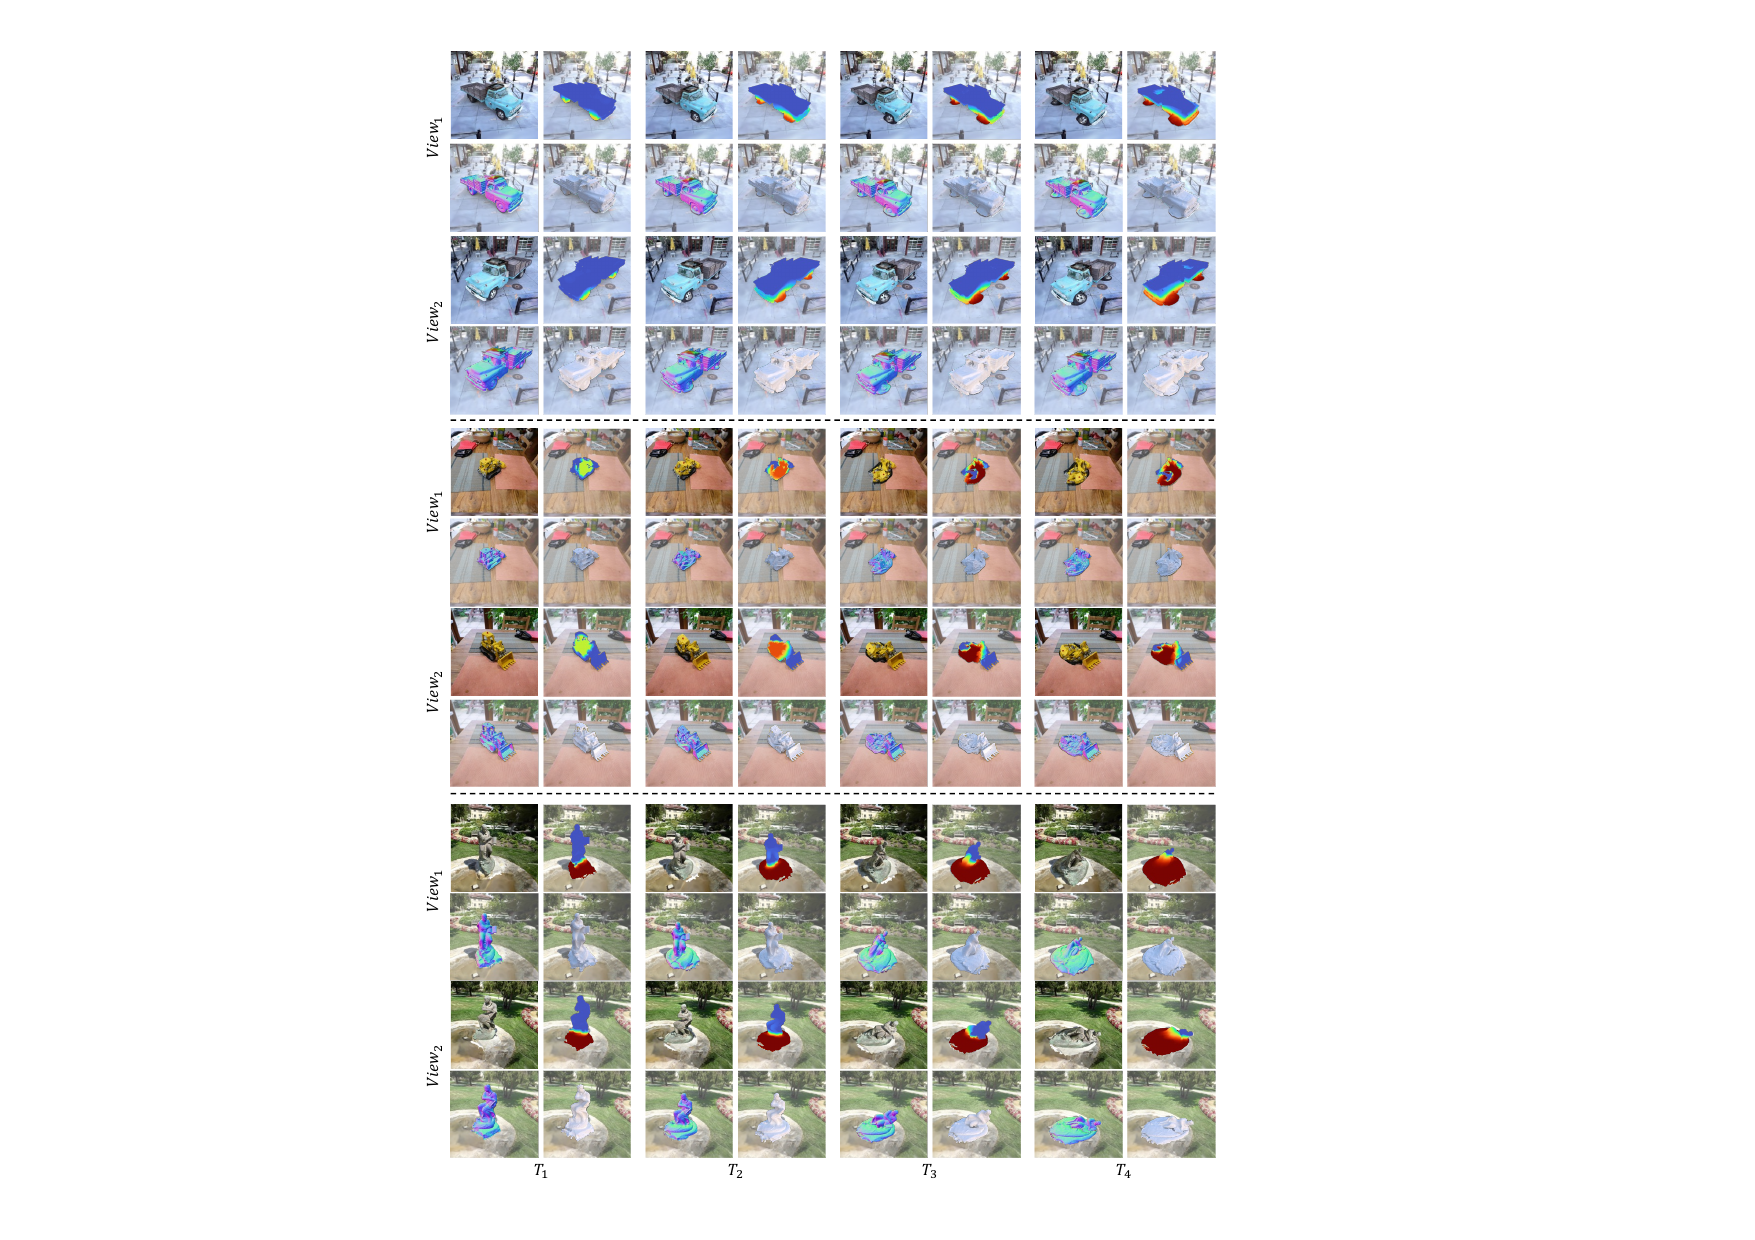}
    % \vspace{-2.5 em}
    \caption{
    \textbf{Our thermophysical scene editing.}
    We illustrate the deformation process on real-world scenes, with rendered RGB images, rendered temperature field, and deformation geometries (rendered normals and meshes) at different viewpoints and time steps.
    }
    \vspace{-0.75 em}
    \label{fig:supp:more_results}
\end{figure*}

\clearpage

% 物体级别的多视图

% Elastoplasticity

% Computational cost

% ---- Bibliography ----
%
% BibTeX users should specify bibliography style 'splncs04'.
% References will then be sorted and formatted in the correct style.
%
% \bibliographystyle{splncs04}
% \bibliography{main}
% \end{document}
