# Supplementary material for: MeGAS: Thermomechanical Dynamic Gaussian Splatting for Thermophysical Scene Editing
Source: arXiv:2606.23455 source file (2026-06-22)
Supplement: Supplementary file 2 [file 0_train_details.tex]

% This document provides (1) training details for the topology-adaptive GS, (2) full formulations and implementation details of the MPM–LBM simulator, (3) derivations and implementation of the implicit-surface-guided densification, (4) prompt and parameter settings for editing baselines, and (5) additional qualitative results.
This supplementary material provides detailed descriptions of the training procedure for topology-adaptive Gaussian Splatting (Sec. \ref{supp:train_3dgs}), the full formulations and implementation details of the MPM-LBM simulator (Sec. \ref{supp:mpm_lbm}), the derivation and implementation of the implicit-surface-guided densification module (Sec. \ref{supp:imls_densify}), the computational cost analysis of each stage (Sec.~\ref{supp:computation_cost}), the generalization behavior of topology-adaptive rendering (Sec. \ref{supp:general_topology_render}), the experimental setup for thermophysical scene editing including baseline prompts, parameter settings, and user-study details (Sec. \ref{supp:exp_edit}), and additional qualitative results on multi-material editing, multi-view consistency, and real-world scenes (Secs. \ref{supp:seg_material}-\ref{supp:more_real_data}).

\vspace{-0.5 em}
\section{Details for Training Topology-Adaptive GS}
\label{supp:train_3dgs}
\vspace{-0.25 em}
% 我们首先使用COLMAP对输入的图像序列以获取位姿和稀疏点云。除了得到逼真的渲染，我们还希望重建的3DGS模型能够有较好的几何，因此在原有3DGS的Pipeline基础上，我们加入了PGSR中的Plane约束，which包括约束|min(s1,s2,s3)|使gs接近于平面surfel，以及使用unbiased plane depth约束depth和normal的一致性。
% 在PGSR的基础上，我们使用了Sec.4.2.1 Internal-Free Uniform Gaussian Regularization来进一步抑制大形变时内部Floater的暴露和gs分布不均匀导致的needle-like floaters。We train 3DGS with the plane-aware regularization from PGSR以及我们的anisotropy loss for 30k iterations:
% L = L_rgb(I,I) + L_geo() + lambda_anisotropy * L_ani
% 我们在训练过程中每2500步开启一次Low-contribution Gaussian Pruning，the weight-pruning threshold tau_prune we used is 0.2，同时我们每1000步apply 一次scale clamping with tau_scale = 1/128. All experiments are conducted on a single NVIDIA RTX 4090 GPU.
% 我们在NeRF-Synthetic Dataset上测试了我们模块对PSNR的影响，在减少内部floater以及得到更均匀的GS分布同时，保持了一样的渲染质量。
We first run COLMAP~\cite{schonberger2016structure} with the input image sequence to estimate the camera poses and sparse point cloud for reconstruction. 
Building on the vanilla 3D Gaussian Splatting pipeline~\cite{kerbl3Dgaussians}, we incorporate the planar regularization from \cite{chen2024pgsr,huang20242d} to improve geometric fidelity.
Specifically, each Gaussian is encouraged to approximate a local plane by penalizing the smallest principal scale $||\min(s_1, s_2, s_3)||_{1}$, and we adopt the unbiased plane-depth regularization to enforce consistency between the rendered depth and the corresponding surface normals to further align with the underlying surface.
On top of the planar regularization, we apply our internal-free uniform Gaussian regularization, introduced in Sec.~\textcolor{red}{4.2.1} of the main paper, to enhance robustness under large deformations.
The topology-adaptive 3DGS is optimized for 30k iterations with a joint loss:
\begin{equation}
    \mathcal{L}
    = \mathcal{L}_{\mathrm{rgb}}
    + \mathcal{L}_{\mathrm{geo}}
    + \lambda_{\mathrm{aniso}} \mathcal{L}_{\mathrm{aniso}},
\end{equation}
where $\mathcal{L}_{\mathrm{rgb}}$ is the photometric loss from 3DGS~\cite{kerbl3Dgaussians}, $\mathcal{L}_{\mathrm{geo}}$ corresponds to the planar constraints from PGSR~\cite{chen2024pgsr}, and $\mathcal{L}_{\mathrm{aniso}}$ is our anisotropy loss.
The weight for anisotropy regularization $\lambda_{\mathrm{aniso}}$ is set to 0.1. 
During training, we perform low-contribution Gaussian pruning every 2{,}500 iterations with the pruning threshold of $\tau_{\text{prune}} $=$0.2$, and apply scale clamping every 1{,}000 iterations by truncating the principal scales with an upper bound $\tau_{\text{scale}}$=$1/128$.

Moreover, since we define each Gaussian normal as the direction of its shortest principal axis, the normal is ambiguous up to a sign in the absence of camera. To resolve this ambiguity, we introduce a learnable pseudo normal for each Gaussian and perform a short self-distillation stage after training. Each pseudo normal $\mathbf{n}'_i$ is randomly initialized and optimized using the rasterized Gaussian normal $\mathbf{n}_i$ as a pseudo label, with the loss:
\begin{equation}
\mathcal{L}_{\text{normal}} = \|\mathbf{N}' - 
\mathrm{stopgrad}(\mathbf{N})
\|_1,
\end{equation}
where $\mathbf{N}'$=$\sum_i T_i \alpha_i \mathbf{n}'_i$ and $\mathbf{N}$=$\sum_i T_i \alpha_i \mathbf{n}_i$. We finetune it for 500 iterations and 
% \clearpage\noindent
correct the orientation of Gaussian normals by enforcing alignment with the directions of the pseudo normals.

\begin{wraptable}{r}{0.475 \textwidth}
\vspace{-0.25 em}
\caption{
\textbf{Ablation of rendering quality.} 
We progressively add each module on top of the backbone. Our module substantially reduces internal floaters and yields a more uniform Gaussian distribution, while maintaining comparable PSNR.
Although the anisotropy regularization slightly degrades PSNR, the subsequent scale clamping recovers the rendering quality.
}
\vspace{1.0 em}
% \begin{table}[t]
\resizebox{\linewidth}{!}{
\begin{tabular}{lccc}
\specialrule{.1em}{.1em}{.1em}
Module (Progressively Add)    & PSNR$\uparrow$ & SSIM$\uparrow$ & LPIPS$\downarrow$ \\
\midrule
Backbone~\cite{chen2024pgsr}  & 37.33          & 0.9813          & 0.031             \\
\midrule
w/ Internal Pruning           & 36.76          & 0.9801          & 0.035             \\
w/ Anisotropy Reg.            & 35.81          & 0.9767          & 0.045             \\
w/ Scale Clamping             & 37.24          & 0.9805          & 0.031             \\
\specialrule{.1em}{.1em}{.1em}
\end{tabular}
}
\vspace{-2.0 em}

\label{supp:tab:psnr}
% \end{table}
\end{wraptable}

We additionally validate our internal-free uniform Gaussian regularization on the NeRF-Synthetic dataset~\cite{mildenhall2021nerf} in terms of rendering quality. 
As shown in Tab.~\ref{supp:tab:psnr}, the regularization substantially reduces internal floaters and yields a more uniform Gaussian distribution, while maintaining comparable PSNR to the vanilla PGSR~\cite{chen2024pgsr} baseline.

% 对于室外场景，我们会先使用PGSR对场景进行正常重建，然后分割出前景，Specifically，我们先使用GroundedSAM通过前景的prompt，i.e. "Truck","Lego Dozer"，获得多视图2D mask，然后使用对比学习实现前景的3D分割，之后对其使用internal-free uniform Gaussian regularization
For outdoor scenes, we first perform scene reconstruction with PGSR and then extract the foreground. Specifically, we employ GroundedSAM~\cite{ren2024grounded} with foreground prompts (e.g., “\textit{Truck}”, “\textit{Lego Dozer}”) to obtain multi-view 2D masks, and subsequently perform 3D foreground segmentation via contrastive learning~\cite{ying2024omniseg3d}. The resulting foreground Gaussians are then refined using our internal-free uniform Gaussian regularization.
All experiments are conducted on an NVIDIA RTX 4090 24GB GPU.

\begin{figure}[h] \centering
    \vspace{-2.0 em}
    \includegraphics[width=0.975 \textwidth]{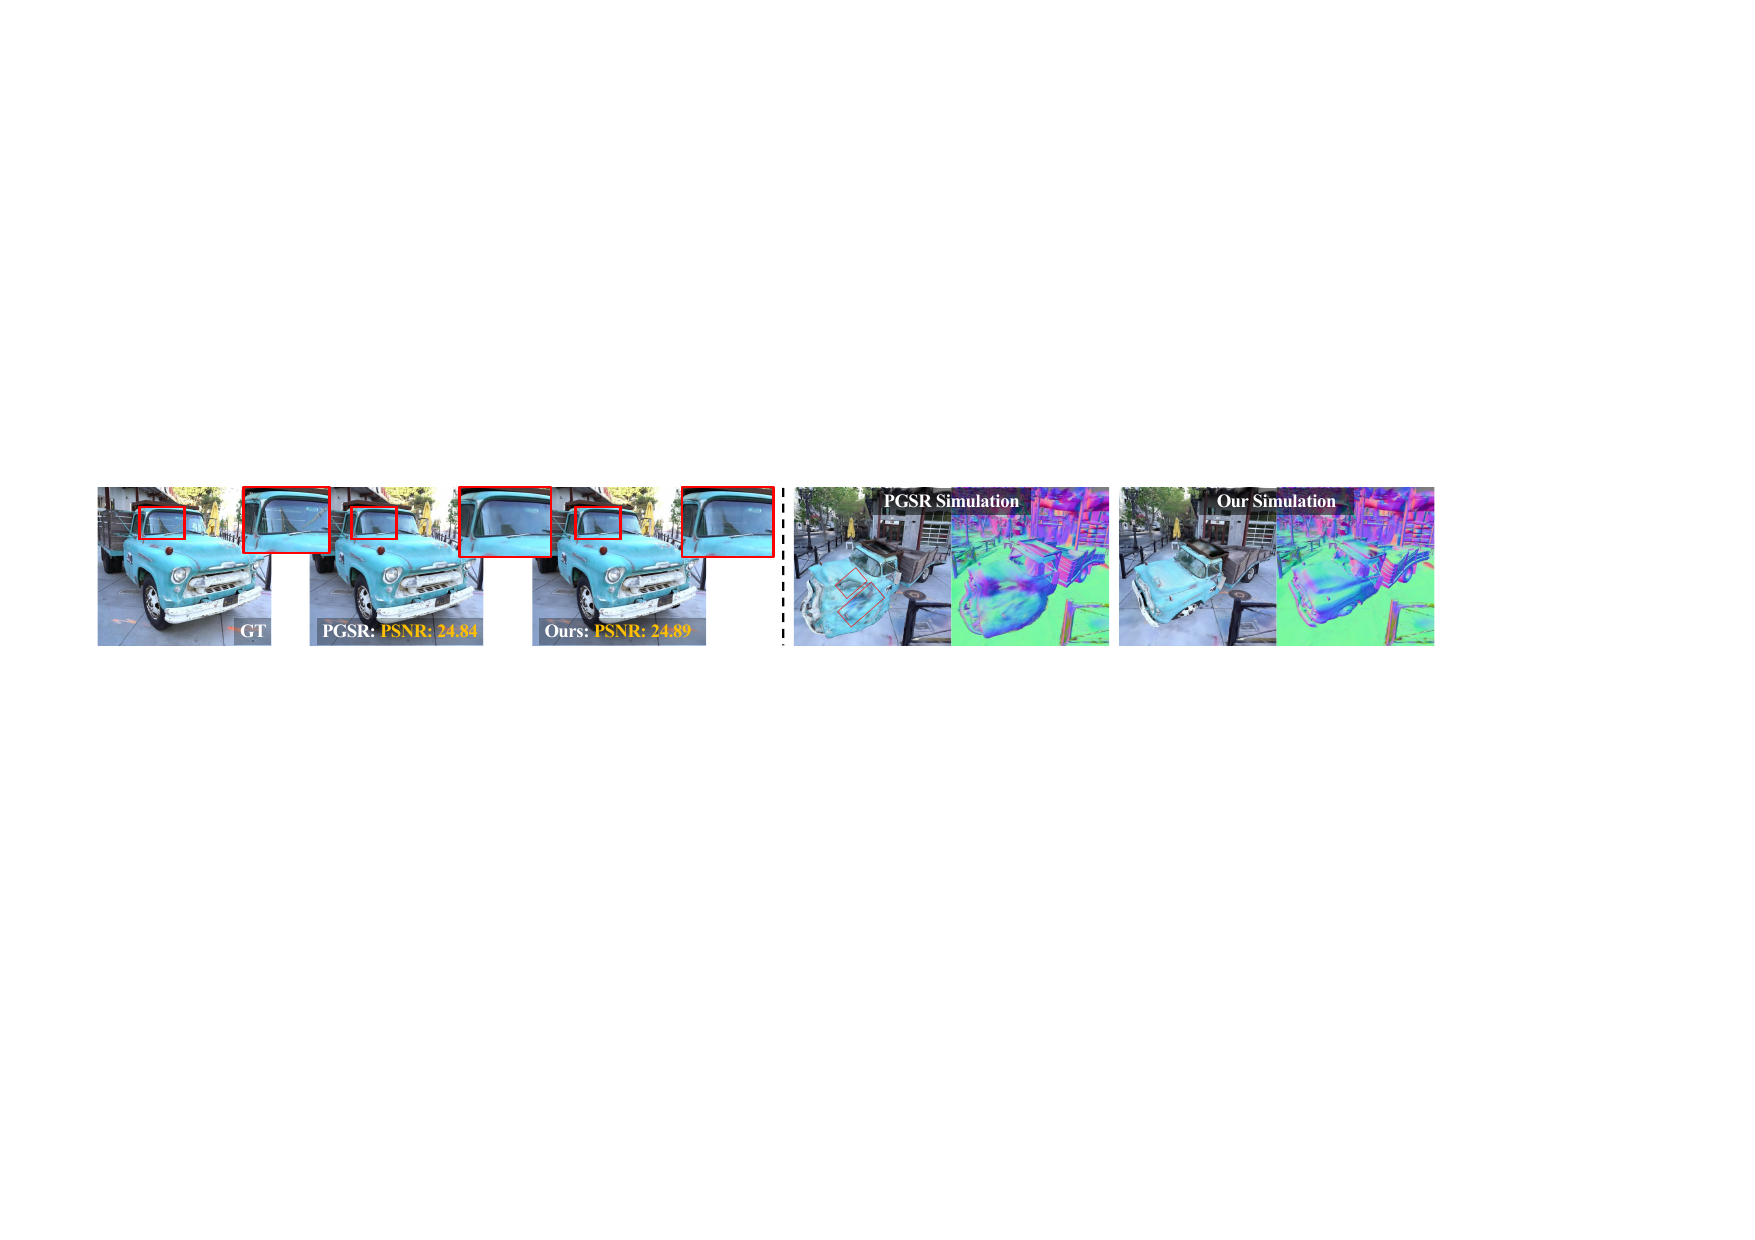}
    % \vspace{-3.5 em}
    \caption{
    We also add real-world finetuning comparisons, where our method adapts GS topology to melting-induced extreme deformations, while maintaining comparable rendering quality. 
    }
\end{figure}
