# Supplementary material for: MeGAS: Thermomechanical Dynamic Gaussian Splatting for Thermophysical Scene Editing
Source: arXiv:2606.23455 source file (2026-06-22)
Supplement: Supplementary file 3 [file 1_thermal_mpm.tex]

\vspace{-0.5 em}
\section{Details for MPM-LBM Simulator}
\label{supp:mpm_lbm}
\vspace{-0.25 em}

% \begin{table}[h]
\begin{wraptable}{l}{0.55 \textwidth}
  \centering
  \vspace{-2.5 em}
  \caption{
  \textbf{Material and discretization parameters.}
  We use identical physical parameters across all experiments.
  }
  \vspace{1.0 em}
  \resizebox{\linewidth}{!}{
  \begin{tabular}{lcl}
    \hline
    Parameter & Value & Description \\
    \hline
    $E$ & $2.8\times10^{4}$ & Young's modulus \\
    $\nu$ & $0.4$ & Poisson's ratio \\
    $g$ & $1.0$ & Gravity acceleration \\
    $\rho$ & $100.0$ & Density of the solid \\
    $\eta$ & $100.0$ & Viscosity coefficient \\
    $h_{\text{shear}}$ & $1.0$ & Shear ratio for plastic flow \\
    $\sigma_{Y}$ & $1.0$ & Yield threshold \\
    $T_{\text{melt}}$ & $0.7$ & Thermal phase threshold \\
    \hline
    $\Delta t$ & $1.0\times 10^{-4}$ & Time step size \\
    $N_{\text{sub}}$ & $100$ & MPM sub-steps per frame \\
    $N_{\text{grid}}$ & $100^3$ & Grid resolution \\
    \hline
  \end{tabular}
  }
  
  \label{tab:mpm_params}
  \vspace{-2.0 em}
% \end{table}

\end{wraptable}

% 我们在此给出Thermal-Driven Material Point Method的完整过程，包括LBM的Heat advection-diffusion Update以及MPM的详细设置
We employ a hybrid particle-grid discretization for the MPM solver and the Lattice Boltzmann solver for the thermal advection-diffusion field. The MPM background grid and the LBM thermal lattice share the same Cartesian layout and spacing $\Delta$x, which allows all operations to be carried out on a common grid without any additional interpolation.

At the particle level (index $p$), we store the position $\mathbf{x}_p$, velocity $\mathbf{v}_p$, mass $m_p$, volume $V_p^0$, elastic deformation gradient $\mathbf{F}_p^{E}$, affine momentum matrix $\mathbf{C}_p$, temperature $T_p$ and its gradient $\nabla T_p$, and a phase flag indicating whether the material is solid or melted.
Grid / lattice nodes (index $i$) store  
mass $m_i$, velocity $\mathbf{v}_i$, and temperature $T_i$.  
For the LBM solver, each lattice node additionally stores the scalar distribution functions $g_{i,k}$ associated with discrete velocities $\mathbf{c}_k$ and weights $w_k$.
Cubic B-spline basis functions are used to define the particle-to-grid and grid-to-particle transfer weights $w_{ip}$ and their gradients $\nabla w_{ip}$.
A single time step from $t^n$ to $t^{n+1}=t^n+\Delta t$ consists of particle-to-grid transfer (P2G), grid update, and grid-to-particle transfer (G2P). The explicit algorithm is outlined as follows.

\noindent\textbf{Particle-to-Grid Transfer.}
We first reset all grid quantities to zero, then accumulate particle mass and momentum via APIC~\cite{jiang2015affine}:
\vspace{-0.5 em}
\begin{equation}
\vspace{-0.25 em}
\begin{aligned}
    m_i^{\,n} &= \sum_p w_{ip}^{\,n} m_p, \\
    \vspace{-1.0 em}
    m_i^{\,n} \mathbf{v}_i^{\,n}
    &= \sum_p w_{ip}^{\,n} m_p
    \left( \mathbf{v}_p^{\,n}
    + \mathbf{C}_p^{\,n} (\mathbf{x}_i - \mathbf{x}_p^{\,n}) \right).
\end{aligned}
\vspace{-0.25 em}
\end{equation}

\noindent For the thermal field we transfer a mass-weighted nodal temperature and its gradient:
\begin{equation}
    m_i^{\,n} T_i^{\,n}
    = \sum_p w_{ip}^{\,n} m_p \left( T_p^{\,n}
    + (\mathbf{x}_i - \mathbf{x}_p^{\,n})^\top \nabla T_p^{\,n} \right).
    \vspace{-0.5 em}
\end{equation}

After the accumulation, grid velocities and temperatures are normalised by mass for nodes with $m_i^{\,n} > 0$
\[
    T_i^{\,n} \leftarrow (m_i^{\,n} T_i^{\,n}) / m_i^{\,n},
    \;
    v_i^{\,n} \leftarrow (m_i^{\,n} v_i^{\,n}) / m_i^{\,n}.
\]

\noindent\textbf{Grid Update.}
Mechanical grid velocities are updated under internal and external forces:
\begin{equation}
    \mathbf{v}_i^{\,n+1}
    = \mathbf{v}_i^{\,n}
    - \frac{\Delta t}{m_i^{\,n}}
      \sum_p \boldsymbol{\tau}_p^{\,n} \nabla w_{ip}^{\,n} V_p^0
    + \Delta t\, \mathbf{g},
\end{equation}
where $\boldsymbol{\tau}_p^{\,n}$ is the Kirchhoff stress computed from the elastic deformation gradient
$\mathbf{F}_p^{E,n}$ and the current constitutive model (solid or melted), and $\mathbf{g}$ is the gravity ( or other external forces).

Thermal boundary conditions are applied to grid nodes associated with user-specified heat sources by constraining their temperatures to the prescribed source values, $T_i^{\,n} = T_{\text{source}}$.
In practice, $T_{\text{source}}$ is implemented as a Neumann-type heating condition, which incrementally increases the boundary temperature according to the imposed heat flux.

The grid temperatures at time $t^{n+1}$ are then updated by performing one step of the LBM solver, denoted by \texttt{LBM\_Update}.

\noindent\textbf{Thermal Advection-Diffusion Solver.}
The temperature field on the grid is advanced with a Lattice Boltzmann solver for the advection-diffusion equation (ADE):
\begin{equation}
\frac{\partial T}{\partial t}
+ \mathbf{u} \cdot \nabla T
= \alpha \nabla^2 T + S,
\end{equation}
where $\mathbf{u}$ is an advection velocity, $\alpha$ is the thermal diffusivity, and $S$ is a volumetric heat source.
In our pure diffusion experiments we simply set $\mathbf{u}=\mathbf{0}$, but the formulation also supports a fully
coupled Navier-Stokes LBM, in which case $\mathbf{u}$ is taken from the fluid velocity field described below.

We employ a standard single-relaxation-time (BGK) advection-diffusion LBM.
At each lattice node and direction $k$, the scalar populations $g_{i,k}$ evolve as:
\vspace{-0.75 em}
\begin{equation}
\label{eq:lbm_T_update}
% \begin{aligned}
g_{i,k}(\mathbf{x} + \mathbf{c}_k \Delta t,\; t + \Delta t)
= g_{i,k}(\mathbf{x}, t)
- \frac{\Delta t}{\tau_T} \left( g_{i,k} - g^{\text{eq}}_{i,k} \right) 
+ \Delta t\, Q_{i,k},
% \end{aligned}
\end{equation}
where $\tau_T$ is the thermal relaxation time.
The macroscopic temperature and discretized source term are recovered from the moments:
\begin{equation}
T_i = \sum_k g_{i,k}, 
\qquad
q_i = \sum_k Q_{i,k}.
\end{equation}

The equilibrium distribution is chosen analogously to the standard LB fluid equilibrium,
but with a single conserved scalar:
\begin{equation}
g^{\text{eq}}_{i,k} = w_k T_i 
\left[
1 
+ \frac{\mathbf{c}_k \cdot \mathbf{u}_i}{c_s^2}
+ \frac{(\mathbf{c}_k \cdot \mathbf{u}_i)^2}{2 c_s^4}
- \frac{\mathbf{u}_i \cdot \mathbf{u}_i}{2 c_s^2}
\right],
\end{equation}
where $c_s$ is the lattice sound speed and $\mathbf{u}_i$ is the prescribed advection velocity at node $i$
(for pure diffusion we set $\mathbf{u}_i = \mathbf{0}$).
The source term is discretized as:
\begin{equation}
Q_{i,k} = w_k\, q_i 
\left( 
1 - \frac{\Delta t}{2 \tau_T}
\right).
\end{equation}
A Chapman-Enskog expansion shows that this scheme recovers the ADE with thermal diffusivity:
\begin{equation}
\alpha = c_s^2 \left( \tau_T - \frac{\Delta t}{2} \right).
\end{equation}

If fluid motion is to be resolved, we augment the above temperature solver with an isothermal LBM for the (weakly compressible) Navier-Stokes equations:
\vspace{-1.0 em}
\begin{equation}
\partial_t (\rho \mathbf{u}) + \nabla \cdot (\rho \mathbf{u} \mathbf{u})
= -\nabla p + \nabla \cdot (2 \rho \nu \mathbf{D}) + \rho \mathbf{g} + \mathbf{F}_{\text{ext}},
\end{equation}
where $\rho$ is the density, $\nu$ is the kinematic viscosity, $\mathbf{D}$ is the rate-of-strain tensor, and $\mathbf{F}_{\text{ext}}$ collects body forces (e.g.\ buoyancy).

We introduce an additional set of distribution functions $f_{i,k}$ living on the same lattice with velocities $\mathbf{c}_k$ and weights $w_k$. Their evolution is given by:
\begin{equation}
\label{eq:lbm_f_update}
% \begin{aligned}
f_{i,k}(\mathbf{x} + \mathbf{c}_k \Delta t,\; t + \Delta t)=
f_{i,k}(\mathbf{x}, t)
- \frac{\Delta t}{\tau_f} \left( f_{i,k} - f^{\text{eq}}_{i,k} \right) 
+ \Delta t\, F_{i,k},
%\end{aligned}
\end{equation}
where $\tau_f$ is the fluid relaxation time and $F_{i,k}$ is a forcing term.
The macroscopic density and velocity are recovered as:
\begin{equation}
\rho_i = \sum_k f_{i,k}, 
\qquad
\rho_i \mathbf{u}_i = \sum_k \mathbf{c}_k f_{i,k}
+ \frac{\Delta t}{2}\, \mathbf{F}_i,
\end{equation}
with $\mathbf{F}_i$ the total body force at node $i$.
The equilibrium distribution is the standard second-order isothermal form:
\begin{equation}
f^{\text{eq}}_{i,k} = w_k \rho_i 
\left[
1 
+ \frac{\mathbf{c}_k \cdot \mathbf{u}_i}{c_s^2}
+ \frac{(\mathbf{c}_k \cdot \mathbf{u}_i)^2}{2 c_s^4}
- \frac{\mathbf{u}_i \cdot \mathbf{u}_i}{2 c_s^2}
\right].
\end{equation}
Under this choice, a Chapman-Enskog analysis shows that the LB scheme recovers the Navier-Stokes equations in the low-Mach-number limit, with kinematic viscosity:
\begin{equation}
\nu = c_s^2 \left( \tau_f - \frac{\Delta t}{2} \right).
\end{equation}

\noindent Body forces are incorporated via a standard Guo-type forcing term:
\begin{equation}
F_{i,k} = w_k
\left[
\frac{\mathbf{c}_k - \mathbf{u}_i}{c_s^2}
+ \frac{(\mathbf{c}_k \cdot \mathbf{u}_i)}{c_s^4}\,\mathbf{c}_k
\right]\!\cdot\! \mathbf{F}_i.
\end{equation}

For thermally driven flows, we use a Boussinesq approximation and define:
\begin{equation}
\mathbf{F}_i
= \rho_0 \beta \left( T_i - T_{\text{ref}} \right) \mathbf{g}
+ \mathbf{F}_{\text{other}},
\end{equation}
where $\rho_0$ is a reference density, $\beta$ is the thermal expansion coefficient, $T_{\text{ref}}$ is a reference temperature, and $\mathbf{F}_{\text{other}}$ collects any additional body forces.
The buoyancy term couples the temperature LBM and the Navier-Stokes LBM: the temperature field $T_i$ feeds into the body force $\mathbf{F}_i$, while the fluid velocity $\mathbf{u}_i$ is used as the advection velocity in the thermal equilibrium $g^{\text{eq}}_{i,k}$ in Eq.~\eqref{eq:lbm_T_update}.
In the special case where fluid motion is neglected, we simply disable the Navier-Stokes solver and set $\mathbf{u}_i=\mathbf{0}$ everywhere, resulting in a purely diffusive temperature evolution.

\noindent\textbf{Grid-to-Particle Transfer and Constitutive Update.}
After the grid velocities and temperatures have been advanced, we interpolate them back to particles:
\vspace{-0.25 em}
\begin{equation}
\mathbf{v}_p^{n+1} = \sum_i w_{ip}^n\, \mathbf{v}_i^{n+1},
\vspace{-0.25 em}
\end{equation}
\vspace{-0.25 em}
\begin{equation}
\nabla \mathbf{v}_p^{n+1} = \sum_i \mathbf{v}_i^{n+1} 
(\nabla w_{ip}^n)^{\!\top}
\vspace{-0.25 em}
\end{equation}

\vspace{-0.75 em}
\begin{equation}
\mathbf{x}_p^{n+1} = \mathbf{x}_p^{n} + \Delta t\, \mathbf{v}_p^{n+1},
\vspace{-0.5 em}
\end{equation}
\vspace{-0.25 em}
\begin{equation}
\mathbf{C}_p^{n+1} 
= \frac{4}{\Delta x^2} \sum_i w_{ip}^n\, \mathbf{v}_i^{n+1} 
(\mathbf{x}_i - \mathbf{x}_p^{n})^{\!\top},
\vspace{-0.25 em}
\end{equation}
\vspace{-0.25 em}
\begin{equation}
T_p^{n+1} = \sum_i w_{ip}^n\, T_i^{n+1},
\vspace{-0.25 em}
\end{equation}
\vspace{-0.25 em}
\begin{equation}
\nabla T_p^{n+1} = \sum_i T_i^{n+1} \left(\nabla w_{ip}^n\right)^{\!\top}.
\vspace{-0.25 em}
\end{equation}

\noindent The elastic deformation gradient is updated as:
\begin{equation}
\mathbf{F}_{p}^{E,n+1}
= \left(\mathbf{I} + \Delta t\, \nabla \mathbf{v}_p^{n+1}\right)
\mathbf{F}_p^{E,n}.
\end{equation}

Finally, we perform \textbf{temperature-driven phase switching}: 
if the particle temperature exceeds the melting threshold $\tau_{\text{melt}}$, we switch its constitutive model from solid to melted state, 
i.e.\ from StVK elasticity~\cite{klar2016drucker} to a Herschel-Bulkley viscoplastic model~\cite{yue2015continuum}; 
otherwise we keep the solid model:
\begin{equation}
(\tau_p^{n+1},\, \mathbf{F}_{p}^{E,n+1}) 
=
\begin{cases}
\text{solidModel}\!\left(\mathbf{F}_{p}^{E,n+1}\right),
\;\;\; T_p^{n+1} \le T_{\text{melt}}, \\[5pt]
\text{meltedModel}\!\left(\mathbf{F}_{p}^{E,n+1}\right),
T_p^{n+1} > T_{\text{melt}}.
\end{cases}
\end{equation}

For the StVK elasticity model, we define the Kirchhoff stress $\tau$ as:
\begin{equation}
\boldsymbol{\tau}
= \mathbf{U}\bigl( 2\mu\boldsymbol{\epsilon}
+ \lambda\mathrm{tr}(\boldsymbol{\epsilon})\mathbf{I} \bigr)\mathbf{V}^T ,
\end{equation}
where 
$\mathbf{F}^E = \mathbf{U}\, \boldsymbol{\Sigma}\, \mathbf{V}^{\!\top}$ is the SVD decomposition of $\mathbf{F}$ 
and 
$\boldsymbol{\epsilon} = \log(\boldsymbol{\Sigma})$ denotes the Hencky strain. Here $\mu$ and $\lambda$ are the Lamé parameters.

\iffalse
\begin{figure}[t] % 使用 !t 尝试强制图像置顶
    \centering
    \scriptsize
    \includegraphics[width=\linewidth]{figures/supp/diffusion_process.pdf}
    \vspace{-2.0 em}
    \caption{
    \textbf{Heat diffusion with constitutive modeling switching.}
    We first present visualizations of pure heat diffusion, where the temperature field gradually propagates from high to low values over time.
    By incorporating phase-change-controlled constitutive model switching, we present melting behavior that is explicitly driven by the evolving temperature field.
    Moreover, we show that different configurations of heat sources give rise to distinct melting patterns and effects.
    }
    \label{fig:supp:diffusion_process}
    \vspace{-2.0 em}
\end{figure}
\fi

For the Herschel-Bulkley viscoplastic model, we first compute the deviatoric part of the trial Kirchhoff stress:
\begin{equation}
\mathbf{s}_{n+1}^{\mathrm{pre}}
= \mu\, \mathrm{dev}\!\left[\tau_{n+1}\right],
\qquad
s_{n+1}^{\mathrm{pre}}
= \left\| \mathbf{s}_{n+1}^{\mathrm{pre}} \right\|_{F},
\end{equation}
where $\mathrm{dev}(\cdot)$ denotes the deviatoric part and 
$\|\cdot\|_{F}$ the Frobenius norm. 
If the von Mises equivalent stress satisfies:
\begin{equation}
s_{n+1}^{\mathrm{pre}}
- \sqrt{\frac{2}{3}}\, \sigma_Y \le 0,
% \vspace{-1.0 em}
\end{equation}
with $\sigma_Y$ the yield stress, the response remains elastic and the trial state is accepted.
Otherwise, plastic flow is activated and we perform a semi-implicit return-mapping step.
Define $\tilde{\mu}=\frac{\mu}{3}\;\mathrm{Tr}(\Sigma^2)$, we update the $s_{n+1}$ explicitly as:
\begin{equation}
\eta^{1/h}\left(s_{n+1} - s_{n+1}^{\mathrm{pre}}\right)
+ 2\tilde{\mu}\,\Delta t
\left(
s_{n+1} - \sqrt{\frac{2}{3}}\, \sigma_Y
\right)^{1/h}
= 0,
\end{equation}
where $\eta$ is the viscosity parameter and $h$ is the shear rate. We obtain $s_{n+1}$ via bisection.
The deviatoric stress is then projected back onto the yield surface as:
\begin{equation}
\hat{\mathbf{s}}_{n+1}
= 
\frac{s_{n+1}}{s_{n+1}^{\,\mathrm{pre}}}\,
\mathbf{s}_{n+1}^{\,\mathrm{pre}} ,
\end{equation}
and we update the Kirchhoff stress with $\hat{\mathbf{s}}_{n+1}$ as:
\begin{equation}
\boldsymbol{\tau} = \mathbf{U}\,
\exp\!\left(
\frac{\hat{s}}{2\mu}\, \mathrm{dev}\!\left[\boldsymbol{\epsilon}\right]
+ \frac{1}{3}\, \mathrm{Tr}(\boldsymbol{\epsilon})\, \mathbf{I}
\right)
\mathbf{V}^{T}.
\end{equation}

% As shown in Fig.~\ref{fig:supp:diffusion_process}, we illustrate the process of heat diffusion alone, as well as the constitutive model switching governed by phase-change control.
