# Supplementary material for: MeGAS: Thermomechanical Dynamic Gaussian Splatting for Thermophysical Scene Editing
Source: arXiv:2606.23455 source file (2026-06-22)
Supplement: Supplementary file 4 [file 3_imls_refine.tex]

\vspace{-1.0 em}
\section{Details for Densification with Implicit Surface Guidance}
\label{supp:imls_densify}
\vspace{-0.5 em}
We provide the full formulation and implementation details for the implicit-surface-guided adaptive densification (Sec.~\textcolor{red}{4.2.2}).

Define $\mathcal{G}_s = \left\{
G_i^{s} = 
\left( 
\mathbf{x}_i^{s},\,
\mathbf{R}_i^{s},\,
\mathbf{S}_i^{s},\,
\mathbf{o}_i^{s},\,
\mathbf{c}_i^{s}
\right)
\right\}
$ the Gaussians that lie on the reconstructed object surface in the rest state, and $\Phi_{t}(\cdot)$ is the deformation mapping at time step $t$ obtained from the MPM simulation.
After deformation, we obtain the deformed surface Gaussians:
\begin{equation}
\tilde{\mathcal{G}}_s^{\,t}
=
\Phi_{t}(\mathcal{G}_s)
=
\left\{
\tilde{G}_i^{s}
=
\left(
\tilde{\mathbf{x}}_i^{s},\,
\tilde{\mathbf{R}}_i^{s},\,
\tilde{\mathbf{S}}_i^{s},\,
\tilde{\mathbf{o}}_i^{s},\,
\tilde{\mathbf{c}}_i^{s}
\right)
\right\},
\end{equation}
and associate to each $\tilde{G}_i^{s}$ a surface normal $\tilde{\mathbf{n}}_i^{\,s}$
given by the shortest axis of $\tilde{\mathbf{S}}_i^{s}$.

% 此时我们有一组surfel-like的表面gaussian，以及内部填充的particle，我们希望用表面gaussian引导内部填充的particle去填补由于extreme deformation导致的表面开裂。我们希望填补的是原始表面gaussian存在空隙的区域，用于填补的对象是刚好填充这些空隙区域的internal particle，因此我们首要的第一步是通过surface detection来筛选出哪些internal particle可以被用来填充表面。我们在物体360度周围按照elevation 25度interval，azimuths 45度interval设置虚拟相机，并将internal particles初始化为isotropic Gaussian Splats with opacity=1。我们遍历virtual cameras，并记录光栅化过程中各个像素对应的gaussian splat with maximal alpha contribution along the ray, 从而筛选出用于填充表面的internal particles. 如图Fig.x所示，我们的方法在形变过程中有效的筛选出了正确的surface particles.

\begin{wrapfigure}[13]{r}{0.5\textwidth}
%\begin{figure}[t] % 使用 !t 尝试强制图像置顶
    \vspace{-1.75 em}
    \centering
    \scriptsize
    \includegraphics[width=\linewidth]{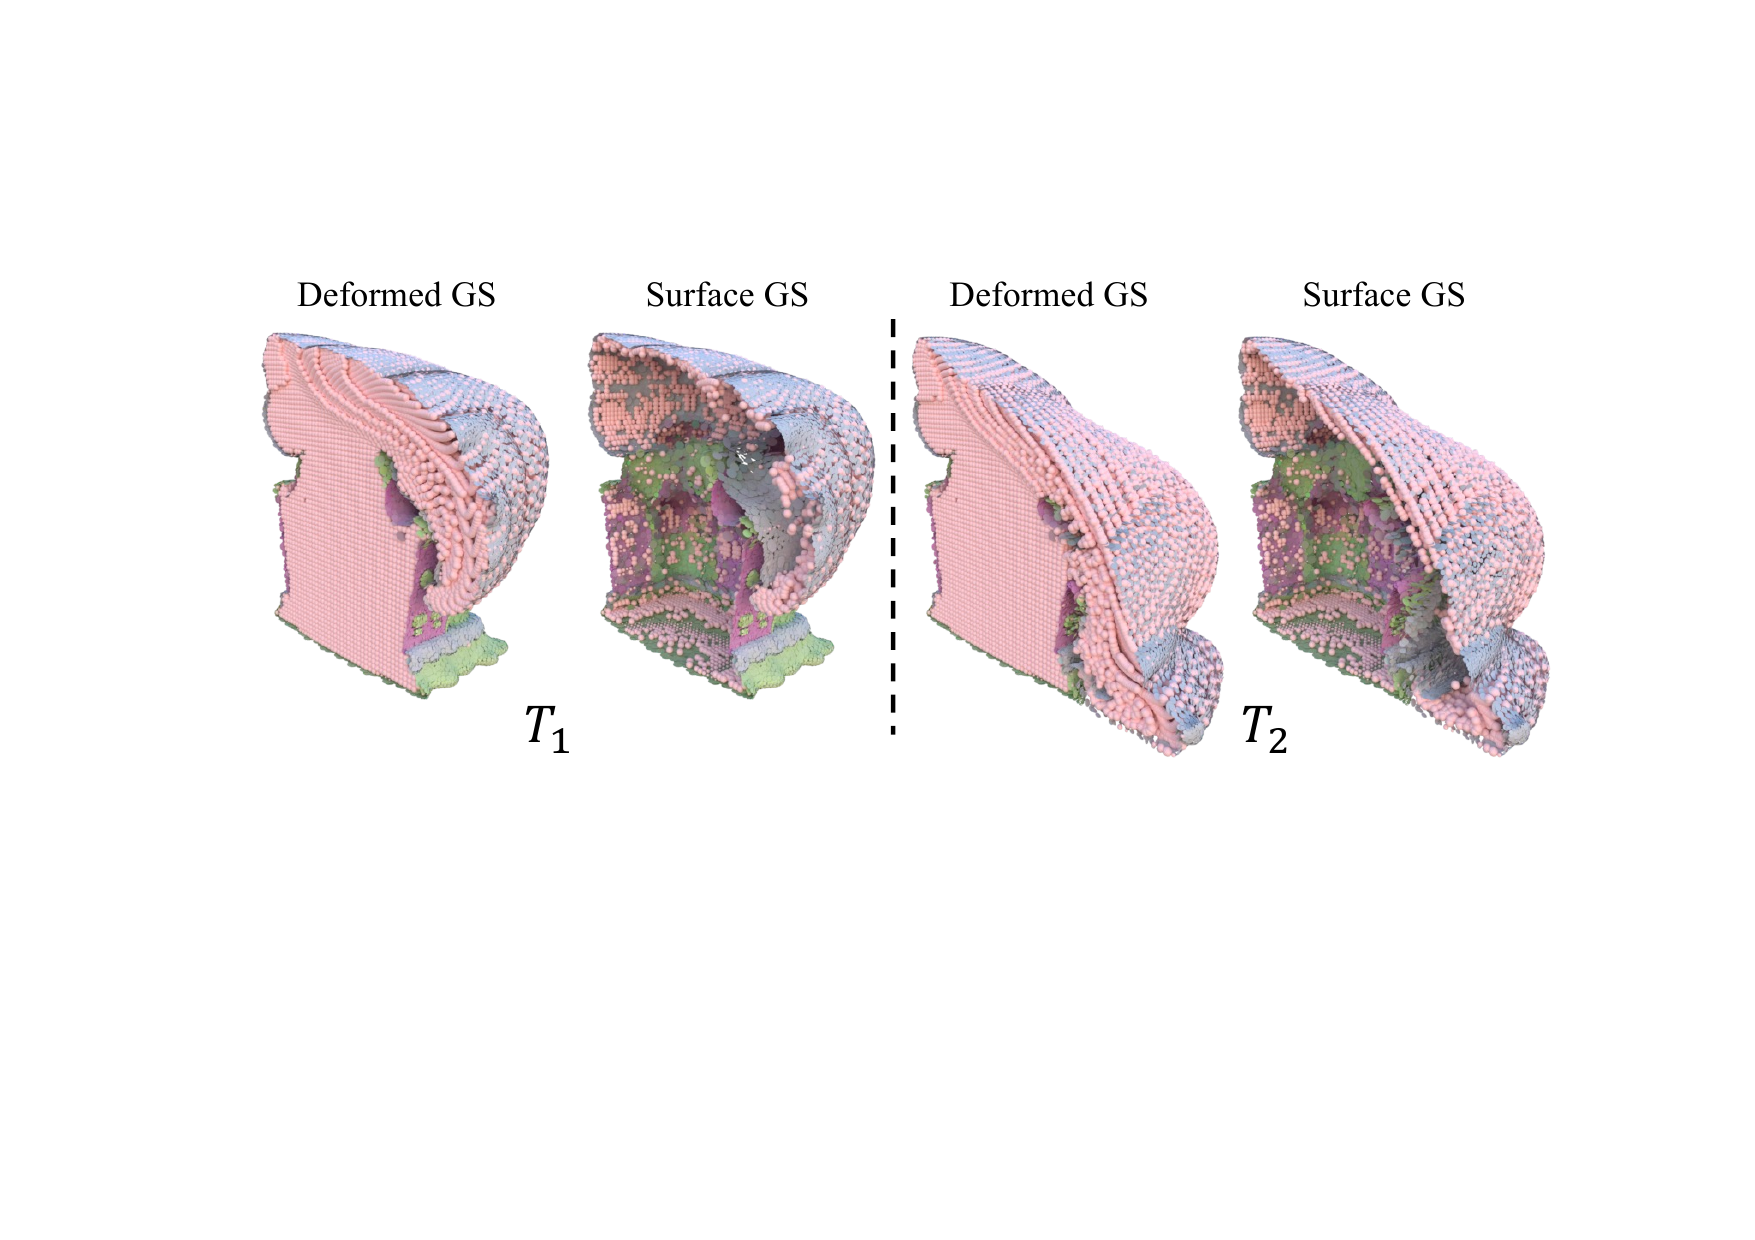}
    \vspace{-1.0 em}
    \caption{
    \textbf{Surface detection.}
    Our surface detection effectively filters the subset of internal particles, which are treated as candidates to be converted into new surface Gaussians for crack sealing.
    The internal particles are highlighted in pink for visualization. 
    }
    \label{fig:supp:surface_detection}
    \vspace{-2.0 em}
% \end{figure}
\end{wrapfigure}

\noindent\textbf{Surface Detection.}
At each rendering step, we maintain two sets of primitives: 
(i) a set of surfel-like surface Gaussians $\tilde{\mathcal{G}}_s^{\,t}$, and
(ii) a set of volumetric internal particles produced by the ray-tracing-based filling scheme.
Under extreme deformations, the surface Gaussians separate and expose cracks in the reconstructed surface, thus our goal is to reuse internal particles that lie close to the visible boundary to fill these newly exposed gaps.
% fill exactly these gaps. 
To this end, we first perform a surface detection that identifies which internal particles can be regarded as surface samples and are thus eligible for subsequent densification.

We distribute a set of virtual cameras on an object-centric viewing sphere to estimate visibility under deformation.
We sample camera azimuths every $45^{\circ}$ and elevations every $25^{\circ}$, covering the full $360^{\circ}$ around the object.
Internal particles $\mathbf{p}_j^t$ are initialized as isotropic Gaussian splats $G_j^p$ with opacity $\mathbf{o}_j=1$ and radius $r_j$:
\begin{equation}
r_j=\kappa\,\min\!\left\{\,\min_i\|\mathbf{p}_j^t-\mathbf{x}_i^s\|,\;\min_{k\neq j}\|\mathbf{p}_j^t-\mathbf{p}_k^t\|\,\right\},
\end{equation}
where $\kappa\in(0,1)$ is a shrinkage ratio, we set $\kappa=0.5$. 

We traverse the virtual cameras, rasterize the Gaussian splats $\{G_p,\; G_s\}$, and record the splat $G_i$ with maximal alpha contribution along the ray for each pixel.
The union of these front-most splats over all views yields the set of visible internal particles, which we treat as candidates to be converted into new surface Gaussians for crack sealing.
As shown in Fig.~\ref{fig:supp:surface_detection}, our surface detection strategy reliably tracks the evolving surface throughout large deformations.

\noindent\textbf{Implicit Surface from Deformed Gaussians.}
Given the deformed surface Gaussians $\tilde{\mathcal{G}}_s^{\,t}$, we follow the implicit moving least squares (IMLS) formulation for point set surfaces~\cite{alexa2001point,kolluri2008provably,oztireli2009feature} and define an implicit function:
\begin{equation}
f(\mathbf{x})
=
\frac{
\sum_i G_i^s (\mathbf{x})\,
(\tilde{\mathbf{n}}_{i}^{s})^{\!\top}
(\mathbf{x}-\tilde{\mathbf{x}}_{i}^{s})
}{
\sum_i G_i^s (\mathbf{x})
}.
\end{equation}
The zero level set $\mathcal{S}_{\text{IMLS}}=\{\mathbf{x} \mid f(\mathbf{x}) = 0\}$ 
defines an approximation of the deformed surface.
For the spatial weighting kernel, we directly reuse the Gaussian kernel associated with each splat $G_i^s$:
\begin{equation}
G_i^s(\mathbf{x})
=
\begin{cases}
\displaystyle
e^{\!-\frac{1}{2}(\mathbf{x}-\mathbf{x}_i^s)^{\top}\boldsymbol{\Sigma}^{-1}(\mathbf{x}-\mathbf{x}_i^s)}, & \|\mathbf{x}-\mathbf{x}_i^s\|_2 < h, \\[6pt]
0, & \|\mathbf{x}-\mathbf{x}_i^s\|_2 \ge h,
\end{cases}
\end{equation}
where $\boldsymbol{\Sigma}$ denotes the covariance of the Gaussian and $h$ is an adaptive influence radius.
For a query point $\mathbf{x}$, we estimate $h$ from the local density of Gaussians as
$h(\mathbf{x}) = \eta\, \bar{d}(\mathbf{x})$, 
where $\bar{d}(\mathbf{x})$ is the average distance to the $k$ nearest surface
Gaussians in $\tilde{\mathcal{G}}_{s}^{\,t}$ (we use $k=32$) and 
$\eta$ is a constant scaling factor (we use $\eta=1.5$).

We then project each candidate internal particle $\mathbf{p}_j^{\,t}$, detected by the surface selection stage described above, onto the implicit surface $\mathcal{S}_{\text{IMLS}}$.
Let $\mathbf{x}_j^{(0)} = \mathbf{p}_j^{\,t}$ be the initialization.
We perform a small, fixed number $L$ of Newton-style iterations:

\begin{enumerate}
\vspace{-1.0 em}
\item Evaluate $f(\mathbf{x}_j^{(\ell)})$.

\item Approximate the gradient of $f$ at $\mathbf{x}_j^{(\ell)}$ by a locally weighted average of normals:
\begin{equation}
\nabla f(\mathbf{x}_j^{(\ell)})
    \approx
    \frac{
        \sum_{i} G_i^s(\mathbf{x}_j^{(\ell)})\, \tilde{\mathbf{n}}_i^{\,s}
    }{
        \sum_{i} G_i^s(\mathbf{x}_j^{(\ell)})
    }.
\end{equation}

\item Normalize the gradient to obtain the local surface normal:
\begin{equation}
\mathbf{n}_j^{(\ell)}
=
\frac{
    \nabla f(\mathbf{x}_j^{(\ell)})
}{
    \bigl\lVert \nabla f(\mathbf{x}_j^{(\ell)}) \bigr\rVert
}.
\end{equation}

\item Update the position along the normal direction:
\begin{equation}
\mathbf{x}_j^{(\ell+1)}
=
\mathbf{x}_j^{(\ell)}
-
\, f(\mathbf{x}_j^{(\ell)})\, \mathbf{n}_j^{(\ell)}.
\end{equation}
\end{enumerate}

We terminate the iterations if $\lvert f(\mathbf{x}_j^{(\ell)}) \rvert < \varepsilon$
(we use $\varepsilon = 10^{-5}$)
or when $\ell$ reaches $L_{\max}$ (we use $L_{\max} = 5$).
The final projected position and normal are denoted by $\mathbf{x}_j^{\star}$ and $\mathbf{n}_j$, respectively.

\noindent\textbf{Gaussian Kernel Refitting.}
Given $(\mathbf{x}_j^{\star}, \mathbf{n}_j, r_j)$, we assign a new Gaussian kernel
$G_j^{p}$ to the crack-filling particle:
\begin{itemize}
  % \vspace{-2.0 em}
  \item \textbf{Position.}
  The Gaussian center is set to the projected position,
  $\boldsymbol{\mu}_j = \mathbf{x}_j^{\star}$.

  \item \textbf{Orientation.}
  We construct a rotation matrix $\mathbf{R}_j$ whose normal axis is aligned with the surface normal $\mathbf{n}_j$.
  
  \item \textbf{Scale.}
  We construct the scale matrix to represent an isotropic disk in the tangent plane, i.e.,
  $\mathbf{S}_j = \mathrm{diag}(r_j,\,r_j,\,0)$.

  \item \textbf{Appearance.}
  The appearance parameter $\mathbf{c}_j$ is computed as the average of
  the $K$ nearest surface Gaussians in $\tilde{\mathcal{G}}_{s}^{\,t}$:
  \begin{equation}
  \vspace{-0.5 em}
  \mathbf{c}_j
  = \frac{1}{K}
    \sum_{i \in \mathcal{N}_K(\mathbf{x}_j^{\star})}
    \tilde{\mathbf{c}}_i^{\,s},
  \end{equation}
  where $\mathcal{N}_K(\mathbf{x}_j^{\star})$ denotes the indices of the $K$
  nearest neighbors in position space.

  \item \textbf{Opacity.}
  We initialize the opacity $o_j = 1$.
  % \vspace{-1.0 em}
\end{itemize}

\begin{wrapfigure}[18]{r}{0.5 \textwidth}
% \begin{figure}[!t] % 使用 !t 尝试强制图像置顶
    \vspace{-3.0 em}
    \centering
    \scriptsize
    \includegraphics[width=0.9\linewidth]{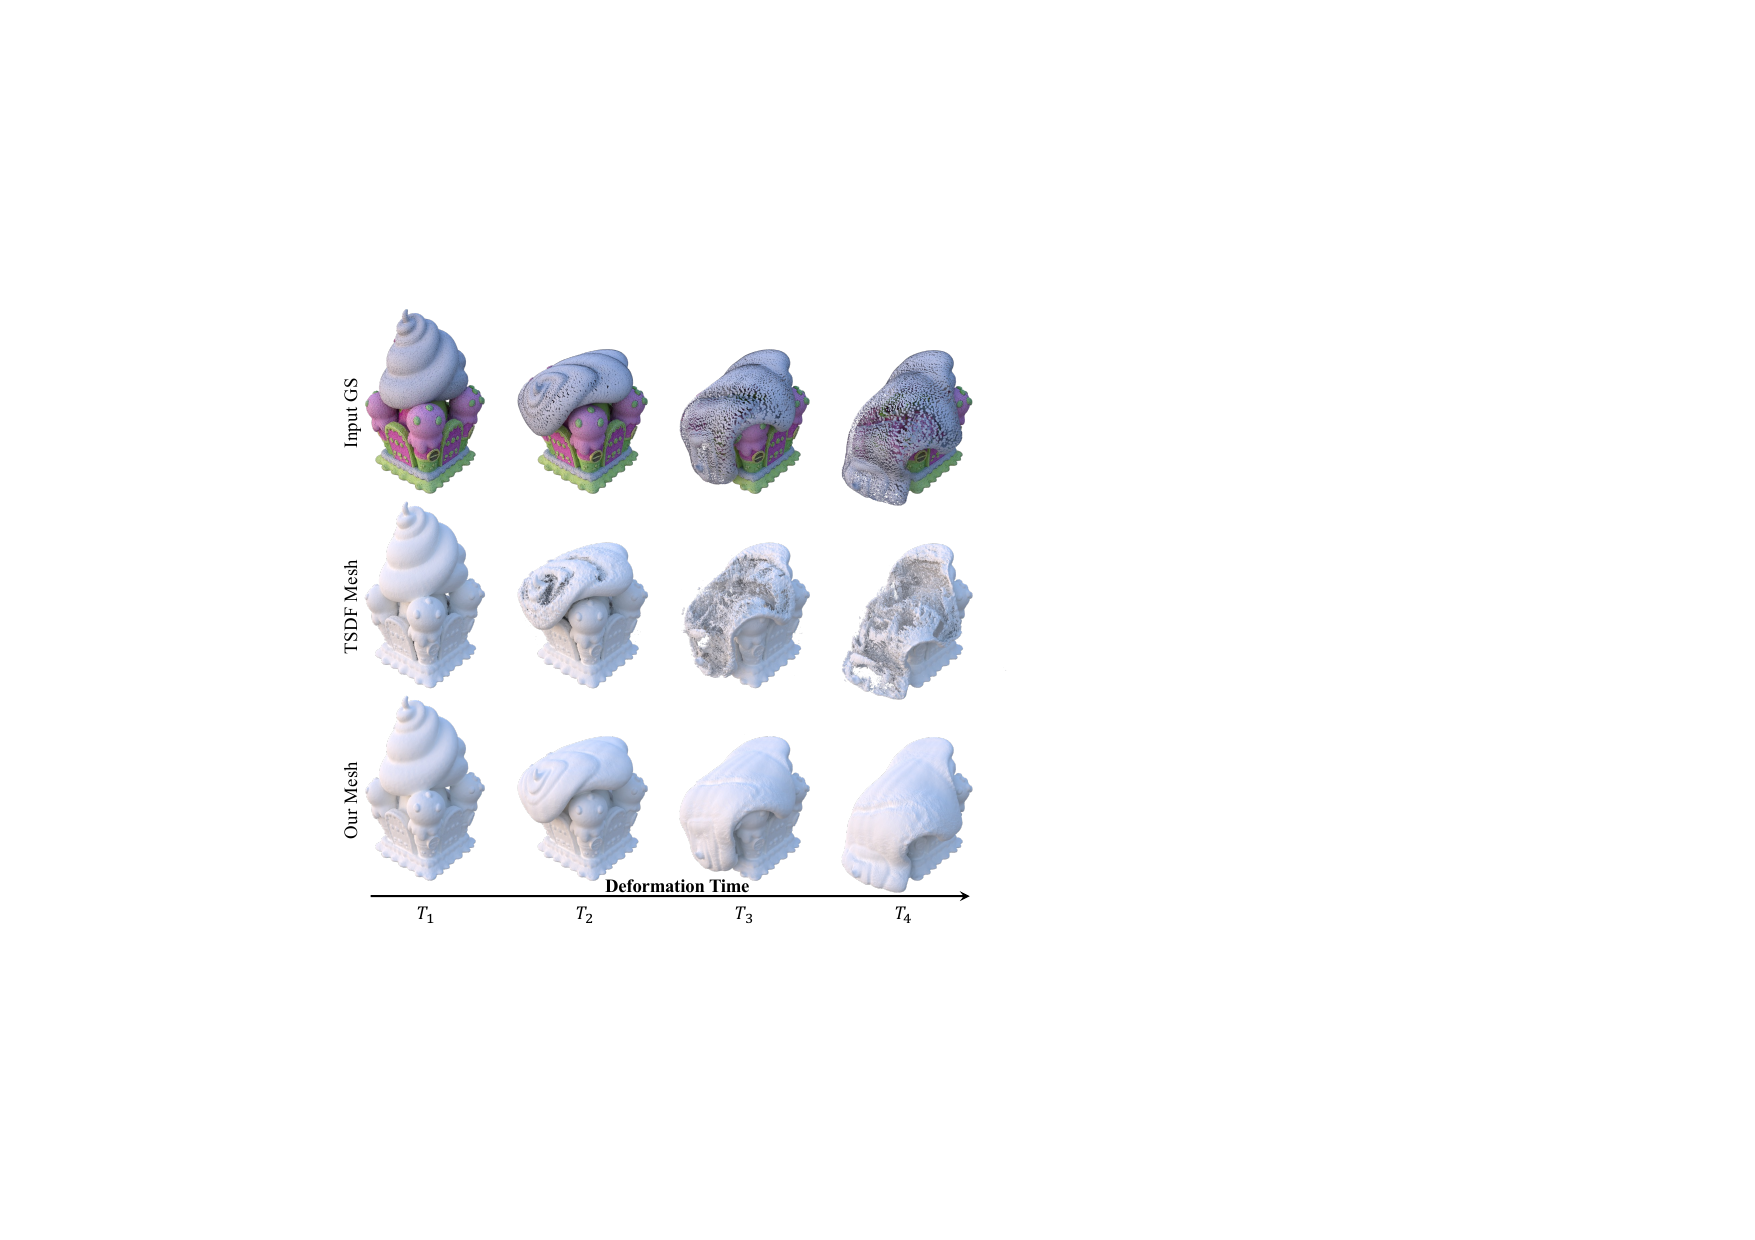}
    % \vspace{-1.0 em}
    \captionsetup{font=footnotesize}
    \caption{
    \textbf{Comparison of our IMLS GS-to-Mesh with TSDF-based baseline.}
    Compared with meshes obtained via TSDFusion, our approach, which combines Gaussian Splatting with IMLS, produces temporally more continuous and smoother surfaces while simultaneously preserving fine geometric details.
    }
    \label{fig:supp:mls_surface}
    % \vspace{-1.0 em}
% \end{figure}
\end{wrapfigure}

The resulting Gaussians $\{G_j^{p}\}$ are finally merged with the existing deformed surface Gaussians to produce the densified representation used for rendering.

We implement the above operation in CUDA, making its computational overhead negligible in practice.
Leveraging the IMLS formulation, we further reinterpret the Gaussian Splatting as a signed distance field and apply the Marching Cubes~\cite{lorensen1998marching} to extract high-quality meshes.
As illustrated in Fig.~\ref{fig:supp:mls_surface}, we compare our IMLS-based GS-to-mesh pipeline with a TSDF-fusion-based~\cite{newcombe2011kinectfusion} GS-to-mesh baseline, and our method consistently preserves finer geometric details.

% \clearpage
% \vspace{1.0 em}
\section{Computational Cost of Each Stage}
\label{supp:computation_cost}
% \vspace{-2.5 em}

\begin{table}[h]
\centering
\setlength{\tabcolsep}{2pt}

\resizebox{\linewidth}{!}{
    \Large
    % \fontsize{13pt}{14pt}\selectfont
    \begin{tabular}{lccccc}
        \toprule
        \textbf{Scene\textbackslash{}Module} 
        & \textbf{\#Splats (+ \#Filling)} 
        & \textbf{Internal Filling }
        & \textbf{MPM + LBM (substep) }
        & \textbf{IMLS Update }
        & \textbf{GS Rendering} \\
        \midrule
        % \multicolumn{6}{l}{\textbf{Synthetic scenes}} \\
        Candy house (\textit{Synthetic})
        & 154k (+103k) & 475 ms / 0.4 GB & 6 ms / 0.6 GB  & 375 ms / 0.9 GB   & 3 ms / 0.9 GB \\
        Lego (\textit{Synthetic})
        & 213k (+13k)  & 231 ms / 0.5 GB & 9 ms / 0.5 GB  & 419 ms / 0.8 GB   & 4 ms / 0.8 GB \\
        Toy bulldozer (\textit{Synthetic})
        & 52k (+47k)   & 206 ms / 0.3 GB & 8 ms / 0.4 GB  & 175 ms / 0.5 GB   & 2.0 ms / 0.5 GB \\
        
        \midrule
        
        % \multicolumn{6}{l}{\textbf{Real scenes}} \\
        Toy Sculpture (\textit{Real})
        & 683k (+70k)  & 662 ms / 1.3 GB & 13 ms / 1.2 GB & 1084 ms / 2.0 GB  & 7 ms / 1.9 GB \\
        Kitchen bulldozer (\textit{Real})
        & 175k (+25k)  & 288 ms / 0.4 GB & 9 ms / 0.5 GB  & 358 ms / 0.7 GB   & 3 ms / 0.8 GB \\
        Truck (\textit{Real})
        & 551k (+21k)  & 441 ms / 1.1 GB & 11 ms / 1.0 GB & 851 ms / 1.6 GB   & 9 ms / 1.5 GB \\
        \bottomrule
    % \vspace{-4.2 em}
    \end{tabular}
}

% \clearpage
\vspace{0.25 em}
\caption{Computational costs.}
% \vspace{-2.5 em}
\end{table}

Under the parameter settings in supp.Tab.~\ref{tab:mpm_params}, we show the
detailed per-scene costs with
runtime and peak GPU memory of each stage on an RTX 4070 
% \clearpage
12GB GPU.
In particular, the \textit{MPM+LBM} and \textit{IMLS update} stages are implemented using our custom Warp~\cite{macklin2022warp} CUDA kernels. The reported costs are measured per invocation of each stage. Note for real-world scenes, we only consider the segmented foreground object as mentioned in section.~\ref{supp:train_3dgs}.

% \begin{table}[h]
% \vspace{-2.0 em}
% \centering
% \large
% \caption{Computational costs.}
% \vspace{-1.0 em}
% \setlength{\tabcolsep}{4pt}
% \renewcommand{\arraystretch}{1.15}
% \resizebox{\linewidth}{!}{
% \begin{tabular}{l c c c c c}
% \specialrule{.1em}{.1em}{.1em}
% \textbf{Module} & \textbf{Internal Filling} & \textbf{MPM+LBM (substep)} & \textbf{IMLS Update} & \textbf{GS Rendering} & \textbf{GS Training} \\
% \textbf{Cost (Time/GPU)} & 200\,ms / 0.25\,GB & 10\,ms / 0.3\,GB & 150\,ms / 0.4\,GB & 2\,ms / 0.5\,GB & 5\,min / 2\,GB (30k steps) \\
% % \hline
% \specialrule{.1em}{.1em}{.1em}
% % \vspace{-4.5 em}
% \end{tabular}
% }
% \vspace{-2.0 em}
    
% \end{table}

\vspace{-1.0 em}
\section{Generalization of Topology-Adaptive Rendering}
\label{supp:general_topology_render}
\vspace{-0.25 em}
% 我们提出的Topology-Adaptive Gaussian Rendering make gaussian splats robuts and yield smoother geometry, 并且可以自然的泛化到其他MPM-driven deformations such as elastoplasticity. As shown in Fig.XX, 在一些特别极端的物理参数下，Naive 3DGS在MPM driven下出现了失败，物体断裂并且出现了极其明显的针状伪影，而我们的方法保持了合理的物理运动。

\begin{wrapfigure}{r}{0.4\linewidth}
% \hspace{-2.0 em}
% \vspace{-2.5 em} % 需要时微调
\centering
\animategraphics[autoplay,loop,width=\linewidth]{12}{figures/supp/elastic_large_deform/}{000000}{000023}
% \vspace{-2.25 em}
\caption{
Generalization to Other MPM-Driven Deformations and Improved Robustness
}

% \vspace{-2.875 em}

\label{fig:supp:elastic_large_deform}
\end{wrapfigure}

Our proposed Topology-Adaptive Gaussian Rendering enhances the robustness of Gaussian splats
% , produces smoother geometry, and naturally generalizes to other MPM-driven deformations, such as elastoplasticity.
by stabilizing splat geometry under extreme deformation, producing smoother surfaces, and naturally generalizing to other MPM-driven deformations such as elastoplasticity.
As shown in Fig.~\ref{fig:supp:elastic_large_deform}, under extreme physical parameter settings, naïve 3DGS breaks down with object fracture and severe needle-like artifacts. In contrast, our method maintains physically plausible motion throughout the deformation process.
\textbf{Please view the dynamic video in Fig.~\ref{fig:supp:elastic_large_deform} in \textcolor{red}{Adobe Acrobat Reader}.}
