# Supplementary material for: MeGAS: Thermomechanical Dynamic Gaussian Splatting for Thermophysical Scene Editing
Source: arXiv:2606.23455 source file (2026-06-22)
Supplement: Supplementary file 5 [file 4_edit_details.tex]

% \pagebreak[0]
\vspace{-0.75 em}
\section{Details for Thermophysical Scene Editing}
\label{supp:exp_edit}
\vspace{-0.25 em}
We compare \method with three representative editing pipelines: DGE~\cite{chen2024dge}, a text-driven diffusion-based editing method for 3DGS; 
AutoVFX~\cite{hsu2025autovfx}, which leverages an LLM model~\cite{achiam2023gpt} to generate scripts for external physics engines to perform mesh-based melting and composite the results back into the scene;
Runway Gen-4.5~\cite{runway_gen4}, a leading commercial image-to-video generation model that augments a single input image with text-guided dynamic effects. 

\iffalse
For DGE, we use the prompt "Turn the (Truck/Sculpture/Lego Dozer) into a melted like" with guidance scale=15 and optimize the GS model with 15k iterations, DGE只能实现静态场景的风格编辑，无法实现动态效果，同时对于融化这种物理驱动的现象拟合效果有限;
For AutoVFX, we use the prompt "Melt the (Truck/Sculpture/Lego Dozer)", AutoVFX对场景使用Bakedsdf重建出Mesh，通过GPT自动分割前景并调取Blender的FLIP仿真算法实现融化效果，时间成本较大，且没有考虑融化效果与原始场景appearance上的一致性；
For Runway Gen-4, we输入各个视角的静态渲染图像作为image condition并use the prompt "The camera keep state, over time the (Truck/Sculpture/Lego Dozer) begins to melt", Runway Gen-4在视觉上实现了vivid dynamic effects, 但是结果并不满足物理合理性，且没有考虑物体自身的材质appearance，同时各个视角的编辑效果独立，无法保证时序上的多视角一致性。
\fi

\textbf{For DGE}, we use the prompt  
\emph{``Make the (Truck / Sculpture / Lego Dozer) look melted''}  
with a guidance scale of $15$, and optimize the 3DGS model for $15$k iterations. 
Since DGE utilizes an image-level diffusion as prior, it can only perform style editing of static scenes and does not produce explicit dynamic motion. 
Moreover, its ability to faithfully capture melting, which is inherently a physics-driven phenomenon, is limited and often results in only superficial, texture-level changes.
\textbf{For AutoVFX}, we use the prompt  
\emph{``Melt the (Truck / Sculpture / Lego Dozer)''}.  
AutoVFX first reconstructs a mesh representation of the scene, then uses GPT-based scripting to automatically segment the foreground object and invoke Blender’s FLIP fluid simulation to realize a melting effect. 
While this pipeline can generate physically plausible deformations on the mesh, it incurs substantial computational overhead and does not explicitly enforce appearance consistency between the simulated melting result and the original scene, leading to noticeable appearance discrepancies in the final composites.
\textbf{For Runway Gen-4.5}, we input per-view static renderings of the reconstructed scene as image conditions and use the prompt  
\emph{``The camera keeps still, and over time the (Truck / Sculpture / Lego Dozer) begins to melt''}.  
Runway Gen-4.5 produces visually vivid dynamic effects, however, the generated motion is not constrained by physical laws and often violates basic physical plausibility. 
In addition, the model does not preserve the original material appearance of the object consistently, and each viewpoint is edited independently, which leads to temporal and multi-view inconsistencies across the different camera trajectories.

\noindent\textbf{User Study.}
We recruited 27 participants, and each participant was asked to evaluate 24 videos generated by different methods and from different viewpoints, and to rank the results according to their personal preference.
We present the user evaluation interface with one representative example as shown in Fig.~\ref{fig:supp:user_study}.

% 额外的视频生成模型对比
\begin{figure}[t] \centering
    % \vspace{-1.375 em}
    \includegraphics[width=0.95\linewidth]{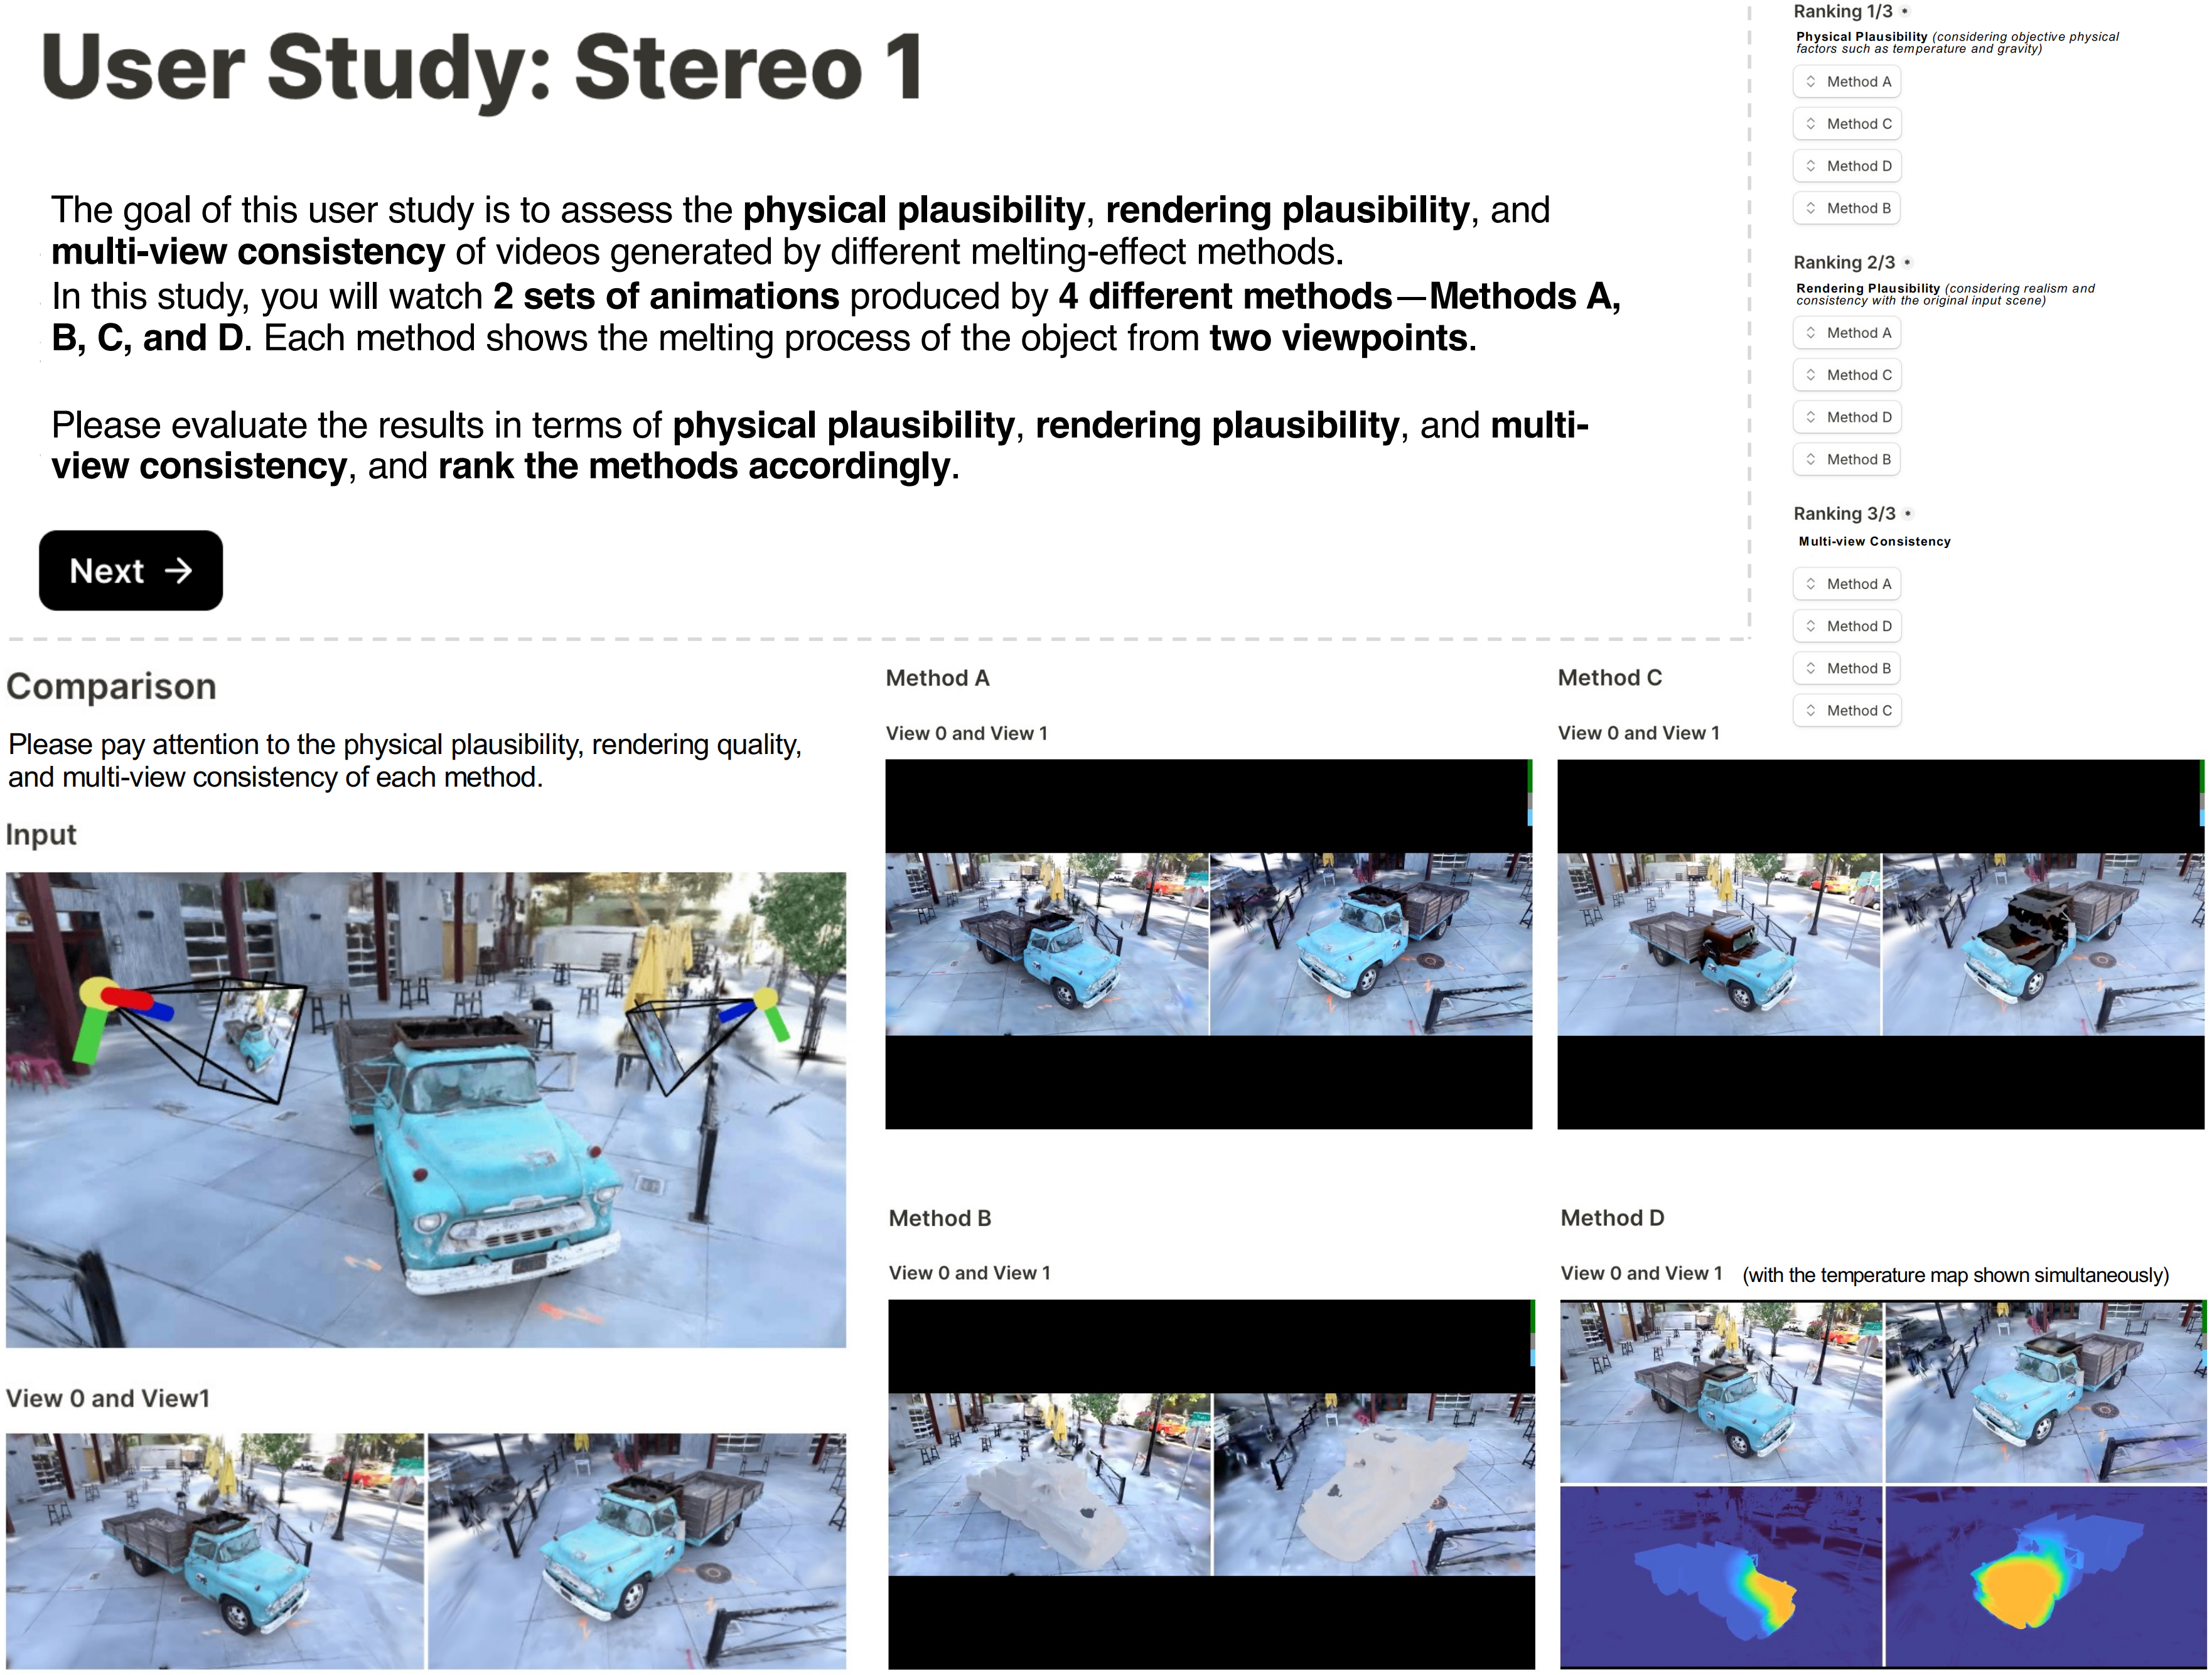}
    % \animategraphics[autoplay,loop,width=\linewidth]{15}{figures/supp/extra_video_gen/}{000000}{000023}
    % \vspace{-0.625 em}
    \caption{
    \textbf{The user evaluation interface.}
    We rearranged the layout of the interface to present it more clearly in the paper.
    }
    \label{fig:supp:user_study}
    \vspace{0.5 em}
\end{figure}

\begin{figure}[t] \centering
    % \vspace{-1.25 em}
    % \includegraphics[width=0.475 \textwidth]{figure/rebuttal/2_complex_scene.pdf}
    \animategraphics[autoplay,loop,width=\linewidth]{15}{figures/supp/extra_video_gen/}{000000}{000023}
    % \vspace{-2.0 em}
    \caption{
    \textbf{Comparison with extra video generation models.} Please view the dynamic videos in \textcolor{red}{Adobe Acrobat Reader}.
    }
    \label{fig:supp:extra_video_gen}
    % \vspace{-1.5 em}
\end{figure}

\noindent\textbf{Additional SOTA Video Generation Comparisons.}
We further compare our method against additional state-of-the-art video generation models, including Veo 3~\cite{veo3_google2025}, Wan 2.6~\cite{wan26_wan2026} and Kling 2.6~\cite{kling26_kuaishou2025}, to show that, for highly physics-grounded animations, although all of them produce vivid visual effects, even recent state-of-the-art video generation models still struggle with controllability, physical plausibility, and multi-view consistency (\textbf{please view the dynamic videos in Fig.~\ref{fig:supp:extra_video_gen} in \textcolor{red}{Adobe Acrobat Reader}}). 
For specific physical phenomena such as melting, coupling with explicit physics simulators remains essential.
This is also supported by prior works, where explicit simulation has been widely adopted as an effective paradigm for modeling specialized physical phenomena, such as in RainyGS~\cite{dai2025rainygs}, FieryGS~\cite{shen2026fierygs}, GaussianSplashing~\cite{feng2025gaussian}, and EnliveningGS~\cite{shen2025enliveninggs}, enabling data-free, controllable, and physically plausible animations.
% 我们比较了更多sota的video generation模型 Veo3/Wan2.6/Kling2.6 来说明for highly physical-grounded animations, 尽管all produce vivid effects but even SOTA models still struggle with controllability, physical plausibility and multi-view consistency. For specific physical phenomena like melting, coupling explicit physics simulators remains necessary.
