# Supplementary material for: MeGAS: Thermomechanical Dynamic Gaussian Splatting for Thermophysical Scene Editing
Source: arXiv:2606.23455 source file (2026-06-22)
Supplement: Supplementary file 6 [file 5_more_results.tex]

\vspace{-0.5 em}
\section{Quantitative Evaluation against Simulation Platform}
\vspace{-0.25 em}
\label{supp:houdini_simulation}
We add a quantitative evaluation against independent mesh-based thermomechanical simulation references generated by Houdini~\cite{houdini}, a professional physical simulation platform, 
under the same heat-source and thermal-boundary setup as our method, these simulations provide an independent physics-based reference.
The temporally averaged surface accuracy shows \method aligns well with the reference while preserving photorealism. 

\begin{figure}[h] \centering
    \vspace{-2.0 em}
    \includegraphics[width=0.975 \textwidth]{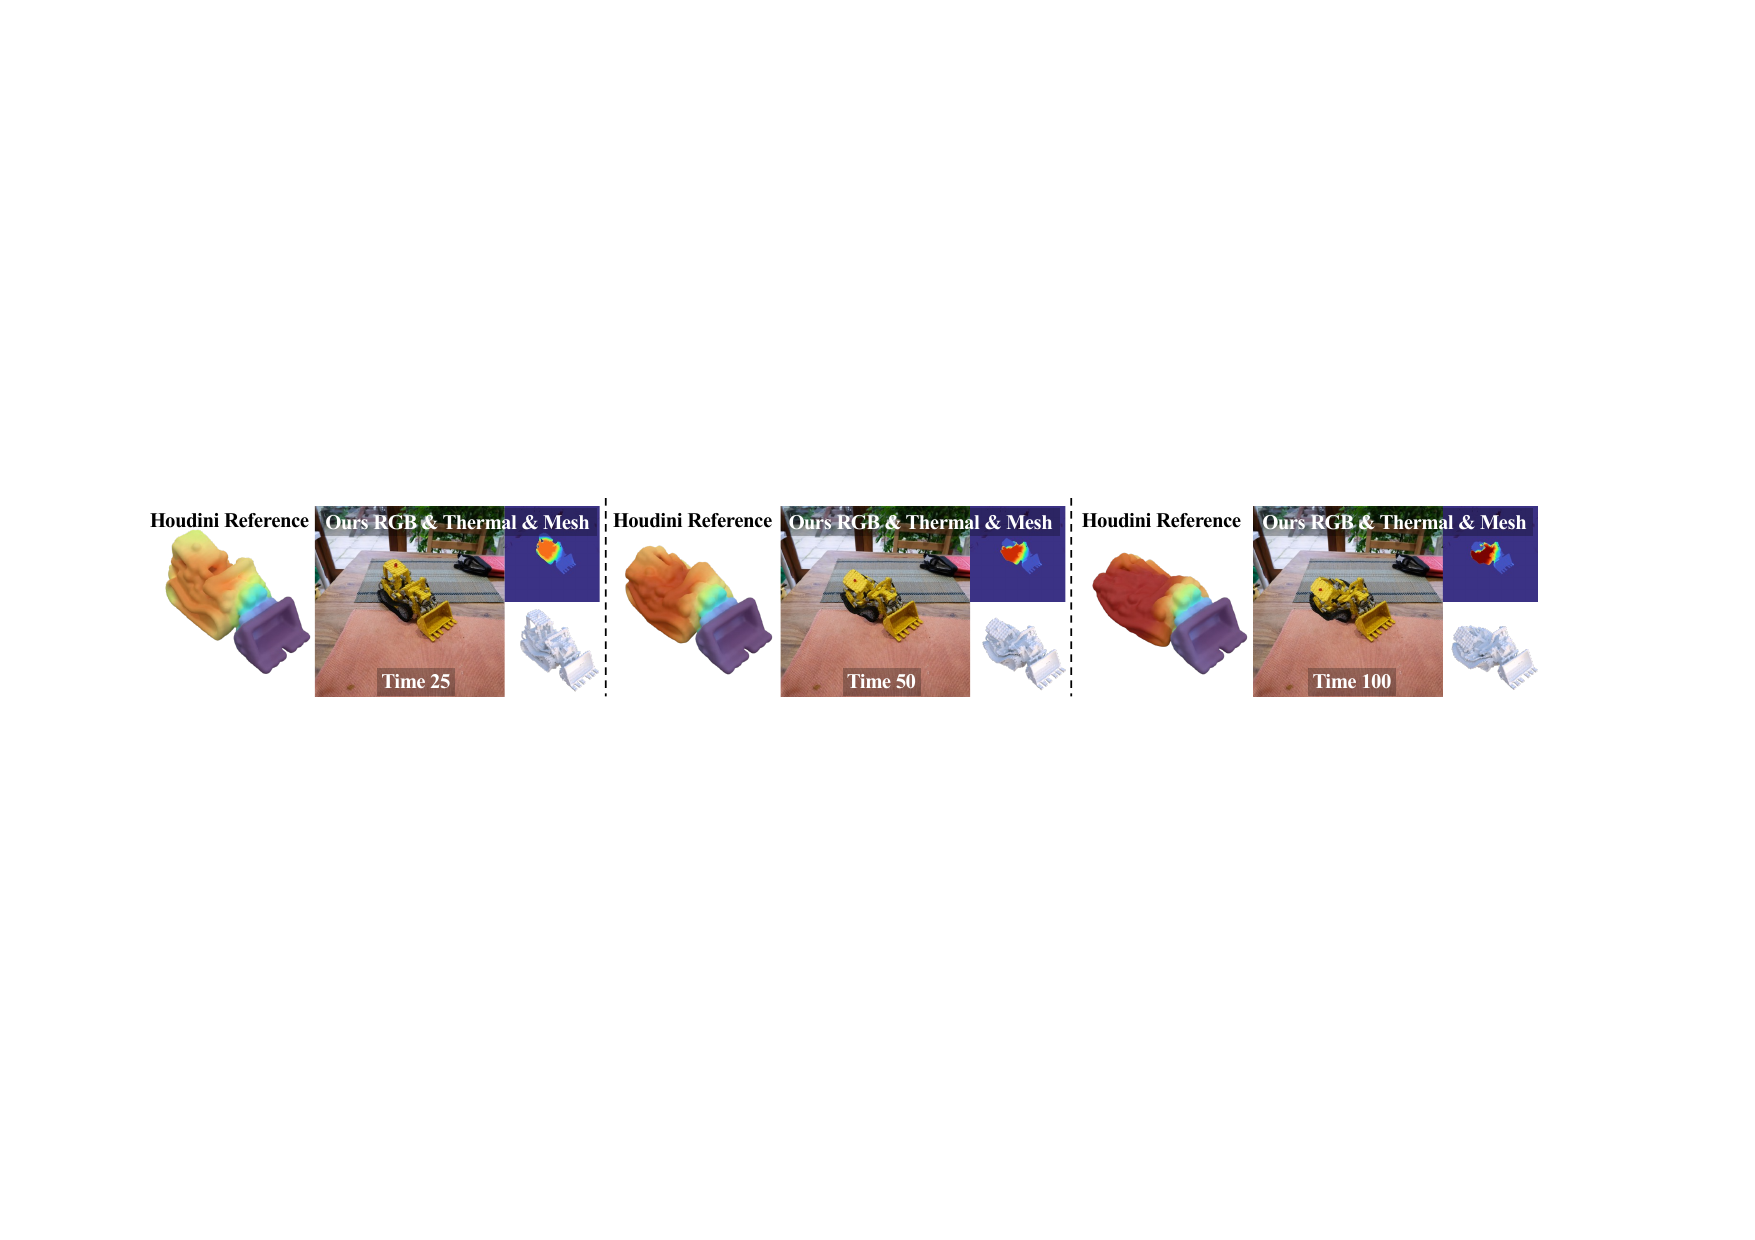}
    \vspace{-4.0 em}
\end{figure}

\begin{table}[h]
\centering
\large
\setlength{\tabcolsep}{4pt}

% \vspace{-1.0 em}
\resizebox{0.9\textwidth}{!}{
    \begin{tabular}{lcccc}
    \specialrule{.1em}{.1em}{.1em}
    Method       
    & Chamfer Distance $\downarrow $
    & F-score $\uparrow $
    & $\mathrm{Depth}_{\mathrm{RMSE}}$ $\downarrow$ 
    & Silhouette IoU $\uparrow$ \\
    \midrule
    PhysGaussian & 0.089 & 0.08 & 0.130 & 0.435 \\
    Ours         & \textbf{0.037} & \textbf{0.23} & \textbf{0.065} & \textbf{0.789} \\
    \specialrule{.1em}{.1em}{.1em}
    % \vspace{-3.375 em}
    \end{tabular}
}
\end{table}

\vspace{-2.5 em}
\section{Handling Different Materials}
\vspace{-0.25 em}
\label{supp:seg_material}
% \begin{figure}[t] \centering
\begin{wrapfigure}[6]{r}{0.7\linewidth}
    \vspace{-2.0 em}
    \includegraphics[width=\linewidth]{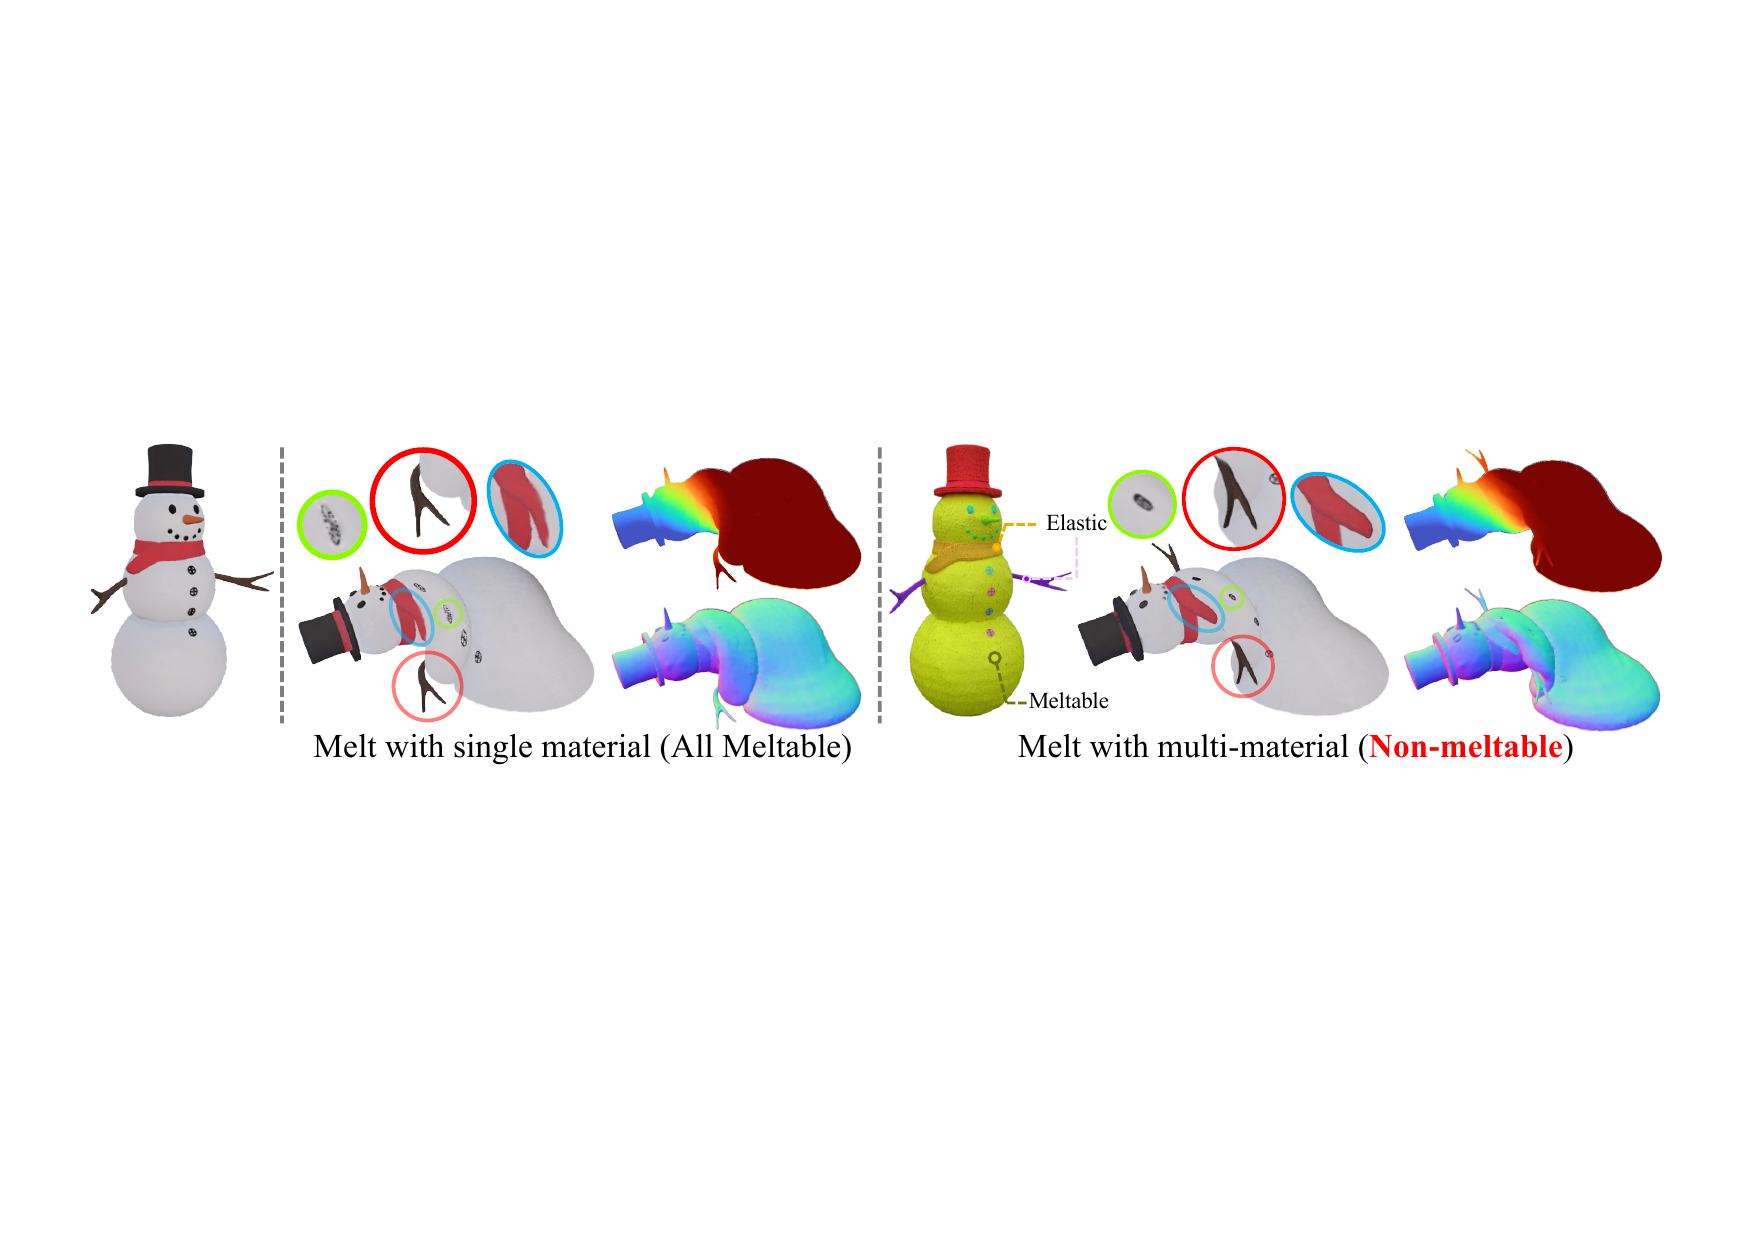}
    % \vspace{-2.0 em}
    \caption{
    Multi-material melting.
    }
    \label{fig:supp:multi_material_melt}
    \vspace{-1.5 em}
\end{wrapfigure}

We further consider multi-material thermophysical editing by performing part-level segmentation and assigning material-specific constitutive models to different object parts.
As shown in Fig.~\ref{fig:supp:multi_material_melt}, object components such as buttons and branches are specified as non-meltable materials (e.g., elastic),
while the snow regions remain thermally deformable, producing distinct deformation behaviors across materials and demonstrating that MeGAS can be naturally extended to handle heterogeneous material compositions.
% We further consider multi-material melting by performing part-level segmentation and assigning material-specific constitutive models to different object parts. This enables distinct deformation behaviors across materials and demonstrates that MeGAS can be naturally extended to handle heterogeneous material compositions.

\section{Additional Multi-view Results}
\vspace{-0.25 em}
\label{supp:multiview_render}
We provide additional multi-view rendering results for Section~\textcolor{red}{5.2} to further demonstrate cross-view consistency under large deformations as shown in Fig.~\ref{fig:supp:mv_render}. 
\textbf{Please view the dynamic videos in \textcolor{red}{Adobe Acrobat Reader}.}

\begin{figure}[h] \centering
    \vspace{-1.5 em}
    \animategraphics[autoplay,loop,width=\linewidth]{15}{figures/supp/mv_render/}{000000}{000029}
    \vspace{-1.5 em}
    \caption{
    Additional multi-view rendering results.
    }
    \label{fig:supp:mv_render}
    % \vspace{-2.5 em}
\end{figure}

\section{Additional Results on Real-World Scenes}
\label{supp:more_real_data}
As shown in Fig.~\ref{fig:supp:more_results}, we visualize the thermomechanical dynamics of our method under heat-diffusion control. As the temperature field propagates through the object, phase-change-aware control triggers constitutive model switching, yielding realistic melting-style scene editing. 
We illustrate the deformation process on real-world scenes, with rendered RGB images, rendered temperature field, and deformation geometries (rendered normals and meshes) at different viewpoints and time steps. 
% Our method achieves high physical plausibility as well as strong temporal and multi-view consistency.
Our method produces physically plausible thermomechanical dynamics while maintaining strong temporal and multi-view consistency.

\begin{figure*}[t] % 使用 !t 尝试强制图像置顶
    \centering
    \scriptsize
    \vspace{-3.0 em}
    \includegraphics[width=\textwidth]{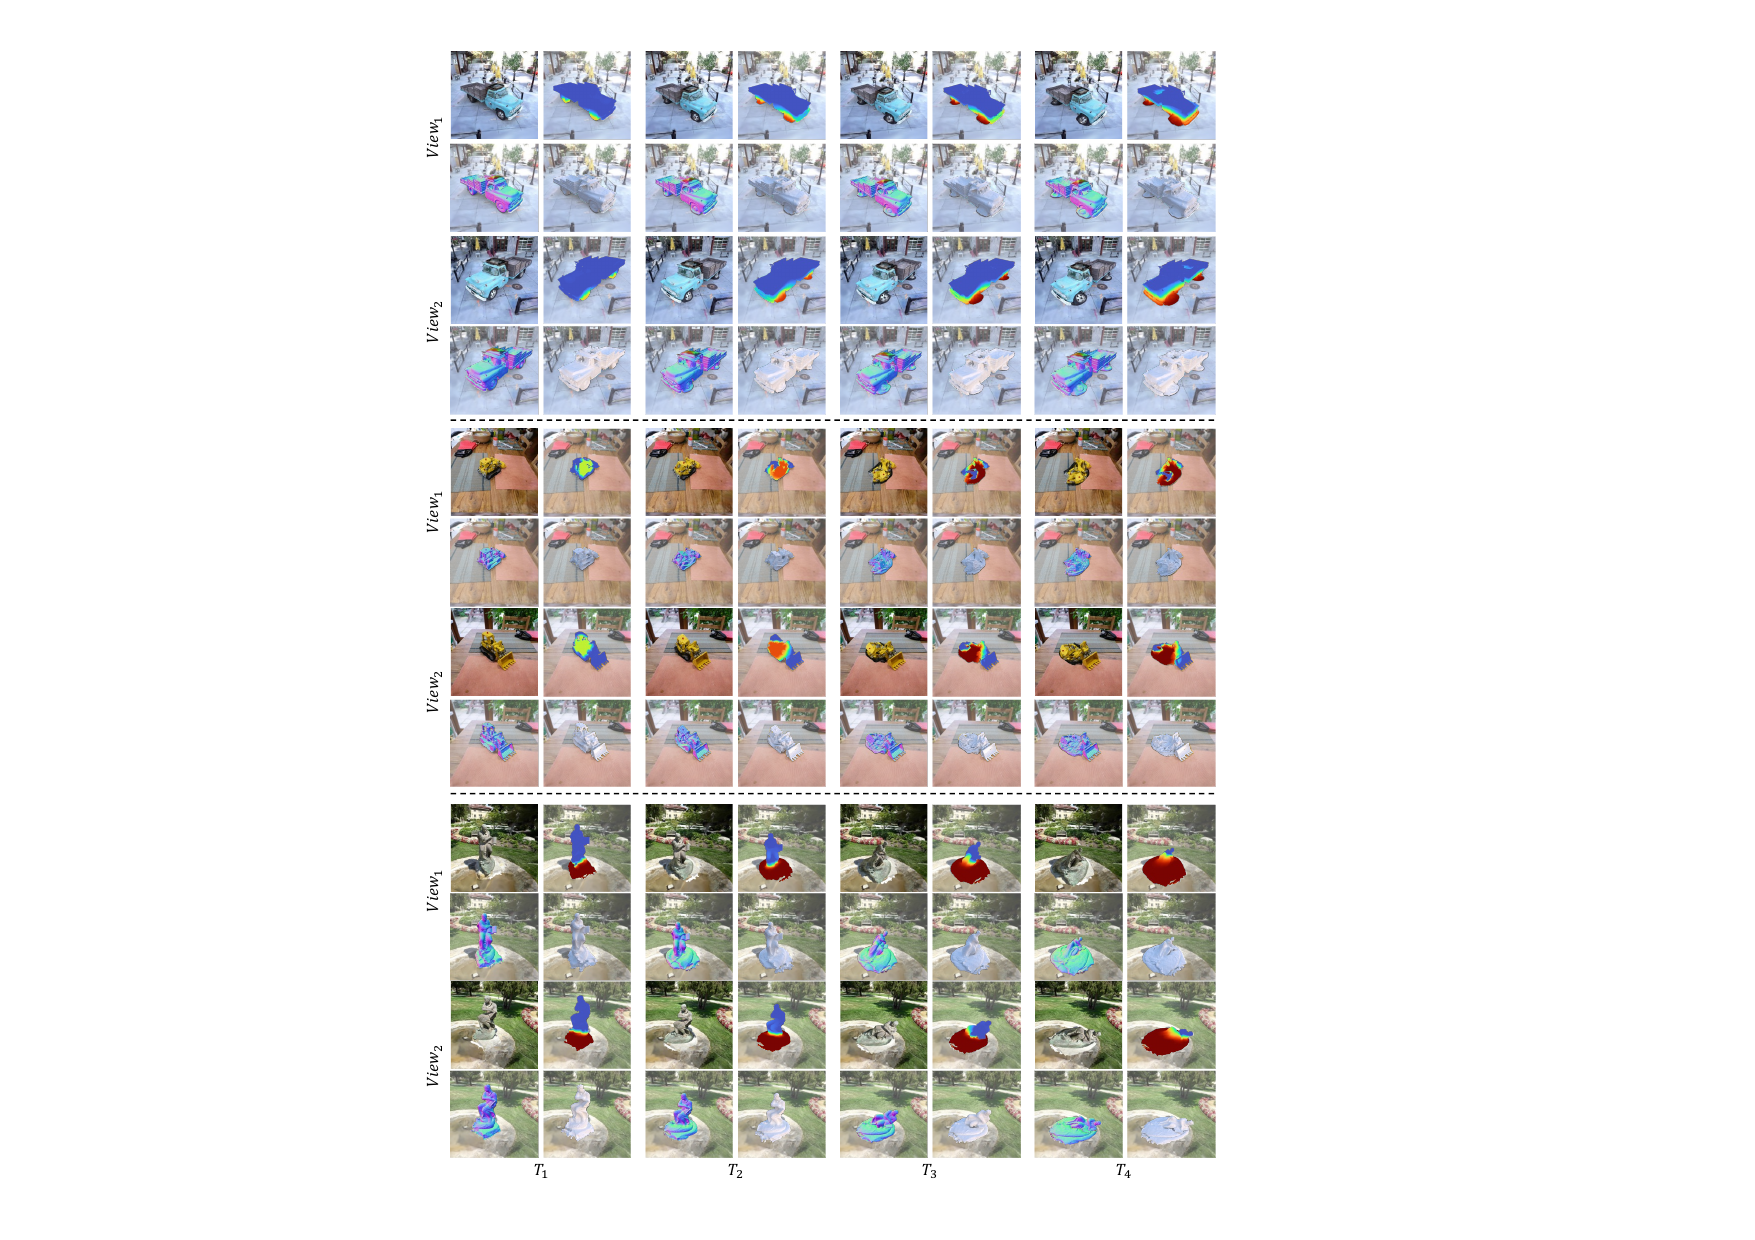}
    % \vspace{-2.5 em}
    \caption{
    \textbf{Our thermophysical scene editing.}
    We illustrate the deformation process on real-world scenes, with rendered RGB images, rendered temperature field, and deformation geometries (rendered normals and meshes) at different viewpoints and time steps.
    }
    \vspace{-0.75 em}
    \label{fig:supp:more_results}
\end{figure*}

\clearpage

% 物体级别的多视图

% Elastoplasticity

% Computational cost
