# Supplementary material for: MeGAS: Thermomechanical Dynamic Gaussian Splatting for Thermophysical Scene Editing
Source: arXiv:2606.23455 source file (2026-06-22)
Supplement: Supplementary file 7 [file mpm_params.tex]

% \begin{table}[h]
\begin{wraptable}{l}{0.55 \textwidth}
  \centering
  \vspace{-2.5 em}
  \caption{
  \textbf{Material and discretization parameters.}
  We use identical physical parameters across all experiments.
  }
  \vspace{1.0 em}
  \resizebox{\linewidth}{!}{
  \begin{tabular}{lcl}
    \hline
    Parameter & Value & Description \\
    \hline
    $E$ & $2.8\times10^{4}$ & Young's modulus \\
    $\nu$ & $0.4$ & Poisson's ratio \\
    $g$ & $1.0$ & Gravity acceleration \\
    $\rho$ & $100.0$ & Density of the solid \\
    $\eta$ & $100.0$ & Viscosity coefficient \\
    $h_{\text{shear}}$ & $1.0$ & Shear ratio for plastic flow \\
    $\sigma_{Y}$ & $1.0$ & Yield threshold \\
    $T_{\text{melt}}$ & $0.7$ & Thermal phase threshold \\
    \hline
    $\Delta t$ & $1.0\times 10^{-4}$ & Time step size \\
    $N_{\text{sub}}$ & $100$ & MPM sub-steps per frame \\
    $N_{\text{grid}}$ & $100^3$ & Grid resolution \\
    \hline
  \end{tabular}
  }
  
  \label{tab:mpm_params}
  \vspace{-2.0 em}
% \end{table}

\end{wraptable}
