# Supplementary material for: MeGAS: Thermomechanical Dynamic Gaussian Splatting for Thermophysical Scene Editing
Source: arXiv:2606.23455 source file (2026-06-22)
Supplement: Supplementary file 8 [file psnr_ablation.tex]

\begin{wraptable}{r}{0.475 \textwidth}
\vspace{-0.25 em}
\caption{
\textbf{Ablation of rendering quality.} 
We progressively add each module on top of the backbone. Our module substantially reduces internal floaters and yields a more uniform Gaussian distribution, while maintaining comparable PSNR.
Although the anisotropy regularization slightly degrades PSNR, the subsequent scale clamping recovers the rendering quality.
}
\vspace{1.0 em}
% \begin{table}[t]
\resizebox{\linewidth}{!}{
\begin{tabular}{lccc}
\specialrule{.1em}{.1em}{.1em}
Module (Progressively Add)    & PSNR$\uparrow$ & SSIM$\uparrow$ & LPIPS$\downarrow$ \\
\midrule
Backbone~\cite{chen2024pgsr}  & 37.33          & 0.9813          & 0.031             \\
\midrule
w/ Internal Pruning           & 36.76          & 0.9801          & 0.035             \\
w/ Anisotropy Reg.            & 35.81          & 0.9767          & 0.045             \\
w/ Scale Clamping             & 37.24          & 0.9805          & 0.031             \\
\specialrule{.1em}{.1em}{.1em}
\end{tabular}
}
\vspace{-2.0 em}

\label{supp:tab:psnr}
% \end{table}
\end{wraptable}
